# Supplementary material for: Cognacy Queries over Dependence Graphs for Transparent Visualisations
Source: arXiv:2403.04403 source file (2024-10-15)
Supplement: Supplementary file 1 [file core-ann-expr.tex]

\section{Core language: Alternative graph semantics}
\begin{figure}[H]
  {\small \flushleft \shadebox{$\gamma, e, V \evalS v, G$}%
  \begin{smathpar}
     \inferrule*[
     lab={\ruleName{$\evalS$-var}}
     ]
     {
        \strut
     }
     {
        \gamma \cons (\bind{x}{v}), \exVar{x}, V
        \evalS
        v,
        \emptyset
     }
     \and
     \inferrule*[
        lab={\ruleName{$\evalS$-int}}
     ]
     {
        \strut
     }
     {
        \gamma, \annInt{n}{\alpha}, V
        \evalS
        \annInt{n}{\alpha'},
        \set{\bind{\alpha'}{(V \disjunion \set{\alpha})}}
     }
     \and
     \inferrule*[lab={\ruleName{$\evalS$-function}}]
     {
        \strut
     }
     {
        \gamma, \exFun{\sigma}, V
        \evalS
        \annClosure{\gamma}{\envEmpty}{\sigma}{\alpha},
        \set{\bind{\alpha}{V}}
     }
     \and
     \inferrule*[lab={\ruleName{$\evalS$-record}}]
     {
        \gamma, \seq{e}, V \evalS \seq{v}, G
     }
     {
        \gamma, \annRec{\seq{\bind{x}{e}}}{\alpha}, V
        \evalS
        \annRec{\seq{\bind{x}{v}}}{\alpha'},
        G \disjunion \set{\bind{\alpha'}{(V \disjunion \set{\alpha})}}
     }
     \and
     \inferrule*[lab={\ruleName{$\evalS$-constr}}
     , right={$\Sigma(c) = |\seq{e}|$}]
     {
        \gamma, \seq{e}, V \evalS \seq{v}, G
     }
     {
        \gamma, \annConstr{c}{\seq{e}}{\alpha}, V
        \evalS
        \annConstr{c}{\seq{v}}{\alpha'},
        G \disjunion \set{\bind{\alpha'}{(V \disjunion \set{\alpha})}},
     }
     \and
     \inferrule*[
        lab={\ruleName{$\evalS$-record-project}}
     ]
     {
        \gamma, e, V \evalS \annRec{\seq{\bind{x}{v}} \cons (\bind{y}{u})}{\alpha}, G
     }
     {
        \gamma, \exRecProj{e}{y}, V
        \evalS
        u,
        G
     }
     \and
     \inferrule*[ lab={\ruleName{$\evalS$-foreign-app}}
     , right={$\Phi(f) = |\seq{e}|$}]
     {
        \gamma, \seq{e}, V \evalS \seq{v}, G
        \\
        \interpret{f}(\seq{v}) = (u, G')
     }
     {
        \gamma, \exForeignApp{f}{\seq{e}}, V
        \evalS
        u,
        G \disjunion G'
     }
     \and
     \inferrule*[
        lab={\ruleName{$\evalS$-app}},
        width=4in,
     ]
     {
        \gamma, e, V \evalS \annClosure{\gamma_1}{\rho}{\sigma}{\alpha}, G_1
        \\
        \gamma_1, \rho, \set{\alpha} \closeDefs \gamma_2, G_2
        \\
        \gamma, e', V \evalS v', G_3
        \hspace{0.5cm}
        v', \sigma \match \gamma_3, e^\twoPrime, V'
        \hspace{0.5cm}
        \gamma_1 \concat \gamma_2 \concat \gamma_3, e^\twoPrime, V' \disjunion \set{\alpha} \evalS u, G_4
     }
     {
        \gamma, \exApp{e}{e'}, V
        \evalS
        u,
        \textstyle{\bigdisjunion}\set{\seqRange{G_1}{G_4}}
     }
     \and
     \inferrule*[
        lab={\ruleName{$\evalS$-let}}
     ]
     {
        \gamma, e, V \evalS v, G
        \\
        \gamma \cons (\bind{x}{v}), e', V \evalS v', G'
     }
     {
        \gamma, \exLet{x}{e}{e'}, V
        \evalS
        v',
        G \disjunion G'
     }
     \and
     \inferrule*[
        lab={\ruleName{$\evalS$-let-rec}}
     ]
     {
        \gamma, \set{\seq{\bind{x}{\sigma}}}, V \closeDefs  \gamma', G
        \\
        \gamma \concat \gamma', e, V \evalS v, G'
     }
     {
        \gamma, \exLetRec{\seq{\bind{x}{\sigma}}}{e}, V
        \evalS
        v,
        G \disjunion G'
     }
  \end{smathpar}}
  \caption{Operational semantics: evaluation and graph construction for (selectively) annotated expressions $e_\alpha$}
  \label{fig:core:eval-ann-expr}
\end{figure}
