# Supplementary material for: Cognacy Queries over Dependence Graphs for Transparent Visualisations
Source: arXiv:2403.04403 source file (2024-10-15)
Supplement: Supplementary file 2 [file desugaring-proofs.tex]

\section{Desugaring: proofs}

\subsection{\lemref{closedefs-eq}}
\label{app:proofs:close-defs-eq}
\setcounter{equation}{0}
\proofContext{closedefs-eq}
\begin{proof}
   \small
   \begin{flalign}
      &
      \gamma_1 \desugar \gamma_2
      &
      \text{suppose}
      \notag
      \\
      &
      \seq{\mu} \desugar \seq{\sigma}
      &
      \text{suppose}
      \notag
      \\
      &
      \derivation{\derivationWidth}{
         \begin{smathpar}
            \inferrule*[
%               left={\ruleName{$\closeDefs$-surface}}
            ]
            {
               g = \seq{\bind{x}{\mu}}
               \\
               v_i = \exClosure{\gamma_1}{g}{\mu_i}
               \quad
               (\forall i \le \length{\seq{x}})
            }
            {
               \gamma_1, g \closeDefs \set{\seq{\bind{x}{v}}}
            }
         \end{smathpar}
      }
      &
      \text{suppose}
      \notag
      \\
      &
      \derivation{\derivationWidth}{
         \begin{smathpar}
            \inferrule*[
%               left={\ruleName{$\closeDefs$-core}}
            ]
            {
               \rho = \set{\seq{\bind{x}{\sigma}}}
               \\
               v'_i = \exClosure{\gamma_2}{\rho}{\sigma_i}
               \quad
               (\forall i \numleq \length{\seq{x}})
            }
            {
               \gamma_2, \rho
               \closeDefs
               \set{\seq{\bind{x}{v}}'}
            }
         \end{smathpar}
      }
      &
      \text{suppose}
      \notag
      \\
      &
      \qedLocal
      \derivation{\derivationWidth}{
         \begin{smathpar}
            \inferrule*
            [
               left={\ruleName{$\desugar$-env}}
            ]
            {
               \inferrule*
               [
                  left={\ruleName{$\desugar$-closure}},
                  right={$\forall i. \numleq \length{\seq{x}}$}
               ]
               {
                  \gamma_1 \desugar \gamma_2
                  \\
                  \seq{\mu} \desugar \seq{\sigma}
                  \\
                  \mu_i \desugar \sigma_i
               }
               {
                  v_i = \exClosure{\gamma_1}{g}{\mu_i} \desugar \exClosure{\gamma_2}{\rho}{\sigma_i}
               }
            }
            {
               \set{\seq{\bind{\exVar{x}}{v}}} \desugar \set{\seq{\bind{\exVar{x}}{v}}'}
            }
         \end{smathpar}
      }
      &
      \notag
   \end{flalign}
\end{proof}

\subsection{\lemref{match-seq-eq}}
\label{app:proofs:match-seq-eq}
\setcounter{equation}{0}
\proofContext{match-seq-eq}
We prove part (2) simultaneously with the $\implies$ direction of part (1) by induction on surface-language
$\match$ derivation. We omit the proof of the $\impliedby$ direction of part (1), which is similar.

\begin{proof}
\small
\begin{flalign}
   &
   \seq{u} \desugar \seq{v}
   &
   \text{suppose}
   \locallabel{us-desugar-vs}
   \\
   &
   \seq{k} \desugar \kappa
   &
   \text{suppose}
   \notag
   \\
   &
   \seq{u}, \seq{k} \match \gamma, s
   &
   \text{suppose}
   \notag
   \\
   \intertext{\crossrule}
   %%%%%%%%%%%%%%%%%%%%%%%%%%%
   &
   \caseDerivation{\derivationWidth}{
      \begin{smathpar}
         \inferrule*[
            lab={\ruleName{$\match$-done-uncurried}}
          ]
          {
             \strut
          }
          {
             \Lowlight{\seq{u} =\;}\seqEmpty,
             \Lowlight{\seq{k} =\;}(\seqEmpty, \clause{\seqEmpty}{s})
             \match \envEmpty\Lowlight{\;= \gamma}, s
          }
      \end{smathpar}
   }
   &
   \notag
   \\
   &
   \derivation{\derivationWidth}{
      \begin{smathpar}
         \inferrule*[
            lab={\ruleName{$\desugar$-clauses-done}}
         ]
         {
            s \desugar e
         }
         {
            \Lowlight{\seq{k} =\;}(\seqEmpty, \clause{\seqEmpty}{s}) \desugar e\Lowlight{\;=\kappa}
         }
      \end{smathpar}
   }
   &
   \text{inversion}
   \locallabel{done-uncurried-inversion}
   \\
   &
   \seq{v} = \seqEmpty
   &
   \text{(\localref{us-desugar-vs})}
   \notag
   \\
   &
   \qedLocal
   \derivation{\derivationWidth}{
      \begin{smathpar}
         \inferrule*[
            lab={\ruleName{$\match$-done}}
         ]
         {
            \strut
         }
         {
            \Lowlight{\seq{v} =\;}\seqEmpty,
            \Lowlight{\kappa =\;}e \match \envEmpty, e
         }
      \end{smathpar}
   }
   &
   \notag
   \\
   &
   \qedLocal
   \envEmpty \desugar \envEmpty\text{ and }s \desugar e
   &
   \text{(\localref{done-uncurried-inversion})}
   \notag
   \\
   \intertext{\crossrule}
   %%%%%%%%%%%%%%%%%%%%%%%%%%%
   &
   \caseDerivation{\derivationWidth}{
      \begin{smathpar}
         \inferrule*[
            left={\ruleName{$\match$-done-curried}}
          ]
          {
             \strut
          }
          {
             \Lowlight{\seq{u} =\;}
             \seqEmpty, (\seqRange{(\seqEmpty, \clause{p_1 \cons \pi_1}{s_1})}
                                  {(\seqEmpty, \clause{p_j \cons \pi_j}{s_j})}) \\
             \match
             \envEmpty\Lowlight{\;=\gamma}, \exFun{(\seq{\clause{p \cons \pi}{s}})}\Lowlight{\;=s}
          }
       \end{smathpar}
   }
   &
   \notag
   \\
   &
   \derivation{\derivationWidth}{
      \begin{smathpar}
         \inferrule*[
            left={\ruleName{$\desugar$-clauses-curried}}
         ]
         {
            \seq{(p, \clause{\pi}{s})}
            \desugar
            \sigma
         }
         {
            \seqRange{(\seqEmpty, \clause{p_1 \cons \pi_1}{s_1})}
                     {(\seqEmpty, \clause{p_j \cons \pi_j}{s_j})}
            \desugar
            \exFun{\sigma}\Lowlight{\;=\kappa}
         }
       \end{smathpar}
   }
   &
   \text{inversion}
   \locallabel{done-curried-inversion}
   \\
   &
   \seq{v} = \seqEmpty
   &
   \text{(\localref{us-desugar-vs})}
   \notag
   \\
   &
   \qedLocal
   \derivation{\derivationWidth}{
      \begin{smathpar}
         \inferrule*[
            left={\ruleName{$\match$-done}}
         ]
         {
            \strut
         }
         {
            \Lowlight{\seq{v} =\;}
            \seqEmpty, \exFun{\sigma} \match \envEmpty, \exFun{\sigma}
         }
      \end{smathpar}
   }
   &
   \notag
   \\
   &
   \qedLocal
   \envEmpty \desugar \envEmpty
   &
   \notag
   \\
   &
   \qedLocal
   \derivation{\derivationWidth}{
      \begin{smathpar}
         \inferrule*[left={\ruleName{$\desugar$-lambda}}]
         {
            \inferrule*[
               left={\ruleName{$\desugar$-fun}}
            ]
            {
               \seq{(p, \clause{\pi}{s})}
               \desugar \sigma
            }
            {
               \seq{\clause{p \cons \pi}{s}}
               \desugar
               \sigma
            }
         }
         {
            \exFun{(\seq{\clause{p \cons \pi}{s}})} \desugar \exFun{\sigma}
         }
      \end{smathpar}
   }
   &
   \text{(\localref{done-curried-inversion})}
   \notag
   \\
   \intertext{\crossrule}
   %%%%%%%%%%%%%%%%%%%%%%%%%%%
   &
   \caseDerivation{\derivationWidth}{
      \begin{smathpar}
         \inferrule*[
            left={\ruleName{$\match$-var}}
          ]
          {
             \seq{u}', \seq{k}
             \match \gamma^\dagger, s
          }
          {
             \Lowlight{\seq{u} =\;}
             u \cons \seq{u}',
             \seqRange{(\pattVar{x} \clauseWith{\cons} k_1)}{(\pattVar{x} \clauseWith{\cons} k_j)}
             \match
             \set{\bind{x}{v}} \disjunion \gamma^\dagger\Lowlight{\;= \gamma}, s
          }
       \end{smathpar}
   }
   &
   \notag
   \\
   &
   \derivation{\derivationWidth}{
      \begin{smathpar}
         \inferrule*[
            left={\ruleName{$\desugar$-clauses-var}}
         ]
         {
            \seq{k} \desugar \kappa'
         }
         {
            \seqRange{(\pattVar{x} \clauseWith{\cons} k_1)}{(\pattVar{x} \clauseWith{\cons} k_j)}
            \desugar
            (\elimVar{x}{\kappa'})\Lowlight{\,= \kappa}
         }
      \end{smathpar}
   }
   &
   \text{inversion}
   \notag
   \\
   &
   \seq{v} = v \cons \seq{v}'\text{ with }u \desugar v\text{ and }\seq{u}' \desugar \seq{v}'
   \quad
   (\exists v, \seq{v}')
   &
   \text{(\localref{us-desugar-vs})}
   \notag
   \\
   &
   \seq{v}', \kappa' \match \gamma^\ddagger, e
   \textit{ with }\gamma^\dagger \desugar \gamma^\ddagger
   \textit{ and }s \desugar e
   \quad
   (\exists\gamma^\ddagger, e)
   &
   \text{IH}
   \notag
   \\
   &
   \qedLocal
   \derivation{\derivationWidth}{
      \begin{smathpar}
         \inferrule*[left={\ruleName{$\match$-var}}]
         {
            \seq{v}', \kappa' \match \gamma^\ddagger, e
         }
         {
            v \cons \seq{v}, \elimVar{x}{\kappa'} \match \set{\bind{x}{v}} \disjunion \gamma^\ddagger, e
         }
      \end{smathpar}
   }
   &
   \notag
   \\
   &
   \qedLocal
   \set{\bind{x}{u}} \disjunion \gamma^\dagger
   \desugar
   \set{\bind{x}{v}} \disjunion \gamma^\ddagger
   \textit{ and }
   s \desugar e
   &
   \text{($u \desugar v$)}
   \notag
   \\
   \intertext{\crossrule}
   %%%%%%%%%%%%%%%%%%%%%%%%%%%
   &
   \caseDerivation{\derivationWidth}{
      \begin{smathpar}
         \inferrule*[
            left={\ruleName{$\match$-record}}
         ]
         {
            \exRecord{\seq{\bind{y}{u}}^\ddagger} \subseteq \exRecord{\seq{\bind{x}{u}}^\dagger}
            \\
            \seq{u}^\ddagger \concat \seq{u}',
            (\seqRange{\seq{p_1}}{\seq{p_j}}) \clauseWith{\concat} \seq{k}
            \match \gamma, s
         }
         {
            \Lowlight{\seq{u} =\;}
            \exRecord{\seq{\bind{x}{u}}^\dagger} \cons \seq{u}',
            (\seqRange{\pattRecord{\seq{\bind{y}{p_1}}}}
                      {\pattRecord{\seq{\bind{y}{p_j}}}}) \clauseWith{\cons} \seq{k}
            \match
            \gamma, s
         }
      \end{smathpar}
   }
   &
   \notag
   \\
   &
   \derivation{\derivationWidth}{
      \begin{smathpar}
         \inferrule*[
            left={\ruleName{$\desugar$-clauses-record}}
         ]
         {
            (\seqRange{\seq{p_1}}{\seq{p_j}}) \clauseWith{\concat} \seq{k} \desugar \kappa'
         }
         {
            (\seqRange{\pattRecord{\seq{\bind{x}{p_1}}}}{\pattRecord{\seq{\bind{x}{p_j}}}})
            \clauseWith{\cons} \seq{k}
            \desugar
            (\elimRecord{\seq{x}}{\kappa'})
            \Lowlight{\;= \kappa}
         }
      \end{smathpar}
   }
   &
   \text{inversion}
   \notag
   \\
   &
   \seq{v} = \exRec{\seq{\bind{x}{v}}^\dagger} \cons \seq{v}'
   \textit{ with }
   \seq{u}^\dagger \desugar \seq{v}^\dagger
   \textit{ and }
   \seq{u}' \desugar \seq{v}'
   \quad
   (\exists \seq{v}^\dagger, \seq{v}')
   &
   \text{(\localref{us-desugar-vs})}
   \notag
   \\
   &
   \exRec{\seq{\bind{y}{v}}^\ddagger} \subseteq \exRec{\seq{\bind{x}{v}}^\dagger}
   \textit{ with }
   \seq{u}^\ddagger \desugar \seq{v}^\ddagger
   \quad
   (\exists \seq{v}^\ddagger)
   &
   \notag
   \\
   &
   \seq{u}^\ddagger \concat \seq{u}' \desugar \seq{v}^\ddagger \concat \seq{v}'
   &
   \notag
   \\
   &
   \seq{v}^\ddagger \concat \seq{v}', \kappa \match \gamma', e
   \textit{ with }
   \gamma \desugar \gamma'\textit{ and }s \desugar e
   \quad
   (\exists \gamma', e)
   &
   \text{IH}
   \notag
   \\
   &
   \qedLocal
   \derivation{\derivationWidth}{
      \begin{smathpar}
         \inferrule*[
            left={\ruleName{$\match$-record}}
         ]
         {
            \seq{v}^\ddagger \concat \seq{v}', \kappa \match \gamma', e
            \\
            \exRec{\seq{\bind{y}{v}}^\ddagger} \subseteq \exRec{\seq{\bind{x}{v}}^\dagger}
         }
         {
            \Lowlight{\seq{v} =\;}\exRec{\seq{\bind{x}{v}}^\dagger} \cons \seq{v}',
            \elimRecord{\seq{y}}{\kappa}
            \match
            \gamma', e
         }
      \end{smathpar}
   }
   &
   \notag
   \\
   \intertext{\crossrule}
   %%%%%%%%%%%%%%%%%%%%%%%%%%%
   &
   \caseDerivation{\derivationWidth}{
      \begin{smathpar}
         \inferrule*[
            left={\ruleName{$\match$-constr}}
         ]
         {
            \seq{u}^\dagger \concat \seq{u}',
            (\pi_i \clauseWith{\concat} k_i \mid c_i = c)
            \match \gamma, s
         }
         {
            \Lowlight{\seq{u} =\;}
            \exConstr{c}{\seq{u}^\dagger} \cons \seq{u}',
            \seq{(\pattConstr{c}{\pi} \clauseWith{\cons} k)}
            \match
            \gamma, s
         }
      \end{smathpar}
   }
   &
   \notag
   \\
   &
   \derivation{\derivationWidth}{
      \begin{smathpar}
         \inferrule*[
            left={\ruleName{$\desugar$-clauses-constr}}
         ]
         {
            (\pi_i \clauseWith{\concat} k_i \mid c_i = c') \desugar \kappa_{c'}
            \\
            \datatype{c'} = D
            \quad
            (\forall c' \in \set{\seq{c}})
         }
         {
            \seq{\pattConstr{c}{\pi} \clauseWith{\cons} k}
            \desugar
            \elimConstr{\elimBind{c'}{\kappa_{c'}} \mid c' \in \set{\seq{c}}}
            \Lowlight{\;= \kappa}
         }
      \end{smathpar}
   }
   &
   \text{inversion}
   \locallabel{constr-inversion}
   \\
   &
   \seq{v} = \exConstr{c}{\seq{v}^\dagger} \cons \seq{v}'
   \textit{ with }
   \seq{u}^\dagger \desugar \seq{v}^\dagger
   \textit{ and }
   \seq{u}' \desugar \seq{v}'
   \quad
   (\exists \seq{v}^\dagger, \seq{v}')
   &
   \text{(\localref{us-desugar-vs})}
   \notag
   \\
   &
   \seq{u}^\dagger \concat \seq{u}' \desugar \seq{v}^\dagger \concat \seq{v}'
   &
   \notag
   \\
   &
   (\pi_i \clauseWith{\concat} k_i \mid c_i = c) \desugar \kappa_{c}
   &
   \text{(\localref{constr-inversion})}
   \notag
   \\
   &
   \seq{v}^\dagger \concat \seq{v}', \kappa_c \match \gamma', e
   \textit{ with }
   \gamma' \desugar \gamma
   \textit{ and }
   s \desugar e
   \quad
   (\exists \gamma', e)
   &
   \text{IH}
   \notag
   \\
   &
   \sigma \eqdef
   \kappa \setminus \set{\elimBind{c}{\kappa_c}}
   &
   \notag
   \\
   &
   \qedLocal
   \derivation{\derivationWidth}{
      \begin{smathpar}
         \inferrule*[lab={\ruleName{$\match$-constr}}]
         {
            \seq{v}^\dagger \concat \seq{v}', \kappa_c \match \gamma', e
         }
         {
            \Lowlight{\seq{v} =\;}
            \exConstr{c}{\seq{v}^\dagger} \cons \seq{v}', \Lowlight{\kappa =\;}((\elimBind{c}{\kappa_c}) \cons \sigma)
            \match
            \gamma', e
         }
      \end{smathpar}
   }
   &
   \notag
\end{flalign}
\end{proof}

\subsection{\thmref{semantics-eq}}
\label{app:proofs:semantics-eq}

It is sufficient (but less verbose) to prove the following:
\begin{theorem}
   \label{thm:app:proofs:semantics-eq}
   Suppose $s \desugar e$ and $\gamma \desugar \gamma'$.
   \begin{enumerate}
      \item If $\gamma, s \evalS v$ then $\exists v'.\;\gamma', e \evalS v'$ with $v \desugar v'$.
      \item If $\gamma', e \evalS v'$ then $\exists v.\;\gamma, s \evalS v$.
   \end{enumerate}
\end{theorem}

\noindent Technically $v \desugar v'$ in part (2) follows easily from part (1) and the determinism of
desugaring and the surface semantics
(\lemrefTwo{surface:eval:determinism}{desugar:determinism}); however the stronger induction
hypothesis is more convenient for the proof.

\subsubsection{\thmref{app:proofs:semantics-eq} part (1)}
\setcounter{equation}{0}
\proofContext{semantics-eq}
Case analysis on surface $\evalS$ derivation and induction on $\desugar$ derivation.
\begin{proof}
\small
\begin{flalign}
   &
   s_0 \desugar e_0
   &
   \text{suppose}
   \locallabel{desug:expr}
   \\
   &
   \gamma \desugar \gamma'
   &
   \text{suppose}
   \locallabel{desug:env}
   \\
   &
   \gamma, s_0 \evalSugS v_0
   &
   \text{suppose}
   \locallabel{eval:surf}
   \\
   \intertext{\crossrule}
   %%%%%%%%%%%%%%%%%%%%%%%%%%%%%%%%%%%%%%%%%%%%%%%%%%%%%%%%%%%%%%%%%%%%%%%%
   &
   \caseDerivation{\derivationWidth}{
      \begin{smathpar}
         \inferrule*[
            lab={\ruleName{$\desugar$-var}}
         ]
         {
            \strut
         }
         {
            \Lowlight{s_0 =\;} \exVar{x} \desugar \exVar{x} \Lowlight{\;= e_0}
         }
      \end{smathpar}
   }
   &
   \notag
   \\
   &
   \derivation{\derivationWidth}{
      \begin{smathpar}
         \inferrule*[
            lab={\ruleName{$\evalSugS$-var}}
         ]
         {
            \strut
         }
         {
            \Lowlight{\gamma =\;} {\gamma_1} \cons (\bind{x}{v}), \exVar{x} \evalSugS v
         }
      \end{smathpar}
   }
   &
   \notag
   \\
   &
   \gamma_1\cons(\bind{x}{v}) \desugar \gamma_2\cons(\bind{x}{v'})
   \textit{ with }
   v \desugar v'
   \quad
   (\exists \gamma_2, v')
   &
   (\text{\localref{desug:env}), \ruleName{$\desugar$-env}}
   \notag
   \\
   &
   \qedLocal
   \derivation{\derivationWidth}{
      \begin{smathpar}
         \inferrule*[
            lab={\ruleName{$\evalSugS$-var}}
         ]
         {
            \strut
         }
         {
            \gamma_2 \cdot (\bind{\exVar{x}}{v'}), \exVar{x} \evalSugS v'
         }
      \end{smathpar}
   }
   &
   \notag
   \\
   \intertext{\crossrule}
   %%%%%%%%%%%%%%%%%%%%%%%%%%%%%%%%%%%%%%%%%%%%%%%%%%%%%%%%%%%%%%%%%%%%%%%%
   &
   \caseDerivation{\derivationWidth}{
      \begin{smathpar}
         \inferrule*[
            lab={\ruleName{$\desugar$-constr}}
         ]
         {
            \seq{s} \desugar \seq{e}
         }
         {
            \exConstr{c}{\seq{s}} \desugar \exConstr{c}{\seq{e}}
         }
      \end{smathpar}
   }
   &
   \notag
   \\
   &
   \derivation{\derivationWidth}{
      \begin{smathpar}
         \inferrule*[
            lab={\ruleName{$\evalSugS$-constr}}
         ]
         {
            \gamma, \seq{s} \evalSugS \seq{v}
         }
         {
            \gamma, \exConstr{c}{\seq{s}} \evalSugS \exConstr{c}{\seq{v}}
         }
      \end{smathpar}
   }
   &
   \notag
   \\
   &
   \gamma', e \evalSugS \seq{v}'
   \textit{ with }
   \seq{v} \desugar \seq{v}'
   \quad
   (\exists \seq{v}')
   &
   \text{IH}
   \notag
   \\
   &
   \qedLocal
   \derivation{\derivationWidth}{
      \begin{smathpar}
         \inferrule*[
            lab={\ruleName{$\evalSugS$-constr}}
         ]
         {
            \gamma', \seq{e} \evalSugS \seq{v}'
         }
         {
            \gamma', \exConstr{c}{\seq{e}} \evalSugS \exConstr{c}{\seq{v}'}
         }
      \end{smathpar}
   }
   &
   \notag
   \\
   &
   \qedLocal
   \derivation{\derivationWidth}{
      \begin{smathpar}
         \inferrule*[
            lab={\ruleName{$\desugar$-constr}}
         ]
         {
            \seq{v} \desugar \seq{v}'
         }
         {
            \exConstr{c}{\seq{v}} \desugar \exConstr{c}{\seq{v}'}
         }
      \end{smathpar}
   }
   &
   \notag
   \intertext{\crossrule}
   %%%%%%%%%%%%%%%%%%%%%%%%%%%%%%%%%%%%%%%%%%%%%%%%%%%%%%%%%%%%%%%%%%%%%%%%
   &
   \caseDerivation{\derivationWidth}{
      \begin{smathpar}
         \inferrule*[
            lab={\ruleName{$\desugar$-app}}
         ]
         {
            s \desugar e
            \\
            s' \desugar e'
         }
         {
            \exApp{s}{s'} \desugar \exApp{e}{e'}
         }
      \end{smathpar}
   }
   &
   \notag
   \\
   &
   \derivation{\derivationWidth}{
      \begin{smathpar}
         \inferrule*[
            lab={\ruleName{$\evalSugS$-app}},
            width=3in,
         ]
         {
            \gamma, s \evalSugS \exClosure{\gamma_1}{g}{\mu}
            \\
            \gamma, s' \evalSugS v
            \\
            \gamma_1, g \closeDefs \gamma_2
            \\
            v, \mu \match \gamma_3, s^\dag
            \\
            \gamma_1 \concat \gamma_2 \concat \gamma_3, s^\dag \evalSugR{S^\dag} v^{\dag}
         }
         {
            \gamma, \exApp{s}{s'} \evalSugR{\trApp{S}{S'}{p}{S^{\dag}}} v^{\dag}
         }
      \end{smathpar}
   }
   &
   \notag
   \\
   &
   \gamma', e \evalSugS \exClosure{\gamma'_1}{\rho}{\sigma}
   \textit{ with }
   \gamma_1 \desugar \gamma_1'
   \textit{ and }
   g \desugar \rho
   \textit{ and }
   \mu \desugar \sigma
   \quad
   (\exists \gamma_1',\rho,\sigma)
   &
   \text{IH, $\desugar$-closure}
   \notag
   \\
   &
   \gamma', e' \evalSugS v'
   \textit{ with }
   v \desugar v'
   \quad
   (\exists v')
   &
   \text{IH}
   \notag
   \\
   &
   \gamma'_1, \rho \closeDefs \gamma'_2
   \textit{ with }
   \gamma_2 \desugar \gamma'_2
   \quad
   (\exists \gamma'_2)
   &
   \text{\lemref{closedefs-eq}}
   \notag
   \\
   &
   v', \sigma \match \gamma'_3, e^{\dag}
   \textit{ with }
   \gamma_3 \desugar \gamma'_3
   \textit{ and }
   s^{\dag} \desugar e^{\dag}
   \quad
   (\exists \gamma'_3, e^{\dag})
   &
   \text{\lemref{match-eq}}
   \notag
   \\
   &
   \gamma_1\concat\gamma_2\concat\gamma_3 \desugar \gamma'_1\concat\gamma'_2\concat\gamma'_3
   &
   \text{\ruleName{$\desugar$-env}}
   \notag
   \\
   &
   \gamma'_1 \concat \gamma'_2 \concat \gamma'_3, e^{\dag} \evalSugS u
   \textit{ with }
   v^{\dag} \desugar u
   \quad
   (\exists u)
   &
   \text{IH}
   \notag
   \\
   &
   \qedLocal
   \derivation{\derivationWidth}{
      \begin{smathpar}
         \inferrule*[
            lab={\ruleName{$\evalSugS$-app}},
            width=3.3in,
         ]
         {
            \gamma', (e, e') \evalS (\exClosure{\gamma_1}{\rho}{\sigma}, v')
            \\
            \gamma'_1, \rho \closeDefs \gamma'_2
            \\
            v', \sigma \match \gamma'_3, e^{\dag}
            \\
            \gamma'_1 \concat \gamma'_2 \concat \gamma'_3, e^{\dag} \evalSugS u
         }
         {
            \gamma', \exApp{e}{e'}
            \evalSugS
            u
         }
      \end{smathpar}
   }
   &
   \notag
   \\
   \intertext{\crossrule}
   %%%%%%%%%%%%%%%%%%%%%%%%%%%%%%%%%%%%%%%%%%%%%%%%%%%%%%%%%%%%%%%%%%%%%%%%
   &
   \caseDerivation{\derivationWidth}{
      \begin{smathpar}
         \inferrule*[lab={\ruleName{$\desugar$-let-rec}}]
         {
            \seq{\mu} \desugar \seq{\sigma}
            \\
            s \desugar e
         }
         {
            \exLetRecPiecewise{\seq{\bind{x}{\mu}}}{s}
            \desugar
            \exLetRecPiecewise{\seq{\bind{x}{\sigma}}}{e}
         }
      \end{smathpar}
   }
   &
   \notag
   \\
   &
   \derivation{\derivationWidth}{
      \begin{smathpar}
         \inferrule*[
            lab={\ruleName{$\evalSugS$-let-rec}}
         ]
         {
            \gamma, \seq{\bind{x}{\mu}} \closeDefs \gamma^{\dag}
            \\
            \gamma \concat \gamma^{\dag}, s \evalSugS v
         }
         {
            \gamma, \exLetRecPiecewise{\seq{\bind{x}{\mu}}}{s} \evalSugS v
         }
      \end{smathpar}
   }
   &
   \notag
   \\
   &
   \gamma', \seq{\bind{x}{\sigma}} \closeDefs \gamma^{\ddagger}
   \textit{ with }
   \gamma^{\dag} \desugar \gamma^{\ddagger}
   \quad
   (\exists \gamma^\ddagger)
   &
   \text{\lemref{closedefs-eq}}
   \notag
   \\
   &
   \gamma \concat \gamma^{\dag} \desugar \gamma' \concat \gamma^{\ddagger}
   &
   \text{\ruleName{$\desugar$-env}, (\localref{desug:env})}
   \notag
   \\
   &
   \gamma' \concat \gamma^{\ddagger}, e \evalSugS v'
   \textit{ with }
   v \desugar v'
   \quad
   (\exists v')
   &
   \text{IH}
   \notag
   \\
   &
   \qedLocal
   \derivation{\derivationWidth}{
      \begin{smathpar}
         \inferrule*[lab={\ruleName{$\evalSugS$-let-rec}}]
         {
            \gamma', \seq{\bind{\exVar{x}}{\sigma}} \closeDefs {\gamma^{\ddagger}}
            \\
            \gamma' \concat {\gamma^{\ddagger}}, e \evalSugS v'
         }
         {
            \gamma', \exLetRecPiecewise{\seq{\bind{\exVar{x}}{\sigma}}}{e} \evalSugS v'
         }
      \end{smathpar}
   }
   &
   \notag
   \\
   \intertext{\crossrule}
   %%%%%%%%%%%%%%%%%%%%%%%%%%%%%%%%%%%%%%%%%%%%%%%%%%%%%%%%%%%
   &
   \caseDerivation{\derivationWidth}{
      \begin{smathpar}
         \inferrule*[lab={\ruleName{$\desugar$-list-comp-done}}]
         {
            s \desugar e
         }
         {
            \exListComp{s}{\seqEmpty}
            \desugar
            \exConstr{\cCons}{e, \exNil}
         }
      \end{smathpar}
   }
   &
   \notag
   \\
   &
   \derivation{\derivationWidth}{
      \begin{smathpar}
         \inferrule*[lab={\ruleName{$\evalSugS$-list-comp-done}}]
         {
            \gamma, s \evalSugR{S} u
         }
         {
            \gamma, \exListComp{s}{\seqEmpty} \evalSugR{\seqEmpty, S} \exConstr{\cCons}{u, \exNil}
         }
      \end{smathpar}
   }
   &
   \notag
   \\
   &
   \gamma', e \evalS v
   \textit{ with }
   u \desugar v
   \quad
   (\exists v)
   &
   \text{IH}
   \notag
   \\
   &
   \qedLocal
   \derivation{\derivationWidth}{
      \begin{smathpar}
         \inferrule*[
            lab={\ruleName{$\evalS$-constr}}
         ]
         {
            \gamma', e \evalS v
         }
         {
            \gamma', \exConstr{\cCons}{e, \exNil} \evalS \exConstr{\cCons}{v, \exNil}
         }
      \end{smathpar}
   }
   &
   \notag
   \\
   \intertext{\crossrule}
   %%%%%%%%%%%%%%%%%%%%%%%%%%%%%%%%%%%%%%%%%%%%%%%%%%%%%%%%%%%
   &
   \caseDerivation{\derivationWidth}{
      \begin{smathpar}
         \inferrule*[lab={\ruleName{$\desugar$-list-comp-guard}}]
         {
            s \desugar e
            \\
            \exListComp{s'}{\seq{q}} \desugar e'
            \\
            \sigma = \elimConstr{\elimBind{\cTrue}{e'}, \elimBind{\cFalse}{\exNil}}
         }
         {
            \exListComp{s'}{\qualGuard{s} \cons \seq{q}}
            \desugar
            \exApp{\exFun{\sigma}}{e}
         }
      \end{smathpar}
   }
   &
   \notag
   \\
   &
   \derivation{\derivationWidth}{
      \begin{smathpar}
         \inferrule*[
            lab={\ruleName{$\evalSugS$-list-comp-guard-false}}
         ]
         {
            \gamma, s \evalSugR{S} \cFalse
         }
         {
            \gamma, \exListComp{s'}{\qualGuard{s} \cons \seq{q}} \evalSugR{\trQualIfFalse{S}{q}} \exNil
         }
      \end{smathpar}
   }
   &
   \notag
   \\
   &
   \gamma', e \evalS \cFalse
   &
   \text{IH}
   \notag
   \\
   &
   \cFalse, \sigma \match \envEmpty, \exNil
   &
   \text{\ruleName{$\match$-constr}}
   \notag
   \\
   &
   \gamma', \envEmpty \closeDefs \envEmpty
   &
   \text{\defref{core:close-defs}}
   \notag
   \\
   &
   \gamma', \exNil \evalS \exNil
   &
   \text{\ruleName{$\evalS$-constr}}
   \notag
   \\
   &
   \qedLocal
   \derivation{\derivationWidth}{
      \begin{smathpar}
         \inferrule*[
            lab={\ruleName{$\evalSugS$-app}},
            width=3.3in,
         ]
         {
            \gamma', \exFun{\sigma} \evalS \exClosure{\gamma'}{\envEmpty}{\sigma}
            \\
            \gamma', e \evalS \cFalse
            \\
            \gamma', \envEmpty \closeDefs \envEmpty
            \\
            \cFalse, \sigma \match \envEmpty, \exNil
            \\
            \gamma' \concat \envEmpty \concat \envEmpty, \exNil \evalSugS \exNil
         }
         {
            \gamma', \exApp{\exFun{\sigma}}{e}
            \evalSugS
            \exNil
         }
      \end{smathpar}
   }
   &
   \notag
   \\
   \intertext{\crossrule}
   %%%%%%%%%%%%%%%%%%%%%%%%%%%%%%%%%%%%%%%%%%%%%%%%%%%%%%%%%%%
   &
   \caseDerivation{\derivationWidth}{
      \begin{smathpar}
         \inferrule*[lab={\ruleName{$\desugar$-list-comp-guard}}]
         {
            s \desugar e
            \\
            \exListComp{s'}{\seq{q}} \desugar e'
            \\
            \sigma = \elimConstr{\elimBind{\cTrue}{e'}, \elimBind{\cFalse}{\exNil}}
         }
         {
            \exListComp{s'}{\qualGuard{s} \cons \seq{q}}
            \desugar
            \exApp{\exFun{\sigma}}{e}
         }
      \end{smathpar}
   }
   &
   \notag
   \\
   &
   \derivation{\derivationWidth}{
      \begin{smathpar}
         \inferrule*[
            lab={\ruleName{$\evalSugS$-list-comp-guard-true}},
         ]
         {
            \gamma, \exListComp{s'}{\seq{q}} \evalSugR{\seq{Q},S} v
            \\
            \gamma, s \evalSugR{S} \cTrue
         }
         {
            \gamma, \exListComp{s'}{\qualGuard{s} \cons \seq{q}} \evalSugR{\trQualIfTrue{S} \cons \seq{Q}, S} v
         }
      \end{smathpar}
   }
   &
   \notag
   \\
   &
   \gamma', e \evalS \cTrue
   &
   \text{IH}
   \notag
   \\
   &
   \cTrue, \sigma \match \envEmpty, e'
   &
   \text{\ruleName{$\match$-constr}}
   \notag
   \\
   &
   \gamma', e' \evalS v'
   \textit{ with }
   v \desugar v'
   \quad
   (\exists v')
   &
   \text{IH}
   \notag
   \\
   &
   \gamma, \envEmpty \closeDefs \envEmpty
   &
   \text{\defref{core:close-defs}}
   \notag
   \\
   &
   \qedLocal
   \derivation{\derivationWidth}{
      \begin{smathpar}
         \inferrule*[
            lab={\ruleName{$\evalSugS$-app}},
            width=3.3in,
         ]
         {
            \gamma', \exFun{\sigma} \evalS \exClosure{\gamma'}{\envEmpty}{\sigma}
            \\
            \gamma', e \evalS \cTrue
            \\
            \gamma', \envEmpty \closeDefs \envEmpty
            \\
            \cTrue, \sigma \match \envEmpty, e'
            \\
            \gamma' \concat \envEmpty \concat \envEmpty, e' \evalSugS v'
         }
         {
            \gamma', \exApp{\exFun{\sigma}}{e}
            \evalSugS
            v'
         }
      \end{smathpar}
   }
   &
   \notag
   \\
   \intertext{\crossrule}
   %%%%%%%%%%%%%%%%%%%%%%%%%%%%%%%%%%%%%%%%%%%%%%%%%%%%%%%%%%%
   &
   \caseDerivation{\derivationWidth}{
      \begin{smathpar}
         \inferrule*[lab={\ruleName{$\desugar$-list-comp-decl}}]
         {
            s \desugar e
            \\
            (\clause{p}{\exListComp{s'}{\seq{q}}}) \desugar \sigma
         }
         {
            \exListComp{s'}{\qualDeclaration{p}{s} \cons \seq{q}}
            \desugar
            \exApp{\exFun{\sigma}}{e}
         }
      \end{smathpar}
   }
   &
   \notag
   \\
   &
   \derivation{\derivationWidth}{
      \begin{smathpar}
         \inferrule*[
            lab={\ruleName{$\evalSugS$-list-comp-decl}}
         ]
         {
            \gamma, s \evalSugR{S'} u'
            \\
            u', (\clause{p}{\exListComp{s'}{\seq{q}}}) \match \gamma^\dag, s^\dag
            \\
            \gamma \concat \gamma^\dag, s^\dag \evalSugR{\seq{Q},S} u
         }
         {
            \gamma, \exListComp{s'}{\qualDeclaration{p}{s} \cons \seq{q}} \evalSugR{\trQualDecl{p}{S'} \cons \seq{Q}, S} u
         }
      \end{smathpar}
   }
   &
   \notag
   \\
   &
   \gamma', e \evalS v'
   \textit{ with }
   u' \desugar v'
   \quad
   (\exists v')
   &
   \text{IH}
   \notag
   \\
   &
   v', \sigma \match \gamma^\ddagger, e^\dag
   \textit{ with }
   \gamma^\dag \desugar \gamma^\ddagger
   \textit{ and }
   s^\dag \desugar e^\dag
   \quad
   (\exists \gamma^\ddagger, e^\dag)
   &
   \text{\lemref{match-eq}}
   \notag
   \\
   &
   \gamma', \exFun{\sigma} \evalS \exClosure{\gamma'}{\envEmpty}{\sigma}
   \textit{ with }
   \gamma \desugar \gamma'
   &
   \text{\ruleName{$\evalS$-lambda}}
   \notag
   \\
   &
   \gamma', \envEmpty \closeDefs \envEmpty
   &
   \text{\defref{surface:close-defs}}
   \notag
   \\
   &
   \gamma' \concat \envEmpty \concat \gamma^\ddagger, e^\dag \evalS u^\dag
   \textit{ with }
   u \desugar u^\dag
   \quad
   (\exists u^\dag)
   &
   \text{IH}
   \notag
   \\
   &
   \qedLocal
   \derivation{\derivationWidth}{
      \begin{smathpar}
         \inferrule*[
            lab={\ruleName{$\evalSugS$-app}},
            width=3.3in,
         ]
         {
            \gamma', (\exFun{\sigma}, e) \evalS (\exClosure{\gamma'}{\envEmpty}{\sigma}, v')
            \\
            \gamma', \envEmpty \closeDefs \envEmpty
            \\
            v', \sigma \match \gamma^\ddagger, e^\dag
            \\
            \gamma' \concat \envEmpty \concat \gamma^\ddagger, e^\dag \evalSugS u^\dag
         }
         {
            \gamma', \exApp{\exFun{\sigma}}{e}
            \evalSugS
            u^\dag
         }
      \end{smathpar}
   }
   &
   \notag
   \\
   \intertext{\crossrule}
   %%%%%%%%%%%%%%%%%%%%%%%%%%%%%%%%%%%%%%%%%%%%%%%%%%%%%%%%%%%
   &
   \caseDerivation{\derivationWidth}{
      \begin{smathpar}
         \inferrule*[lab={\ruleName{$\desugar$-list-comp-gen}}]
         {
            s \desugar e
            \\
            (\clause{p}{\exListComp{s'}{\seq{q}}}), \exNil \orElse \mu
            \\
            \mu \desugar \sigma
         }
         {
            \exListComp{s'}{\qualGenerator{p}{s} \cons \seq{q}}
            \desugar
            \exApp{\exApp{\varConcatMap}{\exFun{\sigma}}}{e}
         }
      \end{smathpar}
   }
   &
   \notag
   \\
   &
   \derivation{\derivationWidth}{
      \begin{smathpar}
         \inferrule*[
            lab={\ruleName{$\evalSugS$-list-comp-gen}},
            flushleft
         ]
         {
            (\clause{p}{\exListComp{s'}{\seq{q}}}), \exNil \orElse \mu
            \\
            \gamma, \exApp{\exApp{\varConcatMap}{\exFun{\mu}}}{s} \evalSugS u
         }
         {
            \gamma, \exListComp{s'}{\qualGenerator{p}{s} \cons \seq{q}} \evalSugR{\trQualGen{p}{S'}\cons\seq{Q}, S} u
         }
      \end{smathpar}
   }
   &
   \notag
   \\
   &
   \derivation{\derivationWidth}{
      \begin{smathpar}
         \inferrule*[left=\ruleName{$\desugar$-app}]
         {
            \inferrule*[
               left={\ruleName{$\desugar$-app}}
            ]
            {
               \inferrule*[
%                  left={\ruleName{$\desugar$-var}}
               ]
               {
                  \strut
               }
               {
                  \varConcatMap \desugar \varConcatMap
               }
               \\
               \inferrule*[
                  left={\ruleName{$\desugar$-lambda}}
               ]
               {
                  \mu \desugar \sigma
               }
               {
                  \exFun{\mu} \desugar \exFun{\sigma}
               }
            }
            {
               \exApp{\varConcatMap}{\exFun{\mu}} \desugar \exApp{\varConcatMap}{\exFun{\sigma}}
            }
            \\
            s \desugar e
         }
         {
            \exApp{\exApp{\varConcatMap}{\exFun{\mu}}}{s} \desugar \exApp{\exApp{\varConcatMap}{\exFun{\sigma}}}{e}
         }
      \end{smathpar}
   }
   &
   \notag
   \\
   &
   \qedLocal
   \gamma', \exApp{\exApp{\varConcatMap}{\exFun{\sigma}}}{e} \evalS v
   \textit{ with }
   u \desugar v
   \quad
   (\exists v)
   &
   \text{IH}
   \notag
\end{flalign}
\end{proof}

\subsubsection{\thmref{app:proofs:semantics-eq} part (2)}
\setcounter{equation}{0}
\proofContext{semantics-eq-2}
Case analysis on surface $\evalS$ derivation and induction on $\desugar$ derivation.
\begin{proof}
\small
\begin{flalign}
   &
   s_0 \desugar e_0
   &
   \text{suppose}
   \locallabel{desug:expr}
   \\
   &
   \gamma \desugar \gamma'
   &
   \text{suppose}
   \locallabel{desug:env}
   \\
   &
   \gamma', e_0 \evalSugS v'_0
   &
   \text{suppose}
   \locallabel{eval:core}
   \\
   \intertext{\crossrule}
   %%%%%%%%%%%%%%%%%%%%%%%%%%%%%%%%%%%%%%%%%%%%%%%%%%%%%%%%%%%%%%%%%%%%%%%%
   &
   \caseDerivation{\derivationWidth}{
      \begin{smathpar}
         \inferrule*[
            lab={\ruleName{$\desugar$-var}}
         ]
         {
            \strut
         }
         {
            s_0 = \exVar{x} \desugar \exVar{x} \Lowlight{\;= e_0}
         }
      \end{smathpar}
   }
   &
   \notag
   \\
   &
   \derivation{\derivationWidth}{
      \begin{smathpar}
         \inferrule*[
            lab={\ruleName{$\evalSugS$-var}}
         ]
         {
            \strut
         }
         {
            \Lowlight{\gamma' =\;}\gamma_2 \cdot (\bind{x}{v'}), x \evalSugS v'
         }
      \end{smathpar}
   }
   &
   \notag
   \\
   &
   \gamma = \gamma_1 \cons (\bind{x}{v}) \desugar \gamma_2 \cons (\bind{x}{v'})
   \textit{ with }v \desugar v'
   \quad
   (\exists \gamma_1, v)
   &
   \text{(\localref{desug:env}), inversion \ruleName{$\desugar$-env}}
   \notag
   \\
   &
   \qedLocal
   \derivation{\derivationWidth}{
      \begin{smathpar}
         \inferrule*[
            lab={\ruleName{$\evalSugS$-var}}
         ]
         {
            \strut
         }
         {
            \Lowlight{\gamma =\;} \gamma_1 \cons (\bind{x}{v}), \exVar{x} \evalSugS v
         }
      \end{smathpar}
   }
   &
   \notag
   \\
   \intertext{\crossrule}
   %%%%%%%%%%%%%%%%%%%%%%%%%%%%%%%%%%%%%%%%%%%%%%%%%%%%%%%%%%%%%%%%%%%%%%%%
   &
   \caseDerivation{\derivationWidth}{
      \begin{smathpar}
         \inferrule*[
            lab={\ruleName{$\desugar$-constr}}
         ]
         {
            \seq{s} \desugar \seq{e}
         }
         {
            \exConstr{c}{\seq{s}} \desugar \exConstr{c}{\seq{e}}
         }
      \end{smathpar}
   }
   &
   \notag
   \\
   &
   \derivation{\derivationWidth}{
      \begin{smathpar}
         \inferrule*[
            lab={\ruleName{$\evalSugS$-constr}}
         ]
         {
            \gamma', \seq{e} \evalSugS \seq{v}'
         }
         {
            \gamma', \exConstr{c}{\seq{e}} \evalSugS \exConstr{c}{\seq{v}'}
         }
      \end{smathpar}
   }
   &
   \notag
   \\
   &
   \gamma, \seq{s} \evalSugS \seq{v}
   \textit{ with }
   \seq{v} \desugar \seq{v}'
   \quad
   (\exists \seq{v})
   &
   \text{IH}
   \notag
   \\
   &
   \qedLocal
   \derivation{\derivationWidth}{
      \begin{smathpar}
         \inferrule*[
            left={\ruleName{$\evalSugS$-constr}}
         ]
         {
            \gamma, \seq{s} \evalSugS \seq{v}
         }
         {
            \gamma, \exConstr{c}{\seq{s}} \evalSugS \exConstr{c}{\seq{v}}
         }
      \end{smathpar}
   }
   &
   \notag
   \\
   &
   \qedLocal
   \derivation{\derivationWidth}{
      \begin{smathpar}
         \inferrule*[
            left={\ruleName{$\desugar$-constr}}
         ]
         {
            \seq{v} \desugar \seq{v}'
         }
         {
            \exConstr{c}{\seq{v}} \desugar \exConstr{c}{\seq{v}'}
         }
      \end{smathpar}
   }
   &
   \notag
   \\
   \intertext{\crossrule}
   %%%%%%%%%%%%%%%%%%%%%%%%%%%%%%%%%%%%%%%%%%%%%%%%%%%%%%%%%%%%%%%%%%%%%%%%
   &
   \caseDerivation{\derivationWidth}{
      \begin{smathpar}
         \inferrule*[
            lab={\ruleName{$\desugar$-app}}
         ]
         {
            s \desugar e
            \\
            s' \desugar e'
         }
         {
            \Lowlight{s_0 =\;} \exApp{s}{s'} \desugar \exApp{e}{e'} \Lowlight{\;= e_0}
         }
      \end{smathpar}
   }
   &
   \notag
   \\
   &
   \derivation{\derivationWidth}{
      \begin{smathpar}
         \inferrule*[
            lab={\ruleName{$\evalSugS$-app}},
            width=3.3in,
         ]
         {
            \gamma, e \evalS \exClosure{\gamma'_1}{\rho}{\sigma}
            \\
            \gamma, e' \evalS v'
            \\
            \gamma'_1, \rho \closeDefs \gamma'_2
            \\
            v', \sigma \match \gamma'_3, e^{\dag}
            \\
            \gamma'_1 \concat \gamma'_2 \concat \gamma'_3, e^{\dag} \evalSugS u
         }
         {
            \gamma', \exApp{e}{e'}
            \evalSugS
            u
         }
      \end{smathpar}
   }
   &
   \notag
   \\
   &
   \gamma, s \evalSugS \exClosure{\gamma_1}{g}{\mu}
   \textit{ with }
   \gamma_1 \desugar \gamma'_1
   \textit{ and }
   g \desugar \rho
   \textit{ and }
   \mu \desugar \sigma
   \quad
   (\exists \gamma_1, g, \mu)
   &
   \text{IH, \ruleName{$\desugar$-closure}}
   \notag
   \\
   &
   \gamma, s' \evalSugS v
   \textit{ with }
   v \desugar v'
   &
   \text{IH}
   \notag
   \\
   &
   \gamma_1, g \closeDefs \gamma_2
   \textit{ with }
   \gamma_2 \desugar \gamma'_2
   \quad
   (\exists \gamma_2)
   &
   \text{\lemref{closedefs-eq}}
   \notag
   \\
   &
   v, \mu \match \gamma_3, s^{\dag}
   \textit{ with }
   \gamma_3 \desugar \gamma'_3
   \textit{ and }
   s^{\dag} \desugar e^{\dag}
   \quad
   (\exists \gamma_3, s^{\dag})
   &
   \text{\lemref{match-eq}}
   \notag
   \\
   &
   \gamma_1\concat\gamma_2\concat\gamma_3 \desugar \gamma'_1\concat\gamma'_2\concat\gamma'_3
   &
   \text{\ruleName{$\desugar$-env}}
   \notag
   \\
   &
   \gamma_1 \concat \gamma_2 \concat \gamma_3, s^{\dag} \evalSugS v^{\dag}
   \textit{ with }
   v^{\dag} \desugar u
   \quad
   (\exists v^\dag)
   &
   \text{IH}
   \notag
   \\
   &
   \qedLocal
   \derivation{\derivationWidth}{
      \begin{smathpar}
         \inferrule*[
            lab={\ruleName{$\evalSugS$-app}},
            width=3in,
         ]
         {
            \gamma, s \evalSugR{(S,S')} \exClosure{\gamma_1}{g}{\mu}
            \\
            \gamma, s' \evalSugR{(S,S')} v
            \\
            \gamma_1, g \closeDefs \gamma_2
            \\
            v, \mu \match \gamma_3, s^\dag
            \\
            \gamma_1 \concat \gamma_2 \concat \gamma_3, s^\dag \evalSugR{S^\dag} v^{\dag}
         }
         {
            \gamma, \exApp{s}{s'} \evalSugR{\trApp{S}{S'}{p}{S^{\dag}}} v^{\dag}
         }
      \end{smathpar}
   }
   &
   \notag
   \\
   \intertext{\crossrule}
   %%%%%%%%%%%%%%%%%%%%%%%%%%%%%%%%%%%%%%%%%%%%%%%%%%%%%%%%%%%%%%%%%%%%%%%%
   &
   \caseDerivation{\derivationWidth}{
      \begin{smathpar}
         \inferrule*[lab={\ruleName{$\desugar$-let-rec}}]
         {
            \seq{\mu} \desugar \seq{\sigma}
            \\
            s \desugar e
         }
         {
            \exLetRecPiecewise{\seq{\bind{x}{\mu}}}{s}
            \desugar
            \exLetRecPiecewise{\seq{\bind{x}{\sigma}}}{e}
         }
      \end{smathpar}
   }
   &
   \notag
   \\
   &
   \derivation{\derivationWidth}{
      \begin{smathpar}
         \inferrule*[
            lab={\ruleName{$\evalSugS$-let-rec}}
         ]
         {
            \gamma', \set{\seq{\bind{x}{\sigma}}} \closeDefs \gamma'
            \\
            \gamma' \concat {\gamma^{\ddagger}}, e \evalSugS v
         }
         {
            \gamma', \exLetRec{\seq{\bind{x}{\sigma}}}{e}
            \evalSugS
            v'
         }
      \end{smathpar}
   }
   &
   \notag
   \\
   &
   \gamma, \seq{\bind{x}{\mu}} \closeDefs \gamma^{\dag}
   \textit{ with }
   \gamma^{\dag} \desugar \gamma^{\ddagger}
   \quad
   (\exists \gamma^{\dag})
   &
   \text{\lemref{closedefs-eq}}
   \notag
   \\
   &
   \gamma \concat \gamma^{\dag} \desugar \gamma' \concat \gamma^{\ddagger}
   &
   \text{(\localref{desug:env}), \ruleName{$\desugar$-env}}
   \notag
   \\
   &
   \gamma \concat \gamma^{\dag}, s \evalSugS v
   \textit{ with }
   v \desugar v'
   &
   \text{IH}
   \notag
   \\
   &
   \qedLocal
   \derivation{\derivationWidth}{
      \begin{smathpar}
         \inferrule*[
            lab={\ruleName{$\evalSugS$-let-rec}}
         ]
         {
            \gamma, \seq{\bind{x}{\mu}} \closeDefs \gamma^{\dag}
            \\
            \gamma \concat \gamma^{\dag}, s \evalSugR{S} v
         }
         {
            \gamma, \exLetRecPiecewise{\seq{\bind{x}{\mu}}}{s} \evalSugS v
         }
      \end{smathpar}
   }
   &
   \notag
   \\
   \intertext{\crossrule}
   %%%%%%%%%%%%%%%%%%%%%%%%%%%%%%%%%%%%%%%%%%%%%%%%%%%%%%%%%%%
   &
   \caseDerivation{\derivationWidth}{
      \begin{smathpar}
         \inferrule*[
            lab={\ruleName{$\desugar$-list-comp-done}}
         ]
         {
            s \desugar e
         }
         {
            \exListComp{s}{\seqEmpty} \desugar \exApp{\cCons}{(e, \exNil)}
         }
      \end{smathpar}
   }
   &
   \notag
   \\
   &
   \derivation{\derivationWidth}{
      \begin{smathpar}
         \inferrule*[
            lab={\ruleName{$\evalS$-Cons}}
         ]
         {
            \gamma', e \evalS v'
         }
         {
            \gamma', \exApp{\cCons}{(e, \exNil)} \evalS \exApp{\cCons}{(v', \exNil)}
         }
      \end{smathpar}
   }
   &
   \notag
   \\
   &
   \gamma, s \evalSugS v
   \textit{ with }
   v \desugar v'
   \quad
   (\exists v)
   &
   \text{IH}
   \notag
   \\
   &
   \qedLocal
   \derivation{\derivationWidth}{
      \begin{smathpar}
         \inferrule*[lab={\ruleName{$\evalSugS$-list-comp-done}}]
         {
            \gamma, s \evalSugR{S} v
         }
         {
            \gamma, \exListComp{s}{\seqEmpty} \evalSugR{\seqEmpty, S} \exConstr{\cCons}{v, \exNil}
         }
      \end{smathpar}
   }
   &
   \notag
   \\
   \intertext{\crossrule}
   %%%%%%%%%%%%%%%%%%%%%%%%%%%%%%%%%%%%%%%%%%%%%%%%%%%%%%%%%%%
   &
   \caseDerivation{\derivationWidth}{
      \begin{smathpar}
         \inferrule*[lab={\ruleName{$\desugar$-list-comp-guard}}]
         {
            s \desugar e
            \\
            \exListComp{s'}{\seq{q}} \desugar e'
            \\
            \sigma = \elimConstr{\elimBind{\cTrue}{e'}, \elimBind{\cFalse}{\exNil}}
         }
         {
            \exListComp{s'}{\qualGuard{s} \cons \seq{q}}
            \desugar
            \exApp{\exFun{\sigma}}{e}
         }
      \end{smathpar}
   }
   &
   \notag
   \\
   &
   \textbfit{Subcase}
   &
   \notag
   \\
   &
   \derivation{\derivationWidth}{
      \begin{smathpar}
         \inferrule*[
            lab={\ruleName{$\evalS$-app}},
            width={3in}
         ]
         {
            \gamma', \exFun{\sigma} \evalS \exClosure{\gamma'}{\envEmpty}{\sigma}
            \\
            \gamma', e \evalS \cFalse
            \\
            \cFalse, \sigma \match \envEmpty, \exNil
            \\
            \gamma', \exNil \evalS \exNil
         }
         {
            \gamma', \exApp{\exFun{\sigma}}{e} \evalS \exNil
         }
      \end{smathpar}
   }
   &
   \notag
   \\
   &
   \gamma, s \evalSugS \cFalse
   &
   \text{IH, invert \ruleName{$\desugar$-constr}}
   \notag
   \\
   &
   \qedLocal
   \derivation{\derivationWidth}{
      \begin{smathpar}
         \inferrule*[
            lab={\ruleName{$\evalSugS$-list-comp-guard-false}}
         ]
         {
            \gamma, s \evalSugS \cFalse
         }
         {
            \gamma, \exListComp{s'}{\qualGuard{s} \cdot \seq{q}} \evalSugS \exNil
         }
      \end{smathpar}
   }
   &
   \notag
   \\
   &
   \textbfit{Subcase}
   &
   \notag
   \\
   &
   \derivation{\derivationWidth}{
      \begin{smathpar}
         \inferrule*[
            lab={\ruleName{$\evalS$-app}}
         ]
         {
            \gamma', \exFun{\sigma} \evalS \exClosure{\gamma'}{\envEmpty}{\sigma}
            \\
            \gamma', e \evalS \cTrue
            \\
            \cTrue, \sigma \match \envEmpty, e'
            \\
            \gamma', e' \evalS v'
         }
         {
            \gamma', \exApp{\exFun{\sigma}}{e} \evalS v'
         }
      \end{smathpar}
   }
   &
   \notag
   \\
   &
   \gamma, s \evalSugS \cTrue
   &
   \text{IH, invert \ruleName{$\desugar$-constr}}
   \notag
   \\
   &
   \gamma, \exListComp{s'}{\seq{q}} \evalS v
   \textit{ with }
   v \desugar v'
   \quad
   (\exists v)
   &
   \text{IH}
   \notag
   \\
   &
   \qedLocal
   \derivation{\derivationWidth}{
      \begin{smathpar}
         \inferrule*[
            lab={\ruleName{$\evalSugS$-list-comp-guard-true}}
         ]
         {
            \gamma, s \evalSugS \cTrue
            \\
            \gamma, \exListComp{s'}{\seq{q}} \evalSugS v
         }
         {
            \gamma, \exListComp{s'}{\qualGuard{s} \cdot \seq{q}} \evalSugS v
         }
      \end{smathpar}
   }
   &
   \notag
   \\
   \intertext{\crossrule}
   %%%%%%%%%%%%%%%%%%%%%%%%%%%%%%%%%%%%%%%%%%%%%%%%%%%%%%%%%%%
   &
   \caseDerivation{\derivationWidth}{
      \begin{smathpar}
         \inferrule*[
            lab={\ruleName{$\desugar$-list-comp-decl}},
            width=3.3in,
         ]
         {
            s \desugar e
            \\
            (\clause{p}{\exListComp{s'}{\seq{q}}}) \desugar \sigma
         }
         {
            (\exListComp{s'}{\qualDeclaration{p}{s} \cons \seq{q}}) \desugar \exApp{\exFun{\sigma}}{e}
         }
      \end{smathpar}
   }
   &
   \notag
   \\
   &
   \derivation{\derivationWidth}{
      \begin{smathpar}
         \inferrule*[
            lab={\ruleName{$\evalS$-list-comp-decl}}
         ]
         {
            \gamma', \exFun{\sigma} \evalS \exClosure{\gamma'}{\seqEmpty}{\sigma}
            \\
            \gamma', e' \evalS v'
            \\
            v', \sigma \match \gamma^\ddagger, e^\dag
            \\
            \gamma' \concat \gamma^\ddagger, e^\dag \evalS u^\dag
         }
         {
            \gamma', \exApp{e}{e'} \evalS u^\dag
         }
      \end{smathpar}
   }
   &
   \notag
   \\
   &
   \gamma, s \evalSugS u'
   \textit{ with }
   u' \desugar v'
   \quad
   (\exists u')
   &
   \text{IH}
   \notag
   \\
   &
   u', (\clause{p}{\exListComp{s'}{\seq{q}}}) \match \gamma^\dag, s^\dag
   \textit{ with }
   \gamma^\dag \desugar \gamma^\ddagger
   \textit{ and }
   s^\dag \desugar e^\dag
   \quad
   (\exists \gamma^\dag, s^\dag)
   &
   \text{\lemref{match-eq}}
   \notag
   \\
   &
   \gamma \concat \gamma^\dag, s^\dag \evalSugS v^\dag
   \textit{ with }
   v^\dag \desugar u^\dag
   \quad
   (\exists v^\dag)
   &
   \text{IH}
   \notag
   \\
   &
   \qedLocal
   \derivation{\derivationWidth}{
      \begin{smathpar}
         \inferrule*[
            lab={\ruleName{$\evalSugS$-list-comp-decl}}
         ]
         {
            \gamma, s \evalSugS u'
            \\
            u', (\clause{p}{\exListComp{s'}{\seq{q}}}) \match \gamma^\dag, s^\dag
            \\
            (\gamma \cdot \gamma^\dag), s^\dag \evalS v^\dag
         }
         {
            \gamma, \exListComp{s'}{\qualDeclaration{p}{s} \cdot \seq{q}} \evalS v^\dag
         }
      \end{smathpar}
   }
   &
   \notag
   \\
   \intertext{\crossrule}
   %%%%%%%%%%%%%%%%%%%%%%%%%%%%%%%%%%%%%%%%%%%%%%%%%%%%%%%%%%%
   &
   \caseDerivation{\derivationWidth}{
      \begin{smathpar}
         \inferrule*[lab={\ruleName{$\desugar$-list-comp-gen}}]
         {
            s \desugar e
            \\
            (\clause{p}{\exListComp{s'}{\seq{q}}}), \exNil \orElse \mu
            \\
            \mu \desugar \sigma
         }
         {
            \exListComp{s'}{\qualGenerator{p}{s} \cons \seq{q}}
            \desugar
            \exApp{\exApp{\varConcatMap}{\exFun{\sigma}}}{e}
         }
      \end{smathpar}
   }
   &
   \notag
   \\
   &
   \derivation{\derivationWidth}{
      \begin{smathpar}
         \inferrule*[
            lab=\ruleName{$\evalS$-app},
            width={3in}
         ]
         {
            \gamma', \exApp{\varConcatMap}{\exFun{\sigma}} \evalS \exClosure{\gamma_1}{\rho}{\sigma'}
            \\
            \gamma', e \evalS u
            \\
            \gamma_1, \rho \closeDefs \gamma_2
            \\
            u, \sigma' \match \gamma_3, e'
            \\
            \gamma_1 \concat \gamma_2 \concat \gamma_3, e' \evalS v
         }
         {
            \gamma', \exApp{\exApp{\varConcatMap}{\exFun{\sigma}}}{e} \evalS v
         }
      \end{smathpar}
   }
   &
   \notag
   \\
   &
   \inferrule*[
      left={\ruleName{$\desugar$-app}}
   ]
   {
      \inferrule*[
%         right={\ruleName{$\desugar$-var}}
      ]
      {
         \strut
      }
      {
         \varConcatMap \desugar \varConcatMap
      }
      \\
      \inferrule*[left={\ruleName{$\desugar$-lambda}}]
      {
         \mu \desugar \sigma
      }
      {
         \exFun{\mu} \desugar \exFun{\sigma}
      }
   }
   {
      \exApp{\varConcatMap}{\exFun{\mu}} \desugar \exApp{\varConcatMap}{\exFun{\sigma}}
   }
   &
   \notag
   \\
   &
   \gamma, \exApp{\varConcatMap}{\exFun{\mu}} \evalSugS \exClosure{\gamma_1'}{g}{\mu'}
   \textit{ with }
   \gamma_1' \desugar \gamma_1, g \desugar \rho, \mu' \desugar \sigma'
   \quad
   (\exists \gamma_1')
   &
   \text{IH, \ruleName{$\desugar$-closure}}
   \notag
   \\
   &
   \gamma, s \evalSugS u^\dagger
   \textit{ with }
   u^\dagger \desugar u
   &
   \text{IH}
   \notag
   \\
   &
   \gamma_1', g \closeDefs \gamma_2'
   \textit{ with }
   \gamma_2' \desugar \gamma_2
   &
   \text{\lemref{closedefs-eq}}
   \notag
   \\
   &
   u^\dagger, \mu' \match \gamma_3', s'
   \textit{ with }
   \gamma_3' \desugar \gamma_3\textit{ and }s' \desugar e'
   &
   \text{\lemref{match-seq-eq}}
   \notag
   \\
   &
   \gamma_1' \concat \gamma_2' \concat \gamma_3', s' \evalSugS v^\dagger
   \textit{ with }
   v^\dagger \desugar v
   &
   \text{IH}
   \notag
   \\
   &
   \derivation{\derivationWidth}{
      \begin{smathpar}
         \inferrule*[
            left={\ruleName{$\evalSugS$-app}},
            width={3in}
         ]
         {
            \gamma, \exApp{\varConcatMap}{\exFun{\mu}} \evalSugS \exClosure{\gamma_1'}{g}{\mu'}
            \\
            \gamma, s \evalSugS u^\dagger
            \\
            \gamma_1', g \closeDefs \gamma_2'
            \\
            u^\dagger, \mu' \match \gamma_3', s'
            \\
            \gamma_1' \concat \gamma_2' \concat \gamma_3', s' \evalSugS v^\dagger
         }
         {
            \gamma, \exApp{\exApp{\varConcatMap}{\exFun{\mu}}}{s} \evalSugS v^\dagger
         }
      \end{smathpar}
   }
   &
   \notag
   \\
   &
   \qedLocal
   \derivation{\derivationWidth}{
      \begin{smathpar}
         \inferrule*[
            left={\ruleName{$\evalSugS$-list-comp-gen}}
         ]
         {
            (\clause{p}{\exListComp{s'}{\seq{q}}}), \exNil \orElse \mu
            \\
            \gamma, \exApp{\exApp{\varConcatMap}{\exFun{\mu}}}{s} \evalSugS v^\dagger
         }
         {
            \gamma, \exListComp{s'}{\qualGenerator{p}{s} \cdot \seq{q}} \evalSugS v^\dagger
         }
      \end{smathpar}
   }
   &
   \notag
\end{flalign}
\end{proof}
