# Supplementary material for: Cognacy Queries over Dependence Graphs for Transparent Visualisations
Source: arXiv:2403.04403 source file (2024-10-15)
Supplement: Supplementary file 3 [file desugaring.tex]

\section{Desugaring}

\figref{desugar} defines the desugaring relation $\desugar$, which extends pointwise to sequences.

\begin{lemma}[Determinism of desugaring]
   \label{lem:desugar:determinism}
   If $s \desugar e$ and $s \desugar e'$ then $e = e'$.
\end{lemma}

\begin{figure}
   {\flushleft \shadebox{$s \desugar e$}\hfill}
   \begin{smathpar}
      \inferrule*[lab={\ruleName{$\desugar$-lambda}}]
      {
         \mu \desugar \sigma
      }
      {
         \exFun{\mu} \desugar \exFun{\sigma}
      }
      \and
      \inferrule*[lab={\ruleName{$\desugar$-binary-apply}}]
      {
         s_1 \desugar e_1
         \\
         s_2 \desugar e_2
      }
      {
         \exBinaryApp{s_1}{\oplus}{s_2}
         \desugar
         \exForeignApp{\oplus}{e, e'}
      }
      \and
      \inferrule*[lab={\ruleName{$\desugar$-let-rec}}]
      {
         \seq{\mu} \desugar \seq{\sigma}
         \\
         s \desugar e
      }
      {
         \exLetRecPiecewise{\seq{\bind{x}{\mu}}}{s}
         \desugar
         \exLetRecPiecewise{\seq{\bind{x}{\sigma}}}{e}
      }
      \and
      \inferrule*[lab={\ruleName{$\desugar$-match}}]
      {
         s \desugar e
         \\
         \mu \desugar\sigma
      }
      {
         \exMatch{s}{\mu}
         \desugar
         \exApp{\exFun{\sigma}}{e}
      }
      \and
      \inferrule*[lab={\ruleName{$\desugar$-non-empty-list}}]
      {
         s \desugar e
         \\
         l \desugar e'
      }
      {
         \exList{s}{l}
         \desugar
         \exConstr{\cCons}{e, e'}
      }
      \and
      \inferrule*[lab={\ruleName{$\desugar$-if}}]
      {
         s \desugar e
         \\
         s_1 \desugar e_1
         \\
         s_2 \desugar e_2
         \\
         \sigma = \elimConstr{\elimBind{\cTrue}{e_1}, \elimBind{\cFalse}{e_2}}
      }
      {
         \exIfThenElse{s}{s_1}{s_2}
         \desugar
         \exApp{\exFun{\sigma}}{e}
      }
      \and
      \inferrule*[lab={\ruleName{$\desugar$-list-enum}}]
      {
         s_1 \desugar e
         \\
         s_2 \desugar e'
      }
      {
         \exListEnum{s_1}{s_2}
         \desugar
         \exApp{\exApp{\varEnumFromTo}{e}}{e'}
      }
      \and
      \inferrule*[lab={\ruleName{$\desugar$-list-comp-done}}]
      {
         s \desugar e
      }
      {
         \exListComp{s}{\seqEmpty}
         \desugar
         \exConstr{\cCons}{e, \exNil}
      }
      \and
      \inferrule*[lab={\ruleName{$\desugar$-list-comp-guard}}]
      {
         s \desugar e
         \\
         \exListComp{s'}{\seq{q}} \desugar e'
         \\
         \sigma = \elimConstr{\elimBind{\cTrue}{e'}, \elimBind{\cFalse}{\exNil}}
      }
      {
         \exListComp{s'}{\qualGuard{s} \cons \seq{q}}
         \desugar
         \exApp{\exFun{\sigma}}{e}
      }
      \and
      \inferrule*[lab={\ruleName{$\desugar$-list-comp-decl}}]
      {
         s \desugar e
         \\
         (\clause{p}{\exListComp{s'}{\seq{q}}}) \desugar \sigma
      }
      {
         \exListComp{s'}{\qualDeclaration{p}{s} \cons \seq{q}}
         \desugar
         \exApp{\exFun{\sigma}}{e}
      }
      \and
      \inferrule*[lab={\ruleName{$\desugar$-list-comp-gen}}]
      {
         s \desugar e
         \\
         (\clause{p}{\exListComp{s'}{\seq{q}}}) \orElse \mu
         \\
         \mu \desugar \sigma
      }
      {
         \exListComp{s'}{\qualGenerator{p}{s} \cons \seq{q}}
         \desugar
         \exApp{\exApp{\varConcatMap}{\exFun{\sigma}}}{e}
      }
   \end{smathpar}
   \\[2mm]
   {\flushleft \shadebox{$l \desugar e$}
   \hfill \phantom{blah}}% \textbfit{$l$ desugars to $e$}}
   \begin{smathpar}
      \inferrule*[lab={\ruleName{$\desugar$-list-rest-nil}}]
      {
         \strut
      }
      {
         \exListEnd
         \desugar
         \exListEnd,
         \exNil
      }
      \and
      \inferrule*[lab={\ruleName{$\desugar$-list-rest-cons}}]
      {
         s \desugar e
         \\
         l \desugar e'
      }
      {
         (\exListNext{s}{l})
         \desugar
         \exConstr{\cCons}{e, e'}
      }
   \end{smathpar}
   \\[2mm]
   \begin{minipage}[t]{0.48\textwidth}
      {\small \flushleft \shadebox{$\gamma \desugar \gamma'$}
      \begin{smathpar}
         \inferrule*[lab={\ruleName{$\desugar$-env}}]
         {
            \seq{v} \desugar \seq{v}'
         }
         {
            \set{\seq{\bind{x}{v}}} \desugar \set{\seq{\bind{x}{v}}'}
         }
      \end{smathpar}
      }
   \end{minipage}%
   \hspace{2mm}%
   \begin{minipage}[t]{0.48\textwidth}
      {\small \flushleft \shadebox {$u \desugar v$}
         \begin{smathpar}
            \inferrule*[lab={\ruleName{$\desugar$-closure}}]
            {
                  \gamma \desugar \gamma'
                  \\
                  \seq{\mu} \desugar \seq{\sigma}
                  \\
                  \mu \desugar \sigma
            }
            {
                  \exClosure{\gamma}{\seq{\bind{x}{\mu}}}{\mu} \desugar \exClosure{\gamma'}{\seq{\bind{x}{\sigma}}}{\sigma}
            }
         \end{smathpar}
      }
   \end{minipage}
   \caption{Desugaring for terms, function definitions, environments and closures}
   \label{fig:desugar}
\end{figure}

\begin{figure}
   {\flushleft \shadebox{$\mu \desugar \sigma$}
   \hfill}
   \begin{smathpar}
      \inferrule*[
         lab={\ruleName{$\desugar$-fun}}
      ]
      {
         \seq{(p, \clause{\pi}{s})}
         \desugar \sigma
      }
      {
         \seq{\clause{p \cons \pi}{s}}
         \desugar
         \sigma
      }
   \end{smathpar}
   \\[2mm]
   {\flushleft \shadebox{$\seq{k} \desugar \kappa$}
   \hfill}
   \begin{smathpar}
      \inferrule*[
         lab={\ruleName{$\desugar$-clauses-done}}
      ]
      {
         s \desugar e
      }
      {
         (\seqEmpty, \clause{\seqEmpty}{s}) \desugar e
      }
      \and
      \inferrule*[
         lab={\ruleName{$\desugar$-clauses-next-arg}}
      ]
      {
         \seq{(p, \clause{\pi}{s})}
         \desugar
         \sigma
      }
      {
         \seqRange{(\seqEmpty, \clause{p_1 \cons \pi_1}{s_1})}
                  {(\seqEmpty, \clause{p_j \cons \pi_j}{s_j})}
         \desugar
         \exFun{\sigma}
      }
      \and
      \inferrule*[
         lab={\ruleName{$\desugar$-clauses-var}}
      ]
      {
         \seq{k} \desugar \kappa
      }
      {
         \seqRange{(\pattVar{x} \clauseWith{\cons} k_1)}{(\pattVar{x} \clauseWith{\cons} k_j)}
         \desugar
         \elimVar{x}{\kappa}
      }
      \and
      \inferrule*[
         lab={\ruleName{$\desugar$-clauses-record}}
      ]
      {
         (\seqRange{\seq{p_1}}{\seq{p_j}}) \clauseWith{\concat} \seq{k} \desugar \kappa
      }
      {
         (\seqRange{\pattRecord{\seq{\bind{x}{p_1}}}}{\pattRecord{\seq{\bind{x}{p_j}}}})
         \clauseWith{\cons}
         \seq{k}
         \desugar
         \elimRecord{\seq{x}}{\kappa}
      }
      \and
      \inferrule*[
         lab={\ruleName{$\desugar$-clauses-constr}}
      ]
      {
         ((\pi_i \clauseWith{\concat} k_i) \mid c_i = c) \desugar \kappa_c
         \\
         \datatype{c} = D
         \quad
         (\forall c \in \set{\seq{c}})
      }
      {
         \seq{\pattConstr{c}{\pi} \clauseWith{\cons} k}
         \desugar
         \elimConstr{\elimBind{c}{\kappa_c} \mid c \in \set{\seq{c}}}
      }
      \and
      \inferrule*[
         lab={\ruleName{$\desugar$-clauses-non-empty-list}}
      ]
      {
         (\pattConstr{\cCons}{p \cons o} \clauseWith{\cons} k) \cons \seq{k}
         \desugar
         \kappa
      }
      {
         (\pattList{p}{o} \clauseWith{\cons} k)
         \cons
         \seq{k}
         \desugar
         \kappa
      }
      \and
      \inferrule*[
         lab={\ruleName{$\desugar$-list-end}}
      ]
      {
         (\cNil \clauseWith{\cons} k) \cons \seq{k}
         \desugar
         \kappa
      }
      {
         (\pattListEnd \clauseWith{\cons} k)
         \cons
         \seq{k}
         \desugar
         \kappa
      }
      \and
      \inferrule*[
         lab={\ruleName{$\desugar$-list-cons}}
      ]
      {
         (\pattConstr{\cCons}{p \cons o} \clauseWith{\cons} k) \cons \seq{k}
         \desugar
         \kappa
      }
      {
         (\pattListNext{p}{o} \clauseWith{\cons} k)
         \cons
         \seq{k}
         \desugar
         \kappa
      }
   \end{smathpar}
   \caption{Desugaring for function definitions}
   \label{fig:desugar:clauses}
\end{figure}

\begin{figure}
   {\small \flushleft \shadebox{$k, \alpha \orElse \mu$}
   \begin{smathpar}
      \inferrule*[
         lab={\ruleName{$\orElse$-done}}
      ]
      {
         \strut
      }
      {
         (\seqEmpty, \clause{\seqEmpty}{s}), \alpha
         \orElse
         \clause{\seqEmpty}{s}
      }
      \and
      \inferrule*[
         lab={\ruleName{$\orElse$-var}}
      ]
      {
         k, \alpha \orElse \seqRange{k_1}{k_j}
      }
      {
         \pattVar{x} \clauseWith{\cons} k, \alpha
         \orElse
         \seqRange{\pattVar{x} \clauseWith{\cons} k_1}
                  {\pattVar{x} \clauseWith{\cons} k_j}
      }
      \and
      \inferrule*[
         lab={\ruleName{$\orElse$-record}}
      ]
      {
         \seq{p} \clauseWith{\concat} k, \alpha
         \orElse
         \seqRange{\seq{p_1} \clauseWith{\concat} k_1}
                  {\seq{p_j} \clauseWith{\concat} k_j}
      }
      {
         \pattRecord{\seq{\bind{x}{p}}} \clauseWith{\cons} k, \alpha
         \orElse
         \seqRange{\pattRecord{\seq{\bind{x}{p_1}}} \clauseWith{\cons} k_1}
                  {\pattRecord{\seq{\bind{x}{p_j}}} \clauseWith{\cons} k_j}
      }
      \and
      \inferrule*[
         lab={\ruleName{$\orElse$-constr}},
         right={$\ctrsF(D) = c \cons \set{\seq{c}}$}
      ]
      {
         \pi \clauseWith{\concat} k, \alpha
         \orElse
         \seq{\pi \clauseWith{\concat} k}
         \\
         \seq{k}' =
         ((\pattVar{\varAnon} \mid n \numleq \length{\pi'}, \clause{\seqEmpty}{\annot{\exNil}{\alpha}})
         \mid
         i \numleq \length{\seq{c}})
         \\
         k = (\pi', \clause{\seqEmpty}{s})
      }
      {
         \pattConstr{c}{\pi} \clauseWith{\cons} k, \alpha
         \orElse
         (\seqRange{\pattConstr{c}{\pi_1} \clauseWith{\cons} k_1}
                   {\pattConstr{c}{\pi_j} \clauseWith{\cons} k_j})
         \concat
         (\pattConstr{c_i}{\pattVar{\varAnon} \mid n \numleq \arity{c_i}}
         \clauseWith{\cons} k'_i
         \mid i \numleq \length{\seq{c}})
      }
      \and
      \inferrule*[
         lab={\ruleName{$\orElse$-non-empty-list}}
      ]
      {
         p \clauseWith{\cons} o \clauseWith{\cons} k, \alpha
         \orElse
         \seq{p \clauseWith{\cons} o \clauseWith{\cons} k}
         \\
         k = (\pi, \clause{\seqEmpty}{s})
      }
      {
         \pattList{p}{o}
         \clauseWith{\cons} k, \alpha
         \orElse
         \seqRange{\pattList{p_1}{o_1} \clauseWith{\cons} k_1}
                  {\pattList{p_j}{o_j} \clauseWith{\cons} k_j},
         \pattNil \cons \pi, \clause{\seqEmpty}{\annot{\exNil}{\alpha}}
      }
      \and
      \inferrule*[
         lab={\ruleName{$\orElse$-list-end}}
      ]
      {
         k, \alpha \orElse \seq{k}
         \\
         k = (\pi, \clause{\seqEmpty}{s})
      }
      {
         \pattListEnd
         \clauseWith{\cons} k, \alpha
         \orElse
         \seqRange{\pattListEnd \clauseWith{\cons} k_1}
                  {\pattListEnd \clauseWith{\cons} k_j},
         (\pattListNext{\pattVar{\varAnon}}{\pattVar{\varAnon}}) \cons \pi, \clause{\seqEmpty}{\annot{\exNil}{\alpha}}
      }
      \and
      \inferrule*[
         lab={\ruleName{$\orElse$-list-cons}}
      ]
      {
         p \clauseWith{\cons} o \clauseWith{\cons} k, \alpha
         \orElse
         \seq{p \clauseWith{\cons} o \clauseWith{\cons} k}
         \\
         k = (\pi, \clause{\seqEmpty}{s})
      }
      {
         (\pattListNext{p}{o})
         \clauseWith{\cons} k, \alpha
         \orElse
         \seqRange{(\pattListNext{p_1}{o_1}) \clauseWith{\cons} k_1}
                  {(\pattListNext{p_j}{o_j}) \clauseWith{\cons} k_j},
         \pattListEnd \cons \pi, \clause{\seqEmpty}{\annot{\exNil}{\alpha}}
      }
   \end{smathpar}}
   \caption{Completing an (uncurried) clause with a default value of $\exNil$}
\end{figure}

\subsection{Equivalence of Semantics}

Write $\gamma, s\,\evalSugS$ to mean $\exists v.\,\gamma, s \evalSugS v$ and similarly for the other
relations.

\begin{theorem}
   \label{thm:semantics-eq}
   Suppose $s \desugar e$ and $\gamma \desugar \gamma'$.
   \begin{enumerate}
      \item $\gamma, s\,\evalSugS$ iff $\gamma', e\,\evalSugS$.
      \item If $\gamma, s \evalSugS v$ and $\gamma',e \evalSugS v'$ then $v \desugar v'$.
   \end{enumerate}
\end{theorem}
\begin{proof}
   See \appref{proofs:semantics-eq}.
\end{proof}

\thmref{semantics-eq} relies on auxiliary lemmas for pattern-matching (\lemref{match-eq}) and recursive
definitions (\lemref{closedefs-eq}).

\begin{lemma}
   \label{lem:match-eq}
   Suppose $v \desugar v'$ and $\mu \desugar \sigma$.
   \hfill
   \begin{enumerate}
      \item $u, \mu\,\match$ iff $v,\sigma\,\match$.
      \item If $u, \mu \match \gamma', s$ and $v, \sigma \match \gamma, e$ then $\gamma' \desugar \gamma$ and $s \desugar e$.
   \end{enumerate}
\end{lemma}
\begin{proof}
   Immediate from \lemref{match-seq-eq} and definitions of $\desugar$ and $\match$ for $\mu$.
\end{proof}

\begin{lemma}
   \label{lem:match-seq-eq}
   Suppose $\seq{u} \desugar \seq{v}$ and $\seq{k} \desugar \kappa$.
   \hfill
   \begin{enumerate}
      \item $\seq{u}, \seq{k}\,\match$ iff $\seq{v},\kappa\,\match$.
      \item If $\seq{u}, \seq{k} \match \gamma', s$ and $\seq{v}, \kappa \match \gamma, e$ then $\gamma' \desugar \gamma$ and $s \desugar e$.
   \end{enumerate}
\end{lemma}
\begin{proof}
   See \appref{proofs:match-seq-eq}.
\end{proof}

Both $\closeDefs$ relations are total, so \lemref{closedefs-eq} is somewhat simpler.

\begin{lemma}
   \label{lem:closedefs-eq}
   Suppose $\gamma_1 \desugar \gamma_2$ and $\seq{\mu} \desugar \seq{\sigma}$. If $\gamma_1, \seq{\bind{x}{\mu}} \closeDefs \gamma_1'$ and $\gamma_2, \seq{\bind{x}{\sigma}} \closeDefs \gamma_2'$ then $\gamma_1' \desugar \gamma_2'$.
\end{lemma}
\begin{proof}
   See \appref{proofs:close-defs-eq}
\end{proof}

\subsection{Related work}

\begin{itemize}
   \item \citet{pombrio14}
   \item \citet{yang22}
\end{itemize}

\subsection{Backwards desugaring}

\begin{figure}
   {\flushleft \shadebox{$s' \desugarBwd{s} e$}\hfill}
   \begin{smathpar}
      \inferrule*[lab={\ruleName{$\desugarBwd{}$-lambda}}]
      {
         \mu' \desugarBwd{\mu} \sigma
      }
      {
         \exFun{\mu'} \desugarBwd{\exFun{\mu}} \exFun{\sigma}
      }
      \and
      \inferrule*[lab={\ruleName{$\desugarBwd{}$-binary-apply}}]
      {
         s_1' \desugarBwd{s_1} e_1
         \\
         s_2' \desugarBwd{s_2} e_2
      }
      {
         \exBinaryApp{s_1'}{\oplus}{s_2'}
         \desugarBwd{\exBinaryApp{s_1}{\oplus}{s_2}}
         \exForeignApp{\oplus}{e, e'}
      }
      \and
      \inferrule*[lab={\ruleName{$\desugarBwd{}$-let-rec}}]
      {
         \seq{\mu'} \desugarBwd{\seq{\mu}} \seq{\sigma}
         \\
         s' \desugarBwd{s} e
      }
      {
         \exLetRecPiecewise{\seq{\bind{x}{\mu'}}}{s'}
         \desugarBwd{\exLetRecPiecewise{\seq{\bind{x}{\mu}}}{s}}
         \exLetRecPiecewise{\seq{\bind{x}{\sigma}}}{e}
      }
      \and
      \inferrule*[lab={\ruleName{$\desugarBwd{}$-match}}]
      {
         s' \desugarBwd{s} e
         \\
         \mu' \desugarBwd{\mu} \sigma
      }
      {
         \exMatch{s'}{\mu'}
         \desugarBwd{\exMatch{s}{\mu}}
         \exApp{\exFun{\sigma}}{e}
      }
      \and
      \inferrule*[lab={\ruleName{$\desugarBwd{}$-non-empty-list}}]
      {
         s' \desugarBwd{s} e
         \\
         l' \desugarBwd{l} e'
      }
      {
         \exList{s'}{l'}
         \desugarBwd{\exList{s}{l}}
         \exConstr{\cCons}{e, e'}
      }
      \and
      \inferrule*[lab={\ruleName{$\desugarBwd{}$-if}}]
      {
         s' \desugarBwd{s} e
         \\
         s_1' \desugarBwd{s_1} e_1
         \\
         s_2' \desugarBwd{s_2} e_2
         \\
         \sigma = \elimConstr{\elimBind{\cTrue}{e_1}, \elimBind{\cFalse}{e_2}}
      }
      {
         \exIfThenElse{s'}{s_1'}{s_2'}
         \desugarBwd{\exIfThenElse{s'}{s_1'}{s_2'}}
         \exApp{\exFun{\sigma}}{e}
      }
      \and
      \inferrule*[lab={\ruleName{$\desugarBwd{}$-list-enum}}]
      {
         s_1' \desugarBwd{s_1} e
         \\
         s_2' \desugarBwd{s_2} e'
      }
      {
         \exListEnum{s_1'}{s_2'}
         \desugarBwd{\exListEnum{s_1}{s_2}}
         \exApp{\exApp{\varEnumFromTo}{e}}{e'}
      }
      \and
      \inferrule*[lab={\ruleName{$\desugarBwd{}$-list-comp-done}}]
      {
         s' \desugarBwd{s} e
      }
      {
         \exListComp{s'}{\seqEmpty}
         \desugarBwd{\exListComp{s}{\seqEmpty}}
         \exConstr{\cCons}{e, \exNil}
      }
      \and
      \inferrule*[lab={\ruleName{$\desugarBwd{}$-list-comp-guard}}]
      {
         s_1' \desugarBwd{s_1} e
         \\
         \exListComp{s_2'}{\seq{q}'}
         \desugarBwd{\exListComp{s_2}{\seq{q}}}
         e'
         \\
         \sigma = \elimConstr{\elimBind{\cTrue}{e'}, \elimBind{\cFalse}{\exNil}}
      }
      {
         \exListComp{s_2'}{\qualGuard{s_1'} \cons \seq{q}'}
         \desugarBwd{\exListComp{s_2}{\qualGuard{s_1} \cons \seq{q}}}
         \exApp{\exFun{\sigma}}{e}
      }
      \and
      \inferrule*[lab={\ruleName{$\desugarBwd{}$-list-comp-decl}}]
      {
         s_1' \desugarBwd{s_1} e
         \\
         (\clause{p}{\exListComp{s_2'}{\seq{q}'}})
         \desugarBwd{\clause{p}{\exListComp{s_2}{\seq{q}}}}
         \sigma
      }
      {
         \exListComp{s_2'}{\qualDeclaration{p}{s_1'} \cons \seq{q}'}
         \desugarBwd{\exListComp{s_2}{\qualDeclaration{p}{s_1} \cons \seq{q}}}
         \exApp{\exFun{\sigma}}{e}
      }
      \and
      \inferrule*[
         lab={\ruleName{$\desugarBwd{}$-list-comp-gen}}
      ]
      {
         s_1' \desugarBwd{s_1} e
         \\
         \exListComp{s_2'}{\seq{q}'}, \exNil
         \orElseBwd{\clause{p}{\exListComp{s_2}{\seq{q}}}}
         \mu'
         \\
         \mu' \desugarBwd{\mu} \sigma
         \\
         (\clause{p}{\exListComp{s_2}{\seq{q}}}) \orElse \mu
      }
      {
         \exListComp{s_2'}{\qualGenerator{p}{s_1'} \cons \seq{q}'}
         \desugarBwd{\exListComp{s_2}{\qualGenerator{p}{s_1} \cons \seq{q}}}
         \exApp{\exApp{\varConcatMap}{\exFun{\sigma}}}{e}
      }
   \end{smathpar}
   \\[2mm]
   {\flushleft \shadebox{$l' \desugarBwd{l} e$}
   \hfill}
   \begin{smathpar}
      \inferrule*[lab={\ruleName{$\desugarBwd{}$-list-rest-nil}}]
      {
         \strut
      }
      {
         \exListEnd
         \desugarBwd{\exListEnd}
         \exListEnd,
         \exNil
      }
      \and
      \inferrule*[lab={\ruleName{$\desugarBwd{}$-list-rest-cons}}]
      {
         s' \desugarBwd{s} e
         \\
         l' \desugarBwd{l} e'
      }
      {
         (\exListNext{s'}{l'})
         \desugarBwd{\exListNext{s}{l}}
         \exConstr{\cCons}{e, e'}
      }
   \end{smathpar}
   \caption{Desugaring for terms and function definitions (backwards rules)}
   \label{fig:desugar}
\end{figure}

\begin{figure}
   {\flushleft \shadebox{$\mu' \desugarBwd{\mu} \sigma$}
   \hfill}
   \begin{smathpar}
      \inferrule*[
         lab={\ruleName{$\desugar$-fun}}
      ]
      {
         \seq{(p, \clause{\pi}{s'})}
         \desugarBwd{\seq{(p, \clause{\pi}{s})}}
         \sigma
      }
      {
         \seq{\clause{p \cons \pi}{s'}}
         \desugarBwd{\seq{\clause{p \cons \pi}{s}}}
         \sigma
      }
   \end{smathpar}
   \\[2mm]
   {\flushleft \shadebox{$\seq{k} \desugarBwd{\seq{k}} \kappa$}
   \hfill}
   \begin{smathpar}
      \inferrule*[
         lab={\ruleName{$\desugarBwd{}$-clauses-done}}
      ]
      {
         s' \desugarBwd{s} e
      }
      {
         (\seqEmpty, \clause{\seqEmpty}{s'}) \desugarBwd{(\seqEmpty, \clause{\seqEmpty}{s})} e
      }
      \and
      \inferrule*[
         lab={\ruleName{$\desugarBwd{}$-clauses-next-arg}}
      ]
      {
         \seq{(p', \clause{\pi'}{s'})}
         \desugarBwd{\seq{(p, \clause{\pi}{s})}}
         \sigma
      }
      {
         \seqRange{(\seqEmpty, \clause{p'_1 \cons \pi'_1}{s'_1})}
                  {(\seqEmpty, \clause{p'_{j'} \cons \pi'_{j'}}{s'_{j'}})}
         \desugarBwd{
            \seqRange{(\seqEmpty, \clause{p_1 \cons \pi_1}{s_1})}
                     {(\seqEmpty, \clause{p_j \cons \pi_j}{s_j})}
         }
         \exFun{\sigma}
      }
      \and
      \inferrule*[
         lab={\ruleName{$\desugarBwd{}$-clauses-var}}
      ]
      {
         \seq{k'} \desugarBwd{\seq{k}} \kappa
      }
      {
         \seqRange{(\pattVar{x} \clauseWith{\cons} k'_1)}{(\pattVar{x} \clauseWith{\cons} k'_j)}
         \desugarBwd{\seqRange{(\pattVar{x} \clauseWith{\cons} k_1)}{(\pattVar{x} \clauseWith{\cons} k_j)}}
         \elimVar{x}{\kappa}
      }
      \and
      \inferrule*[
         lab={\ruleName{$\desugarBwd{}$-clauses-record}}
      ]
      {
         (\seqRange{\seq{p'_1}}{\seq{p'_{j'}}}) \clauseWith{\concat} \seq{k'}
         \desugarBwd{(\seqRange{\seq{p_1}}{\seq{p_j}}) \clauseWith{\concat} \seq{k}}
         \kappa
      }
      {
         (\seqRange{\pattRecord{\seq{\bind{x}{p'_1}}}}{\pattRecord{\seq{\bind{x}{p'_{j'}}}}})
         \clauseWith{\cons}
         \seq{k'}
         \desugarBwd{
            (\seqRange{\pattRecord{\seq{\bind{x}{p_1}}}}{\pattRecord{\seq{\bind{x}{p_j}}}})
            \clauseWith{\cons}
            \seq{k}
         }
         \elimRecord{\seq{x}}{\kappa}
      }
      \and
      \inferrule*[
         lab={\ruleName{$\desugarBwd{}$-clauses-constr}}
      ]
      {
         ((\pi'_i \clauseWith{\concat} k'_i) \mid c_i = c)
         \desugarBwd{((\pi_i \clauseWith{\concat} k_i) \mid c_i = c)}
         \kappa_c
         \\
         (\forall c \in \set{\seq{c'}})
      }
      {
         \seq{\pattConstr{c'}{\pi'} \clauseWith{\cons} k'}
         \desugarBwd{\seq{\pattConstr{c}{\pi} \clauseWith{\cons} k}}
         \elimConstr{\seq{\elimBind{c'}{\kappa}}}
      }
   \end{smathpar}
   \caption{Desugaring for function definitions (backwards rules)}
   \label{fig:desugar:clauses:bwd}
\end{figure}

\begin{figure}
   {\small \flushleft \shadebox{$s, \alpha \orElseBwd{k} \mu$}
   \begin{smathpar}
      \inferrule*[
         lab={\ruleName{$\orElseBwd{}$-done}}
      ]
      {
         \strut
      }
      {
         s', \bot
         \orElseBwd{(\seqEmpty, \clause{\seqEmpty}{s})}
         \clause{\seqEmpty}{s'}
      }
      \and
      \inferrule*[
         lab={\ruleName{$\orElseBwd{}$-var}}
      ]
      {
         s, \alpha \orElseBwd{k} \seqRange{k'_1}{k'_j}
      }
      {
         s, \alpha
         \orElseBwd{\pattVar{x} \clauseWith{\cons} k}
         \seqRange{\pattVar{x} \clauseWith{\cons} k'_1}
                  {\pattVar{x} \clauseWith{\cons} k'_j}
      }
      \and
      \inferrule*[
         lab={\ruleName{$\orElseBwd{}$-record}}
      ]
      {
         s, \alpha
         \orElseBwd{\seq{p} \clauseWith{\concat} k}
         \seqRange{\seq{p_1} \clauseWith{\concat} k'_1}
                  {\seq{p_j} \clauseWith{\concat} k'_j}
      }
      {
         s, \alpha
         \orElseBwd{\pattRecord{\seq{\bind{x}{p}}} \clauseWith{\cons} k}
         \seqRange{\pattRecord{\seq{\bind{x}{p_1}}} \clauseWith{\cons} k'_1}
                  {\pattRecord{\seq{\bind{x}{p_j}}} \clauseWith{\cons} k'_j}
      }
      \and
      \inferrule*[
         lab={\ruleName{$\orElseBwd{}$-constr}}
      ]
      {
         s, \beta
         \orElseBwd{\pi \clauseWith{\concat} k}
         \seq{\pi \clauseWith{\concat} k'}
         \\
         k^\twoPrime_i =
         \clause{(\pattVar{\varAnon} \mid n \numleq \length{\pi'})}{\alpha_i}
         \quad
         (\forall i \numleq \length{\seq{c}})
         \\
         \ctrsF(D) \supseteq c \cons \set{\seq{c}}
      }
      {
         s, \bigjoin\set{\seq{\alpha}} \join \beta
         \orElseBwd{\pattConstr{c}{\pi} \clauseWith{\cons} k}
         (\seqRange{\pattConstr{c}{\pi_1} \clauseWith{\cons} k'_1}
                   {\pattConstr{c}{\pi_j} \clauseWith{\cons} k'_j})
         \concat
         (\pattConstr{c_i}{\pattVar{\varAnon} \mid n \numleq \arity{c_i}}
         \clauseWith{\cons} k^\twoPrime_i
         \mid i \numleq \length{\seq{c}})
      }
      \and
      \inferrule*[
         lab={\ruleName{$\orElseBwd{}$-non-empty-list}}
      ]
      {
         s, \alpha
         \orElseBwd{p \clauseWith{\cons} o \clauseWith{\cons} k}
         \seq{p' \clauseWith{\cons} o' \clauseWith{\cons} k'}
      }
      {
         s, \alpha
         \orElseBwd{\pattList{p}{o} \clauseWith{\cons} k}
         \seqRange{\pattList{p'_1}{o'_1} \clauseWith{\cons} k'_1}
                  {\pattList{p'_j}{o'_j} \clauseWith{\cons} k'_j},
         k^\twoPrime
      }
      \and
      \inferrule*[
         lab={\ruleName{$\orElseBwd{}$-list-end}}
      ]
      {
         s, \alpha \orElseBwd{k} \seq{k}'
      }
      {
         s, \alpha
         \orElseBwd{\pattListEnd \clauseWith{\cons} k}
         \seqRange{\pattListEnd \clauseWith{\cons} k'_1}
                  {\pattListEnd \clauseWith{\cons} k'_j},
         k^\twoPrime
      }
      \and
      \inferrule*[
         lab={\ruleName{$\orElseBwd{}$-list-cons}}
      ]
      {
         s, \alpha
         \orElseBwd{p \clauseWith{\cons} o \clauseWith{\cons} k}
         \seq{p' \clauseWith{\cons} o' \clauseWith{\cons} k'}
      }
      {
         s, \alpha
         \orElseBwd{(\pattListNext{p}{o}) \clauseWith{\cons} k}
         \seqRange{(\pattListNext{p'_1}{o'_1}) \clauseWith{\cons} k'_1}
                  {(\pattListNext{p'_j}{o'_j}) \clauseWith{\cons} k'_j},
         k^\twoPrime
      }
   \end{smathpar}}
   \caption{Completing an (uncurried) clause with a default value of $\exNil$ (backwards rules)}
\end{figure}
