# Supplementary material for: Cognacy Queries over Dependence Graphs for Transparent Visualisations
Source: arXiv:2403.04403 source file (2024-10-15)
Supplement: Supplementary file 5 [file inductive-graphs.tex]

\section{Inductive Definition of Graphs}

\subsection{Graph Syntax}
Graphs are defined by the syntax given in \figref{graph-syntax}.

\begin{figure}[h]
   {\small
   \begin{minipage}[t]{0.48\textwidth}
      \begin{tabularx}{\textwidth}{rL{2.8cm}L{3cm}}
         &\textbfit{Inductive Graphs}&
         \\
         $G ::=$
         &
         $\set{\seq{G \mapsto \alpha}}$
         &
         collection of rooted direted graphs
         \\
      \end{tabularx}
   \end{minipage}
   }
   \caption{Syntax of Graphs}
   \label{fig:graph-syntax}
\end{figure}

% We need some auxiliary functions to go with the new syntax:
% \begin{definition}[Vertices]
%    For a graph $G$, we define the set $\opName{V}(G)$ to be the vertices of $G$,
%    and define it as:
%    \begin{salign}
%       \opName{V}((G \mapsto \alpha) \cdot \set{\seq{H}}) &= {\alpha} \cup \opName{V}(\set{\seq{H}})\\
%       \opName{V}(\emptyset) &= \emptyset\\
%    \end{salign}
% \end{definition}

% To find the leaves of a graph, we use a specified version of the vertices function.
% \begin{definition}[Leaves]
%    For a graph $G$, write  $\opName{Leaves}(G)$ to be the 
%    set of leaves in $G$, and define it as:
%    \begin{salign}
%       \opName{Leaves}((\emptyset \mapsto \alpha) \cdot \set{\seq{H}}) &= \set{\alpha} \cup \opName{Leaves}(\set{\seq{H}}) \\
%       \opName{Leaves}((G \mapsto \alpha) \cdot \set{\seq{H}}) &= \opName{Leaves}(\set{\seq{H}}) \\
%       \opName{Leaves}(\emptyset) &= \emptyset \\
%    \end{salign}
% \end{definition}

We can consider a graph $G$ to be a finite
map from vertices to subgraphs. For a vertex $\alpha$ if $\alpha \in \opName{V}(G)$
then $\exists G'$ such that $G = \set{\alpha \mapsto G'} \cup \set{\seq{H}}$, write $G(\alpha) = (\alpha \mapsto G')$ for
the subgraph of $G$ rooted at $\alpha$.
% \begin{definition}[Roots]
%    For a graph $G$, we write $\opName{Roots}(G)$ for the set
%    of \textit{root nodes} in $G$, and define it as:
%    \begin{salign}
%       \opName{Roots}(\exForest{\set{\seq{G}}}) &= \bigcup_{G \in \set{\seq{G}}} \opName{Roots}(G) \\
%       \opName{Roots}(\exStar{F}{\alpha}) &= \set{\alpha} \\
%    \end{salign}
% \end{definition}

% \begin{definition}[Recursive Lookup]
%    For a graph $G$, and a vertex $\alpha$, we write $\opName{F}(\alpha, G)$ for
%    the graph of ancestors of $\alpha$, and define it as:
%    \begin{salign}
%       \opName{F}(\alpha, \exForest{\set{\seq{G}}}) &= \exForest{\bigcup_{G' \in \set{\seq{G}}} \opName{F}(\alpha, G)} \\
%       \opName{F}(\alpha, \exStar{F}{\alpha}) &= \exStar{(\exForest{\bigcup_{G' \in F} \opName{F}(\opName{Roots}(G'), G')})}{\alpha} \\
%       \opName{F}(\alpha, \exStar{F}{\alpha'}) &= \emptyset \\
%    \end{salign}
% \end{definition}

\begin{figure}
   \begin{subfigure}{\textwidth}
   {\small \flushleft \shadebox{$\gamma, e, G, G_{1} \evalS v, G_{2}$}
      \begin{smathpar}
      \inferrule*[
         lab={\ruleName{$\evalS$-var}},
         right={$\gamma = \gamma' \cons \bind{x}{v}$}
      ]
      {
         \strut
      }
      {
         \gamma, x, G, G_{1} \evalS v, G_{1} 
      }
      \and
      \inferrule*[
         lab={\ruleName{$\evalS$-int}},
         right={$\alpha \notin \dom{G_{1}}$},
      ]
      {
         \strut
      }
      {
         \gamma, n, G, G_{1} \evalS n_{\alpha \mapsto G}, G_{1} \cdot \set{\alpha \mapsto G}
      }
      \and
      \inferrule*[
         lab={\ruleName{$\evalS$-function}},
         right={$\alpha \notin \dom{G_{1}}$},
      ]
      {
         \strut
      }
      {
         \gamma, \exFun{\sigma}, G, G_{1} \evalS \exClosure{\gamma}{\emptyset}{\sigma}_{\alpha \mapsto G}, G_{1} \cdot \set{\alpha \mapsto G}
      }
      \and
      \inferrule*[
         lab={\ruleName{$\evalS$-record}},
         right={$\alpha \notin \dom{G_{2}}$},
      ]
      {
         \gamma, \seq{e}, G, G_{1} \evalS \seq{v}, G_{2}
      }
      {
         \gamma, \exRecord{\seq{\bind{x}{e}}}, G, G_{1} \evalS \exRecord{\seq{\bind{x}{v}}}_{\alpha}, G_{2} \cdot (\alpha \mapsto G)
      }
      \and
      \inferrule*[
         lab={\ruleName{$\evalS$-constr}},
         right={$\Sigma(c) = |\seq{e}|, \alpha \notin \dom{G_{2}}$}
      ]
      {
         \gamma, \seq{e}, G, G_{1} \evalS \seq{v}, G_{2}
      }
      {
         \gamma, \exConstr{c}{\seq{e}}, G, G_{1} \evalS \exConstr{c}{\seq{v}}_{\alpha \mapsto G}, G_{2} \cdot \set{\alpha \mapsto G}
      }
      \and
      \inferrule*[
         lab={\ruleName{$\evalS$-foreign-app}}
      ]
      {
         \gamma, \seq{e}, G, G_{1} \evalS \seq{v}, G_{2}
         \\
         \hat{f}(\seq{v}) = \exPair{u}{G_{3}}
      }
      {
         \gamma, f(\seq{e}), G, G_{1} \evalS u, G_{3}
      }
      \and
      \inferrule*[
         lab={\ruleName{$\evalS$-let}}
      ]
      {
         \gamma, e, G, G_{1} \evalS v, G_{2}
         \\
         \gamma\cdot(\bind{x}{v}), e', G, G_{2} \evalS v', G_{3}
      }
      {
         \gamma, \exLet{x}{e}{e'}, G, G_{1} \evalS v', G_{3}
      }
      \and
      \inferrule*[
         lab={\ruleName{$\evalS$-let-rec}}
      ]
      {
         \gamma, \exRecord{\seq{\bind{x}{\sigma}}}, G_{1} \closeDefs \gamma', G_{2}
         \\
         \gamma \concat \gamma', e, G, G_{2} \evalS v, G_{3}
      }
      {
         \gamma, \exLetRec{\seq{\bind{x}{\sigma}}}{e}, G, G_{1} \evalS v, G_{3} 
      }
      \and
      \inferrule*[
         lab={\ruleName{$\evalS$-app}},
         width=4in,
         right={$\alpha \notin \dom{G_{4}}$},
      ]
      {
         \gamma, e, G, G_{1} \evalS \exClosure{\gamma_{1}}{\rho}{\sigma}_{\alpha \mapsto G}, G_{2}
         \\
         \gamma_{1}, \rho, G_{2} \closeDefs \gamma_2, G_{3}
         \\
         \gamma, e', G, G_{3} \evalS v', G_{4}
         \\
         v', \sigma \match \gamma_{3}, e'', G_{5}
         \\
         \gamma_{1} \concat \gamma_{2} \concat \gamma_{3}, e'', G_{4}\cdot\set{\alpha \mapsto G} \evalS u, G_{6}
      }
      {
         \gamma, \exApp{e}{e'}, G, G_{1} \evalS u, G_{6}
      }
      \end{smathpar}
   }
   \end{subfigure}
   \\[3mm]
   \begin{subfigure}{\textwidth}
   {\small \flushleft \shadebox{$\gamma, \seq{e}, G, G_{1} \evalS \seq{v}, G_{2}$}
   \begin{smathpar}
      \inferrule*[
         lab={\ruleName{$\evalS$-seq}},
         right={$n = |\seq{e}|$}
      ]
      {
         \gamma, e_i, G, G_{i-1} \evalS v_i, G_i
         \quad
         (\forall i. 1 \leq i \leq |\seq{e}|)
      }
      {
         \gamma, \seq{e}, G, G_{0} \evalS \seq{v}, G_{n}
      }
   \end{smathpar}
   }
   \end{subfigure}
   \caption{Graph Evaluation}
\end{figure}

\begin{figure}
   {\small \flushleft \shadebox{$\seq{v}, \kappa, \match \gamma, \kappa', G$}
   \begin{smathpar}
      \inferrule*[
         lab={\ruleName{$\match$-done}}
      ]
      {
         \strut
      }
      {
         \epsilon, e, \match \emptyset, e, \emptyset
      }
      \and
      \inferrule*[
         lab={\ruleName{$\match$-var}}
      ]
      {
         \seq{v}, \kappa \match \gamma, \tau, G_{1}
      }
      {
         v \cdot \seq{v}, x \mapsto \kappa \match \gamma \cdot (\bind{x}{v}), \tau, G_{1}
      }
      \and
      \inferrule*[
         lab={\ruleName{$\match$-constr}}
      ]
      {
         \seq{v} \concat \seq{v}', \kappa \match \gamma, e, G_{1}
      }
      {
         \exConstr{c}{\seq{v}}_{\alpha \mapsto G} \cdot \seq{v}', (c \mapsto \kappa) \cdot\set{\seq{c \mapsto \kappa}} \match \gamma, e, G_{1} \cup \set{\alpha \mapsto G}
      }
      \and
      \inferrule*[
         lab={\ruleName{$\match$-record}}
      ]
      {
         \set{\seq{\bind{y}{u}}} \subseteq \set{\seq{\bind{x}{v}}}
         \\
         \seq{u} \concat \seq{v}', \kappa \match \gamma, e, G_{1}
      }
      {
         \set{\seq{\bind{x}{v}}}_{\alpha \mapsto G} \cdot \seq{v}', \set{\seq{y}} \mapsto \kappa \match \gamma, e, G_{1} \cup \set{\alpha \mapsto G}
      }
   \end{smathpar}
   }
   \caption{Pattern Match}
\end{figure}
\begin{figure}
   {\small \flushleft \shadebox{$\gamma, \rho, G \closeDefs \gamma', G'$} 
      \begin{smathpar}
         \inferrule*[]
         {
            v_{i} = \exClosure{\gamma}{\rho}{\rho(x_i)}_{\alpha_{i} \mapsto G'}
         }
         {
            \gamma,\rho, G \closeDefs \set{\seq{\bind{x}{v}}}, \set{\alpha_{i} \mapsto G' \mid 1 \leq i \leq |\seq{e}|}
         }
      \end{smathpar}
   }
\end{figure}
% \subsection*{Demands and Demanded By}

% \begin{definition}[Demands]
%    For a graph $G$, with some subset of root nodes $\set{\seq{\alpha}}$, we write
%    $\demandsR_G(\set{\seq{\alpha}})$ for the set of leaf nodes which can reach 
%    a member of the set $\set{\seq{\alpha}}$, and define it as:
%    $$
%       \demandsR_{G}(\set{\seq{\alpha}}) \eqdef \opName{Leaves}(\bigcup_{\alpha \in \set{\seq{\alpha}}} \opName{F}(\alpha, G))
%    $$
% \end{definition}

% We can write the above as a judgement as follows:
% \input{appendix/fig/graphs/demands-inductive}
