# Supplementary material for: Cognacy Queries over Dependence Graphs for Transparent Visualisations
Source: arXiv:2403.04403 source file (2024-10-15)
Supplement: Supplementary file 6 [file surface.tex]

\section{Surface Language}

We give a direct semantics for the surface language in \figref{surface:eval} and the corresponding notion of
surface value. (Surface values differ from core values only in the case of closures, which contain surface
expressions and other surface values.) We prove that directly evaluating a surface program $s$ and desugaring
the resulting value is equivalent to desugaring $s$ to a core program and then evaluating it in the core
semantics.

\begin{lemma}[Determinism]
   \label{lem:surface:eval:determinism}
   If $\gamma, s \evalS v$ and $\gamma, s \evalS v'$ then $v = v'$.
\end{lemma}

\subsubsection{Mutual recursion}

The following relation determines the closures associated with a block of mutually recursive functions $g =
\seq{\bind{x}{\mu}}$. (Read $x$ as the function name and $\mu$ as the defining clauses of the function.)

\begin{definition}[Close defs]
   \label{def:surface:close-defs}
   \figref{surface:eval} defines the \emph{close defs} relation $\closeDefs$.
\end{definition}

\subsubsection{Piecewise function definitions}

We disallow certain combinations of patterns which are commonly allowed in other languages, such as:%
{\small
\begin{lstlisting}[language=Fluid]
   foo (Cons y ys) (Cons z zs) = ...
   foo  x           Nil        = ...

   bar x ... = ...
   bar y ... = ...
\end{lstlisting}}

\noindent In particular, ``aligned'' variable patterns must have the same name, and variable patterns and any other kind of pattern may only be aligned if we have already been able to distinguish the clauses they are part of. Thus the following is allowed:%
{\small
\begin{lstlisting}[language = Fluid]
   baz (Cons y ys)  x = ...
   baz  Nil         x = ...
\end{lstlisting}}

Let $k$ range over $(\pi, \clause{\pi'}{s})$ pairs. The first component $\pi$ is a stack of subpatterns active
during the processing of a single top-level pattern $p$, initially containing only $p$ and ending up empty.
The second component $\clause{\pi'}{s}$ stores the remaining top-level patterns, and is non-empty only for
curried functions. The following notation is useful for processing piecewise function definitions:

\begin{definition}
   Suppose $k = (\pi, \clause{\pi'}{s})$.
   \begin{enumerate}
      \item Define $p \clauseWith{\cons} k \eqdef (p \cons \pi, \clause{\pi'}{s})$.
      \item Define $\pi^\dagger \clauseWith{\concat} k \eqdef (\pi^\dagger \concat \pi, \clause{\pi'}{s})$.
   \end{enumerate}
   Extend the notation to same-length sequences, so that for example $\seq{p} \clauseWith{\cons} \seq{k} = \seq{p \clauseWith{\cons} k}$.
\end{definition}

\begin{figure}
   {\small
   \begin{minipage}[t]{0.48\textwidth}
   \begin{tabularx}{\textwidth}{rL{2.8cm}L{3cm}}
      &\textbfit{Surface term}&
      \lowlight{$\SExpr\;\Gamma\;A$}
      \\
      $s ::=$
      &
      $\exBinaryApp{s}{\oplus}{s'}$
      &
      binary application
      \\
      &
      $\exLetRecPiecewise{g}{s}$
      &
      recursive functions
      \\
      &
      $\exIfThenElse{s}{s_1}{s_2}$
      &
      if
      \\
      &
      $\exMatch{s}{\seq{\clauseUncurried{p}{s}}'}$
      &
      match
      \\
      &
      $\exList{s}{l}$
      &
      non-empty list
      \\
      &
      $\exListEnum{s}{s'}$
      &
      list enum
      \\
      &
      $\exListComp{s}{\seq{q}}$
      &
      list comprehension
      \\
      &
      $\exDo{\seq{d}}$
      &
      do
      \\
      &
      $\exFun{\mu}$
      &
      lambda
      \\[2mm]
      &\textbfit{List rest}&
      \lowlight{$\ListRest\;\Gamma\;A$}
      \\
      $l ::=$
      &
      $\exListEnd$
      &
      end
      \\
      &
      $\exListNext{s}{l}$
      &
      cons
      \\[2mm]
      &\textbfit{Recursive functions}&
      \\
      $g ::=$
      &
      $\seq{\bind{x}{\mu}}$
      &
      \\[2mm]
      &\textbfit{Function definition}&
      \\
      $\mu ::=$
      &
      $\seq{\clause{\pi}{s}}$
      &
      \\[8mm]
      \end{tabularx}
   \end{minipage}%
   \begin{minipage}[t]{0.5\textwidth}
      \begin{tabularx}{\textwidth}{rL{2.8cm}L{2.9cm}}
      &\textbfit{Pattern sequence}&
      \\
      $\pi ::=$
      &
      $\seq{p}$
      &
      \\[2mm]
      &\textbfit{Pattern}&
      \lowlight{$\Patt\;A\;\Gamma$}
      \\
      $p ::=$
      &
      $\pattVar{x}$
      &
      variable
      \\
      &
      $\pattRecord{\seq{\bind{x}{p}}}$
      &
      record
      \\
      &
      $\pattConstr{c}{\pi}$
      &
      constructor
      \\
      &
      $\pattList{p}{o}$
      &
      non-empty list
      \\[2mm]
      &\textbfit{List rest pattern}&
      \lowlight{$\ListRestPatt\;A\;\Gamma$}
      \\
      $o ::=$
      &
      $\pattListEnd$
      &
      end
      \\
      &
      $\pattListNext{p}{o}$
      &
      cons
      \\[2mm]
      &\textbfit{Qualifier}&
      \\
      $q ::=$
      &
      $\qualGuard{s}$
      &
      guard
      \\
      &
      $\qualDeclaration{p}{s}$
      &
      declaration
      \\
      &
      $\qualGenerator{p}{s}$
      &
      generator
      \\[2mm]
      &\textbfit{Surface value}&
      \lowlight{$\SVal{A}$}
      \\
      $v, u ::=$
      &
      $\dots$
      &
      $\dots$
      \\
      &
      $\exClosure{\gamma}{g}{\mu}$
      &
      closure
      \\[8mm]
      \end{tabularx}
   \end{minipage}
   }
   \caption{Syntax of surface terms}
\end{figure}

\begin{figure}
   {\small \flushleft \shadebox{$\gamma, \seq{s} \evalSugR{\seq{S}} \seq{v}$}%
   \begin{smathpar}
      \inferrule*[
         lab={\ruleName{$\evalSugS$-seq}}
      ]
      {
         \gamma, s_i \evalSugR{S_i} v_i
         \quad
         (\forall i \numleq \length{\seq{s}})
      }
      {
         \gamma, \seq{s} \evalSugR{\seq{S}} \seq{v}
      }
      \and
   \end{smathpar}}
   {\small \flushleft \shadebox{$\gamma, s \evalSugR{S} v$}%
   \begin{smathpar}
      \inferrule*[lab={\ruleName{$\evalSugS$-nonempty-list}}]
      {
         \gamma, s \evalSugR{S} v
         \\
         \gamma, l \evalSugR{S'} v'
      }
      {
         \gamma, \exList{s}{l} \evalSugR{\trList{S}{S'}} \cCons(v, v')
      }
      \and
      \inferrule*[lab={\ruleName{$\evalSugS$-list-comp-done}}]
      {
         \gamma, s \evalSugR{S} u
      }
      {
         \gamma, \exListComp{s}{\seqEmpty} \evalSugR{\seqEmpty, S} \exConstr{\cCons}{u, \exNil}
      }
      \and
      \inferrule*[
         lab={\ruleName{$\evalSugS$-list-comp-decl}}
      ]
      {
         \gamma, s' \evalSugR{S'} u'
         \\
         u', (\clause{p}{\exListComp{s}{\seq{q}}})\match \gamma', s^\dag
         \\
         (\gamma \concat \gamma'), s^\dag \evalSugR{\seq{Q},S} u
      }
      {
         \gamma, \exListComp{s}{\qualDeclaration{p}{s'} \cons \seq{q}} \evalSugR{\trQualDecl{p}{S'} \cons \seq{Q}, S} u
      }
      \and
      \inferrule*[
         lab={\ruleName{$\evalSugS$-list-comp-gen}}
      ]
      {
         (\clause{p}{\exListComp{s'}{\seq{q}}}), \exNil \orElse \mu
         \\
         \gamma, \exApp{\exApp{\varConcatMap}{\exFun{\mu}}}{s} \evalSugS u
      }
      {
         \gamma, \exListComp{s'}{\qualGenerator{p}{s} \cons \seq{q}}
         \evalSugR{\trQualGen{p}{S'}\cons\seq{Q}, S}
         u
      }
      \and
      \inferrule*[
         lab={\ruleName{$\evalSugS$-list-comp-guard-false}}
      ]
      {
         \gamma, s \evalSugR{S} \cFalse
      }
      {
         \gamma, \exListComp{s'}{\qualGuard{s} \cons \seq{q}} \evalSugR{\trQualIfFalse{S}{q}} \exNil
      }
      \and
      \inferrule*[
         lab={\ruleName{$\evalSugS$-list-comp-guard-true}},
      ]
      {
         \gamma, \exListComp{s'}{\seq{q}} \evalSugR{\seq{Q},S} v
         \\
         \gamma, s \evalSugR{S} \cTrue
      }
      {
         \gamma, \exListComp{s'}{\qualGuard{s} \cons \seq{q}} \evalSugR{\trQualIfTrue{S} \cons \seq{Q}, S} v
      }
      \and
      \inferrule*[
         lab={\ruleName{$\evalSugS$-app}},
         width=3in,
      ]
      {
         \gamma, s \evalSugR{S} \exClosure{\gamma_1}{g}{\mu}
         \\
         \gamma, s' \evalSugR{S'} v
         \\
         \gamma_1, g \closeDefs \gamma_2
         \\
         v, \mu \match \gamma_3, s^\dag
         \\
         \gamma_1 \concat \gamma_2 \concat \gamma_3, s^\dag \evalSugR{S^\dag} v'
      }
      {
         \gamma, \exApp{s}{s'} \evalSugR{\trApp{S}{S'}{p}{S^{\dag}}} v'
      }
      \and
      \inferrule*[
         lab={\ruleName{$\evalSugS$-bin-app}}
      ]
      {
         \gamma, s_1 \evalSugR{S_1} u_1
         \\
         \gamma, s_2 \evalSugR{S_2} u_2
         \\
         \gamma, \hat{\oplus}(u_1, u_2) = u
      }
      {
         \gamma, s_1 \oplus s_1 \evalSugR{\trBinApp{S_1}{S_2}{t}} u
      }
      \and
      \inferrule*[
         lab={\ruleName{$\evalSugS$-if-true}}
      ]
      {
         \gamma, s \evalSugR{S} \cTrue
         \\
         \gamma, s_1 \evalSugR{S_1} u
      }
      {
         \gamma, \exIfThenElse{s}{s_1}{s_2}\evalSugR{\exIfThenElse{S}{S_1}{s_2}} u
      }
      \and
      \inferrule*[
         lab={\ruleName{$\evalSugS$-if-false}}
      ]
      {
         \gamma, s \evalSugR{S} \cFalse
         \\
         \gamma, s_2 \evalSugR{S_2} u
      }
      {
         \gamma, \exIfThenElse{s}{s_{1}}{s_{2}}\evalSugR{\exIfThenElse{S}{s_1}{S2}} u
      }
      \and
      \inferrule*[
         lab={\ruleName{$\evalSugS$-let-rec}}
      ]
      {
         \gamma, g \closeDefs \gamma'
         \\
         \gamma \concat \gamma', s \evalSugR{S} v
      }
      {
         \gamma, \exLetRecPiecewise{g}{s} \evalSugR{\trLetRec{g}{S}} v
      }
      \and
      \inferrule*[
         lab={\ruleName{$\evalSugS$-match-as}}
      ]
      {
         \gamma, s \evalSugR{S} v
         \\
         v, \seq{\clauseUncurried{p}{s}}' \match \gamma', s_i
         \\
         \gamma \concat \gamma', s_i \evalSugR{S'} v'
      }
      {
         \gamma, \exMatch{s}{\seq{\clauseUncurried{p}{s}}'} \evalSugR{\trMatchAs{S}{\clauseUncurried{p'}{S'}}} v'
      }
      \and
      \inferrule*[
         lab={\ruleName{$\evalSugS$-enum}}
      ]
      {
         \gamma, \exApp{\exApp{\varEnumFromTo}{s_1}}{s_2} \evalSugR{\trSurfaceApp{(\trSurfaceApp{\varEnumFromTo}{S_1}{\exClosure{\varepsilon}{\varepsilon}{\clause{y}{S'}}})}{S_2}{S^{\dag}}} v
      }
      {
         \gamma, \exListEnum{s_1}{s_2} \evalSugR{\trEnum{S_1}{S_2}} v
      }
   \end{smathpar}}
   \\[3mm]
   {\small \flushleft \shadebox{$\gamma, r \evalSugS v$}
   \begin{smathpar}
      \inferrule*[
         lab={\ruleName{$\evalSugS$-list-rest-nil}}
      ]
      {
         \strut
      }
      {
         \gamma, \exListEnd \evalSugR{\trListEnd} \exNil
      }
      \and
      \inferrule*[
         lab={\ruleName{$\evalSugS$-list-rest-next}}
      ]
      {
         \gamma, s \evalSugR{S} v
         \\
         \gamma, l \evalSugR{S'} v'
      }
      {
         \gamma, (\exListNext{s}{l}) \evalSugR{\trListNext{S}{S'}} \exConstr{\cCons}{v, v'}
      }
   \end{smathpar}
   }
   \\[2mm]
   {\small\flushleft \shadebox{$\gamma, g \closeDefs \gamma'$}
      \begin{smathpar}
         \inferrule*[
%            lab={\ruleName{$\closeDefs$-surface}}
         ]
         {
            g = \seq{\bind{x}{\mu}}
            \\
            v_i = \exClosure{\gamma}{g}{\mu_i}
            \quad
            (\forall i \le \length{\seq{x}})
         }
         {
            \gamma, g \closeDefs \set{\seq{\bind{x}{v}}}
         }
      \end{smathpar}}
   \caption{Surface semantics}
   \label{fig:surface:eval}
\end{figure}

\begin{figure}
   {\small \flushleft \shadebox{$v, \mu \match \gamma, s$}
   \begin{smathpar}
      \inferrule*[
         lab={\ruleName{$\match$-fun}}
      ]
      {
         v, \seq{(p, \clause{\pi}{s})} \match \gamma, s
      }
      {
         v, (\seq{\clause{p \cons \pi}{s}})
         \match
         \gamma, s
      }
   \end{smathpar}}
   \\[3mm]
   {\small \flushleft \shadebox{$\seq{v}, \seq{k} \match \gamma, s$}
   \begin{smathpar}
      \inferrule*[
         lab={\ruleName{$\match$-done-uncurried}}
      ]
      {
         \strut
      }
      {
         \seqEmpty, (\seqEmpty, \clause{\seqEmpty}{s}) \match \envEmpty, s
      }
      \and
      \inferrule*[
         lab={\ruleName{$\match$-done-curried}}
      ]
      {
         \strut
      }
      {
         \seqEmpty,
         \seqRange{(\seqEmpty, \clause{p_1 \cons \pi_1}{s_1})}{(\seqEmpty, \clause{p_j \cons \pi_j}{s_j})}
         \match
         \envEmpty, \exFun{(\seq{\clause{p \cons \pi}{s}})}
      }
      \and
      \inferrule*[
         lab={\ruleName{$\match$-var}}
      ]
      {
         \seq{v}, \seq{k} \match \gamma, s
      }
      {
         v \cons \seq{v}, \seqRange{(\pattVar{x} \clauseWith{\cons} k_1)}{(\pattVar{x} \clauseWith{\cons} k_j)}
         \match
         \set{\bind{x}{v}} \disjunion \gamma, s
      }
      \and
      \inferrule*[
         lab={\ruleName{$\match$-record}}
      ]
      {
         \exRecord{\seq{\bind{y}{u}}} \subseteq \exRecord{\seq{\bind{x}{v}}}
         \\
         \seq{u} \concat \seq{v}',
         (\seqRange{\seq{p_1}}{\seq{p_j}})
         \clauseWith{\concat} \seq{k}
         \match \gamma, s
      }
      {
         \exRecord{\seq{\bind{x}{v}}} \cons \seq{v}',
         (\seqRange{\pattRecord{\seq{\bind{y}{p_1}}}}{\pattRecord{\seq{\bind{y}{p_j}}}})
         \clauseWith{\cons}
         \seq{k}
         \match
         \gamma, s
      }
      \and
      \inferrule*[
         lab={\ruleName{$\match$-constr}}
      ]
      {
         \seq{v} \concat \seq{v}',
         (\pi_i \clauseWith{\concat} k_i \mid c_i = c)
         \match \gamma, s
      }
      {
         \exConstr{c}{\seq{v}} \cons \seq{v}',
         \seq{\pattConstr{c}{\pi} \clauseWith{\cons} k}
         \match
         \gamma, s
      }
   \end{smathpar}}
   \caption{Surface semantics: pattern matching}
\end{figure}
