# Supplementary material for: Cognacy Queries over Dependence Graphs for Transparent Visualisations
Source: arXiv:2403.04403 source file (2024-10-15)
Supplement: Supplementary file 7 [file typing.tex]

\section{Typing}

\subsection{Surface language typing}

\begin{figure}
   \flushleft \shadebox{$\Gamma \vdash g: \Delta$}
   \begin{smathpar}
      \inferrule*[right={
         \textnormal{$\Delta = \seq{\bind{x}{\tyFun{A}{B}}}$}
      }]
      {
         \Gamma \concat \Delta \vdash \seq{\mu: \tyFun{A}{B}}
      }
      {
         \Gamma \vdash \seq{\bind{x}{\mu}}: \Delta
      }
   \end{smathpar}

   \vspace{5pt}
   \flushleft \shadebox{$\Gamma \vdash s: A$}
   \begin{smathpar}
      \inferrule*[right={$\primOp: \tyForeign{(A,A')}{B} \in \Gamma$}]
      {
         \Gamma \vdash s: A
         \\
         \Gamma \vdash s': A'
      }
      {
         \Gamma \vdash \exBinaryApp{s}{\oplus}{s'}: B
      }
      \and
      \inferrule*[]
      {
         \Gamma \vdash \mu: \tyFun{A}{B}
      }
      {
         \Gamma \vdash \exApp{\lambda}{\mu}: \tyFun{A}{B}
      }
      \and
      \inferrule*
      {
         \Gamma \vdash g: \Delta
         \\
         \Gamma \concat \Delta \vdash s: A
      }
      {
         \Gamma \vdash \exLetRec{g}{s}: A
      }
      \and
      \inferrule*
      {
         \Gamma \vdash s: \tyBool
         \\
         \Gamma \vdash s_1: A
         \\
         \Gamma \vdash s_2: A
      }
      {
         \Gamma \vdash \exIfThenElse{s}{s_1}{s_2}: A
      }
      \and
      \inferrule*
      {
         \Gamma \vdash s: A
         \\
         \Gamma \vdash \mu: \tyFun{A}{B}
      }
      {
         \Gamma \vdash \exMatch{s}{\mu}: B
      }
      \and
      \inferrule*
      {
         p: A \dashv \Gamma'
         \\
         \Gamma \vdash s: A
         \\
         \Gamma \concat \Gamma' \vdash s': B
      }
      {
         \Gamma \vdash \exLet{p}{s}{s'}: B
      }
      \and
      \inferrule*
      {
         \Gamma \vdash s : A
         \\
         \Gamma \vdash r : \tyList{A}
      }
      {
         \Gamma \vdash \exList{s}{r} : \tyList{A}
      }
      \and
      \inferrule*
      {
         \Gamma \vdash s: \tyInt
         \\
         \Gamma \vdash s': \tyInt
      }
      {
         \Gamma \vdash \exListEnum{s}{s'}: \tyList{\tyInt}
      }
      \and
      \inferrule*
      {
         \Gamma \vdash \seq{q} \dashv \Delta
         \\
         \Gamma \concat \Delta \vdash s: A
      }
      {
         \Gamma \vdash \exListComp{s}{\seq{q}}: \tyList{A}
      }
      \end{smathpar}

      % List rest
      \vspace{5pt}
      \flushleft \shadebox{$\Gamma \vdash r: \tyList{A}$}
      \begin{smathpar}
      \inferrule*
      {
         \strut
      }
      {
         \Gamma \vdash \exListEnd : \tyList{A}
      }
      \and
      \inferrule*
      {
         \Gamma \vdash s : A
         \\
         \Gamma \vdash r : \tyList{A}
      }
      {
         \Gamma \vdash (\exListNext{s}{r}) : \tyList{A}
      }
      \end{smathpar}

      \vspace{0.1em}
      %% Qualifiers

      \flushleft \shadebox{$\Gamma \vdash \seq{q} \dashv \Delta $}
      \begin{smathpar}
      \inferrule*
      {
         \strut
      }
      {
         \Gamma \vdash \seqEmpty \dashv \seqEmpty
      }
      \and
      \inferrule*
      {
         \Gamma \vdash s: \tyBool
      }
      {
         \Gamma \vdash \qualGuard{s} \dashv \seqEmpty
      }
      \and
      \inferrule*
      {
         \Gamma \vdash s: \tyList{A}
         \\
         p: A \dashv \Delta
      }
      {
         \Gamma \vdash \qualGenerator{p}{s} \dashv \Delta
      }
      \and
      \inferrule*
      {
         \Gamma \vdash s: A
         \\
         p: A \dashv \Delta
      }
      {
         \Gamma \vdash \qualDeclaration{p}{s} \dashv \Delta
      }
      \and
      \inferrule*[
         right={$\seq{q} \neq \seqEmpty$}
      ]
      {
         \Gamma \vdash q \dashv \Gamma'
         \\
         \Gamma \concat \Gamma' \vdash \seq{q} \dashv \Delta
      }
      {
         \Gamma \vdash q \cons \seq{q} \dashv \Delta
      }
   \end{smathpar}
   \caption{Typing rules for surface terms (additional forms only) and qualifiers}
   \label{fig:surface-language:typing-term}
   \end{figure}

\begin{figure}

   %% Patterns
   \flushleft \shadebox{$\seq{p: A} \dashv \Gamma $}
   \begin{smathpar}
      \inferrule*[
         right={$\length{\seq{p}} = n$}
      ]
      {
         p_i: A_i \dashv \Gamma_i
         \quad
         (\forall i \numleq n)
      }
      {
         \seq{p: A} \dashv \seqRangeOp{\Gamma_1}{\Gamma_n}{\concat}
      }
   \end{smathpar}
   \vspace{3mm}

   \flushleft \shadebox{$p: A \dashv \Gamma $}
   \begin{smathpar}
      \inferrule*
      {
         \strut
      }
      {
         \pattVar{x}: A \dashv \set{\bind{x}{A}}
      }
      \and
      \inferrule*[
      ]
      {
         \seq{p: A} \dashv \Gamma
      }
      {
         \pattRec{\seq{\bind{x}{p}}}: \tyRec{\seq{\bind{x}{A}}} \dashv \Gamma
      }
      \and
      \inferrule*[
         right={$\datatype{c} = \tyForeign{\seq{A}}{D}$}
      ]
      {
         \seq{p: A} \dashv \Gamma
      }
      {
         \pattConstr{c}{\seq{p}}: \tyData{D} \dashv \Gamma
      }
      \and
      \inferrule*
      {
         p: A \dashv \Gamma
         \\
         o: \tyList{A} \dashv \Gamma'
      }
      {
         \pattList{p}{o} : \tyList{A} \dashv \Gamma \concat \Gamma'
      }
   \end{smathpar}
   \vspace{3mm}

   \flushleft \shadebox{$o: \tyList{A} \dashv \Gamma $}
   \begin{smathpar}
      \inferrule*
      {
         \strut
      }
      {
         \pattListEnd : \tyList{A} \dashv \seqEmpty
      }
      \and
      \inferrule*
      {
         p : A \dashv \Gamma
         \\
         o : \tyList{A} \dashv \Gamma'
      }
      {
         (\pattListNext{p}{o}) : \tyList{A} \dashv \Gamma \concat \Gamma'
      }
      \end{smathpar}
      \vspace{3mm}

      \flushleft \shadebox{$\Gamma \vdash \mu: \tyFun{A}{B}$}
      \begin{smathpar}
      \inferrule*
      {
         p: A \dashv \Gamma'
         \\
         \Gamma \concat \Gamma' \vdash s: B
      }
      {
         \Gamma \vdash \clauseUncurried{p}{s} : \tyFun{A}{B}
      }
      \and
      \inferrule*[
         right={$\seq{p} \neq \seqEmpty$}
      ]
      {
         p : A \dashv \Gamma'
         \\
         \Gamma \concat \Gamma' \vdash \clause{\seq{p}'}{s} : \tyFun{A'}{B}
      }
      {
         \Gamma \vdash \clauseUncurried{(p \cdot \seq{p})}{s} : \tyFun{A}{\tyFun{A'}{B}}
      }
      \and
      \inferrule*[
      ]
      {
         \Gamma \vdash c: \tyFun{A}{B}
         \\
         \compatPatt{c}{\mu}
         \\
         \Gamma \vdash \mu : \tyFun{A}{B}
      }
      {
         \Gamma \vdash c \cdot \mu: \tyFun{A}{B}
      }
   \end{smathpar}

\caption{Typing rules for patterns and clauses}
\label{fig:surface-language:typing-pattern}
\end{figure}

\begin{figure}
   \flushleft \shadebox{$\compatPatt{p}{p'}$}
   \begin{smathpar}
      \inferrule*[
         lab={\ruleName{$\compatPatt{}{}$-constr-neq}}
      ]
      {
         \exVar{c} \neq \exVar{c'}
      }
      {
         \compatPatt{\exConstr{c}{\seq{p}}}{\exConstr{c'}{\seq{p}'}}
      }
      \and
      \inferrule*[
         lab={\ruleName{$\compatPatt{}{}$-constr-eq}}
      ]
      {
         \compatPatt{\seq{p}}{\seq{p}'}
      }
      {
         \compatPatt{\exConstr{c}{\seq{p}}}{\exConstr{c}{\seq{p}'}}
      }
      \and
      \inferrule*[
         lab={\ruleName{$\compatPatt{}{}$-record}}
      ]
      {
         \compatPatt{\seq{p}}{\seq{p}'}
      }
      {
         \compatPatt{\exRecord{\seq{\bind{\exVar{x}}{p}}}}{\exRecord{\seq{\bind{\exVar{x}}{p}}'}}
      }
   \end{smathpar}
   {\flushleft \shadebox{$\compatPatt{\seq{p}}{\seq{p}'}$}
   \begin{smathpar}
      \inferrule*[
         lab={\ruleName{$\compatPattSym$-head}}
      ]
      {
         \compatPatt{p}{p'}
      }
      {
         \compatPatt{p\cdot\seq{p}}{p'\cdot\seq{p}'}
      }
      \and
      \inferrule*[
         lab={\ruleName{$\compatPattSym$-tail}}
      ]
      {
         \compatPatt{\seq{p}}{\seq{p}'}
      }
      {
         \compatPatt{p\cdot\seq{p}}{p\cdot\seq{p}'}
      }
   \end{smathpar}}
   {\flushleft \shadebox{$\compatPatt{c}{\mu}$}
   \begin{smathpar}
      \inferrule*[]
      {
         \exists i.(\compatPatt{p_i}{p_i'})
         \textit{ and }
         \forall j < i.\; p_j = p'_j
      }
      {
         \compatPatt{(\clause{\seq{p}}{s})}{(\clause{\seq{p}'}{s'})}
      }
      \and
      \inferrule*[
         right={$\mu \neq \seqEmpty$}
      ]
      {
         \compatPatt{c}{c'}
         \\
         \compatPatt{c}{\mu}
      }
      {
         \compatPatt{c}({c'\cdot\mu)}
      }
   \end{smathpar}}
   \caption{Disjointness of patterns and clauses}
\end{figure}

\subsection{Core language typing}

Eliminators are polymorphic in the type of the object they return, which we call the continuation type;
typically an eliminator returns another eliminator or an expression. Well-typed eliminators are
never partial.

\begin{figure}[H]
\begin{minipage}[t]{0.48\textwidth}
   \begin{tabularx}{\textwidth}{rL{2.6cm}L{3.6cm}}
      &\textit{Continuation type}&
      \\
      $K ::=$
      &
      $A$
      &
      term
      \\
      &
      $\elimTy{A}{K}$
      &
      eliminator
   \end{tabularx}
\end{minipage}
\end{figure}

\begin{figure}
   \small{\flushleft \shadebox{$\Gamma \vdash e: A$}%
   \hfill \textbfit{$e$ has type $A$ under $\Gamma$}}
   \begin{smathpar}
   \inferrule*[right={$x : A \in \Gamma$}]
   {
      \strut
   }
   {
      \Gamma \vdash \exVar{x}: A
   }
   \and
   \inferrule*
   {
      \strut
   }
   {
      \Gamma \vdash \exInt{n}: \tyInt
   }
   \and
   \inferrule*[
      right={$\datatype{c} = \tyForeign{\seq{A}}{D}$}
   ]
   {
      \Gamma \vdash \seq{e: A}
   }
   {
      \Gamma \vdash \exConstr{c}{\seq{e}}: D
   }
   \and
   \inferrule*
   {
      \Gamma \vdash e_i: \tyStr
      \\
      \Gamma \vdash e'_i: A
      \quad
      (\forall i \numleq \length{\seq{e}})
   }
   {
      \Gamma \vdash \exDict{\seq{\bind{e}{e}}'}: \tyDict{A}
   }
   \and
   \inferrule*
   {
      \Gamma \vdash \seq{e: A}
   }
   {
      \Gamma \vdash \exRec{\seq{\bind{x}{e}}}: \tyRec{\seq{\bind{x}{A}}}
   }
   \and
   \inferrule*[
      right={$i \numleq \length{\seq{x}}$}
   ]
   {
      \Gamma \vdash e: \tyRec{\seq{\bind{x}{A}}}
   }
   {
      \Gamma \vdash \exRecProj{e}{x_i}: A_i
   }
   \and
   \inferrule*
   {
      \Gamma \vdash \sigma : \elimTy{A}{B}
   }
   {
      \Gamma \vdash \exFun{\sigma} : \tyFun{A}{B}
   }
   \and
   \inferrule*[
      right={$f: \tyForeign{\seq{A}}{B} \in \Phi$}
   ]
   {
      \Gamma \vdash \seq{e: A}
   }
   {
      \Gamma \vdash f(\seq{e}): B
   }
   \and
   \inferrule*
   {
      \Gamma \vdash e: \tyFun{A}{B}
      \\
      \Gamma \vdash e': A
   }
   {
      \Gamma \vdash \exApp{e}{e'}: B
   }
   \and
   \inferrule*
   {
      \Gamma \vdash \rho: \Delta
      \\
      \Gamma \concat \Delta \vdash e: A
   }
   {
      \Gamma \vdash \exLetRec{\rho}{e}: A
   }
   \end{smathpar}
   \\[2mm]
   {\small \flushleft \shadebox{$\Gamma \vdash \sigma: \elimTy{A}{K}$}%
   \hfill \textbfit{$\sigma$ has type $\elimTy{A}{K}$ under $\Gamma$}}
   \begin{smathpar}
   \inferrule*
   {
      \Gamma \cons \bind{x}{A} \vdash \kappa: K
   }
   {
      \Gamma \vdash (\elimVar{x}{\kappa}): \elimTy{A}{K}
   }
   \and
   \inferrule*
   {
      (\datatype{c_i} = \tyForeign{\seq{A}_i}{D} \in
       \implies
       \Gamma \vdash \kappa_i: \elimTy{\seq{A}_i}{K})
      \quad
      (\forall i \numleq \length{\seq{c}})
   }
   {
      \Gamma \vdash \{\seq{\elimBind{c}{\kappa}}\}: \elimTy{D}{K}
   }
   \and
   \inferrule*
   {
      \Gamma \vdash \kappa: K
   }
   {
      \Gamma
      \vdash
      \elimRecord{}{\kappa}: \elimTy{\tyRecEmpty}{K}
   }
   \and
   \inferrule*
   {
      \Gamma \vdash \elimRecord{\seq{x}}{\sigma}: \elimTy{\tyRec{\seq{\bind{x}{A}}}}{\elimTy{B}{K}}
   }
   {
      \Gamma
      \vdash
      \elimRecord{\seq{x} \cons y}{\sigma}: \elimTy{\tyRec{\seq{\bind{x}{A}} \cons \bind{y}{B}}}{K}
   }
   \end{smathpar}
   \\[2mm]
   {\small \flushleft \shadebox{$\vdash v: A$}%
   \hfill \textbfit{$v$ has type $A$}}
   \begin{smathpar}
   \inferrule*
   {
      \strut
   }
   {
      \vdash \exInt{n}: \tyInt
   }
   \and
   \inferrule*
   {
      \vdash \seq{v: A}
   }
   {
      \vdash \exRec{\seq{\bind{x}{v}}}: \tyRec{\seq{\bind{x}{A}}}
   }
   \and
   \inferrule*
   {
      \vdash \gamma: \Gamma
      \\
      \Gamma \vdash \rho: \Delta
      \\
      \Gamma \concat \Delta \vdash \sigma: \elimTy{A}{B}
   }
   {
      \vdash \exClosure{\gamma}{\rho}{\sigma}: \tyFun{A}{B}
   }
   \and
   \inferrule*[
      right={$\datatype{c} = \tyForeign{\seq{A}}{D}$}
   ]
   {
      \Gamma \vdash \seq{v: A}
   }
   {
      \Gamma \vdash \exConstr{c}{\seq{v}}: \tyData{D}
   }
   \end{smathpar}
   \\[2mm]
   \begin{minipage}[t]{0.4\textwidth}%
   {\small \flushleft \shadebox{$\vdash \gamma: \Gamma$}%
   \hfill \textbfit{$\gamma$ has type $\Gamma$}}
   \begin{smathpar}
   \inferrule*
   {
      \vdash \seq{v: A}
   }
   {
      \vdash \seq{\bind{x}{v}}: \seq{\bind{x}{A}}
   }
   \end{smathpar}
   \end{minipage}%
   \hspace{5mm}%
   \begin{minipage}[t]{0.5\textwidth}%
   {\small \flushleft \shadebox{$\Gamma \vdash \rho: \Delta$}%
   \hfill \textbfit{$\rho$ has type $\Delta$ under $\Gamma$}}
   \begin{smathpar}
      \inferrule*[right={
         \textnormal{$\Delta = \seq{\bind{x}{\tyFun{A}{B}}}$}
      }]
      {
         \Gamma \concat \Delta \vdash \seq{\sigma: \elimTy{A}{B}}
      }
      {
         \Gamma \vdash \seq{\bind{x}{\sigma}}: \Delta
      }
   \end{smathpar}
   \end{minipage}
   \caption{Typing rules for core language}
   \label{fig:core-language:typing}
\end{figure}
