# Supplementary material for: Cognacy Queries over Dependence Graphs for Transparent Visualisations
Source: arXiv:2403.04403 source file (2024-10-15)
Supplement: Supplementary file 8 [file dict-primitives.tex]

\begin{figure}
\small
\addtolength{\jot}{-0.4em}
\begin{align*}
   % =============================================================
   \dictMap &: \Val{(\tyFun{A}{B})} \times \Val{(\tyDict{A})} \to \Val{(\tyDict{B})}
   % =============================================================
   \\
   \dictMap(v, d_{\alpha})
   &=
   (\annDict{\seq{\bind{s}{(\alpha', v')}}}{\beta}, \bigcup\set{\seq{E}} \cup \set{(\alpha, \beta)})
   \\
   &\quad\textit{where }\beta\textit{ fresh and }
   \set{\seq{\bind{s}{(\alpha', (v',E))}}} = \Dmap(\lambda(\alpha', u).(\alpha', \apply(v, u)), d)
   \\[2mm]
   % =============================================================
   \dictIntersectionWith
   &:
   \Val{(\tyFun{A}{\tyFun{B}{A'}})} \times \Val{(\tyDict{A})} \times \Val{(\tyDict{B})} \to \Val{(\tyDict{A'})}
   % =============================================================
   \\
   \dictIntersectionWith(v, d_{\alpha}, d'_{\alpha'})
   &=
    (\annDict{\seq{\bind{s}{(\beta', v'}}}{\beta},
    \bigcup\set{\seq{E}} \cup \set{(\alpha, \beta), (\alpha', \beta)}
   \\
   &\quad\textit{ where }\beta\textit{ fresh and }
   \set{\seq{\bind{s}{(\beta', (v',E))}}} = \DintersectionWith(f, d, d')
   \\
   &\quad\textit{ and }
   f((\beta', u), (\_, u')) = (\beta', \apply(v, (u, u')))
   \\[2mm]
   % =============================================================
   \dictDisjUnion &: \Val{(\tyDict{A})}^2 \to \Val{(\tyDict{A})}
   % =============================================================
   \\
   \dictDisjUnion(d_{\alpha}, d'_{\alpha'})
   &=
   ((d \disjunion d')_{\beta}, \set{(\alpha, \beta), (\alpha', \beta)})
   \quad\;\textit{iff }\beta\textit{ fresh and }\dom{d} \cap \dom{d'} = \varnothing
   \\[2mm]
   % =============================================================
   \dictDifference &: \Val{(\tyDict{A})} \times \Val{(\tyDict{B})} \to \Val{(\tyDict{A})}
   % =============================================================
   \\
   \dictDifference(d_{\alpha}, d'_{\beta})
   &=
   ((\Ddifference(d, d')_{\beta}, \set{(\alpha, \beta), (\alpha', \beta)})
   \quad\;\textit{where }\beta\textit{ fresh}
   \\[2mm]
   % =============================================================
   \dictGet &: \Val{\tyStr} \times \Val{(\tyDict{A})} \to \Val{A}
   % =============================================================
   \\
   \dictGet(\annStr{s}{\alpha}, d_{\alpha'}) &= (v, \varnothing)
   \quad\textit{iff }\bind{s}{(\beta, v)} \in d
   \\[2mm]
   % =============================================================
   \dictFoldl &: \Val{(\tyFun{B}{\tyFun{A}{B}})} \times \Val{B} \times \Val{(\tyDict{A})} \to \Val{B}
   % =============================================================
   \\
   \dictFoldl(v, u, d_\alpha) &= \Dfoldl(f, (u, \varnothing), d)
   \\
   &\quad\textit{where }
   f(s, (v', E), (\_, u')) = (v^\dagger, E \cup E')\textit{ where }(v^\dagger, E') = \apply(v, (v', u'))
   \\[2mm]
   % =============================================================
   \dictFromRecord &: \Val{(\tyRec{\seqRange{\bind{x_1}{A}}{\bind{x_n}{A}}})} \to \Val{(\tyDict{A})}
   % =============================================================
   \\
   \dictFromRecord(\annRec{\seq{\bind{x}{v}}}{\alpha})
   &=
   (\annDict{\seq{\bind{s}{(\beta, v)}}}{\alpha'},
    \set{(\alpha, \alpha')} \cup (\alpha, \set{\seq{\beta}})
   \quad\textit{where }\alpha', \seq{\beta}\textit{ fresh and }\str(x_i) = s_i
\end{align*}
\caption{Foreign functions for dictionaries; $\dictFromRecord$ assumes embedding $\str: \Var \hookrightarrow \Str$}
\end{figure}
