# Supplementary material for: Cognacy Queries over Dependence Graphs for Transparent Visualisations
Source: arXiv:2403.04403 source file (2024-10-15)
Supplement: Supplementary file 9 [file clauses-bwd.tex]

\begin{figure}
   {\flushleft \shadebox{$\mu' \desugarBwd{\mu} \sigma$}
   \hfill}
   \begin{smathpar}
      \inferrule*[
         lab={\ruleName{$\desugar$-fun}}
      ]
      {
         \seq{(p, \clause{\pi}{s'})}
         \desugarBwd{\seq{(p, \clause{\pi}{s})}}
         \sigma
      }
      {
         \seq{\clause{p \cons \pi}{s'}}
         \desugarBwd{\seq{\clause{p \cons \pi}{s}}}
         \sigma
      }
   \end{smathpar}
   \\[2mm]
   {\flushleft \shadebox{$\seq{k} \desugarBwd{\seq{k}} \kappa$}
   \hfill}
   \begin{smathpar}
      \inferrule*[
         lab={\ruleName{$\desugarBwd{}$-clauses-done}}
      ]
      {
         s' \desugarBwd{s} e
      }
      {
         (\seqEmpty, \clause{\seqEmpty}{s'}) \desugarBwd{(\seqEmpty, \clause{\seqEmpty}{s})} e
      }
      \and
      \inferrule*[
         lab={\ruleName{$\desugarBwd{}$-clauses-next-arg}}
      ]
      {
         \seq{(p', \clause{\pi'}{s'})}
         \desugarBwd{\seq{(p, \clause{\pi}{s})}}
         \sigma
      }
      {
         \seqRange{(\seqEmpty, \clause{p'_1 \cons \pi'_1}{s'_1})}
                  {(\seqEmpty, \clause{p'_{j'} \cons \pi'_{j'}}{s'_{j'}})}
         \desugarBwd{
            \seqRange{(\seqEmpty, \clause{p_1 \cons \pi_1}{s_1})}
                     {(\seqEmpty, \clause{p_j \cons \pi_j}{s_j})}
         }
         \exFun{\sigma}
      }
      \and
      \inferrule*[
         lab={\ruleName{$\desugarBwd{}$-clauses-var}}
      ]
      {
         \seq{k'} \desugarBwd{\seq{k}} \kappa
      }
      {
         \seqRange{(\pattVar{x} \clauseWith{\cons} k'_1)}{(\pattVar{x} \clauseWith{\cons} k'_j)}
         \desugarBwd{\seqRange{(\pattVar{x} \clauseWith{\cons} k_1)}{(\pattVar{x} \clauseWith{\cons} k_j)}}
         \elimVar{x}{\kappa}
      }
      \and
      \inferrule*[
         lab={\ruleName{$\desugarBwd{}$-clauses-record}}
      ]
      {
         (\seqRange{\seq{p'_1}}{\seq{p'_{j'}}}) \clauseWith{\concat} \seq{k'}
         \desugarBwd{(\seqRange{\seq{p_1}}{\seq{p_j}}) \clauseWith{\concat} \seq{k}}
         \kappa
      }
      {
         (\seqRange{\pattRecord{\seq{\bind{x}{p'_1}}}}{\pattRecord{\seq{\bind{x}{p'_{j'}}}}})
         \clauseWith{\cons}
         \seq{k'}
         \desugarBwd{
            (\seqRange{\pattRecord{\seq{\bind{x}{p_1}}}}{\pattRecord{\seq{\bind{x}{p_j}}}})
            \clauseWith{\cons}
            \seq{k}
         }
         \elimRecord{\seq{x}}{\kappa}
      }
      \and
      \inferrule*[
         lab={\ruleName{$\desugarBwd{}$-clauses-constr}}
      ]
      {
         ((\pi'_i \clauseWith{\concat} k'_i) \mid c_i = c)
         \desugarBwd{((\pi_i \clauseWith{\concat} k_i) \mid c_i = c)}
         \kappa_c
         \\
         (\forall c \in \set{\seq{c'}})
      }
      {
         \seq{\pattConstr{c'}{\pi'} \clauseWith{\cons} k'}
         \desugarBwd{\seq{\pattConstr{c}{\pi} \clauseWith{\cons} k}}
         \elimConstr{\seq{\elimBind{c'}{\kappa}}}
      }
   \end{smathpar}
   \caption{Desugaring for function definitions (backwards rules)}
   \label{fig:desugar:clauses:bwd}
\end{figure}
