# Supplementary material for: Cognacy Queries over Dependence Graphs for Transparent Visualisations
Source: arXiv:2403.04403 source file (2024-10-15)
Supplement: Supplementary file 10 [file clauses.tex]

\begin{figure}
   {\flushleft \shadebox{$\mu \desugar \sigma$}
   \hfill}
   \begin{smathpar}
      \inferrule*[
         lab={\ruleName{$\desugar$-fun}}
      ]
      {
         \seq{(p, \clause{\pi}{s})}
         \desugar \sigma
      }
      {
         \seq{\clause{p \cons \pi}{s}}
         \desugar
         \sigma
      }
   \end{smathpar}
   \\[2mm]
   {\flushleft \shadebox{$\seq{k} \desugar \kappa$}
   \hfill}
   \begin{smathpar}
      \inferrule*[
         lab={\ruleName{$\desugar$-clauses-done}}
      ]
      {
         s \desugar e
      }
      {
         (\seqEmpty, \clause{\seqEmpty}{s}) \desugar e
      }
      \and
      \inferrule*[
         lab={\ruleName{$\desugar$-clauses-next-arg}}
      ]
      {
         \seq{(p, \clause{\pi}{s})}
         \desugar
         \sigma
      }
      {
         \seqRange{(\seqEmpty, \clause{p_1 \cons \pi_1}{s_1})}
                  {(\seqEmpty, \clause{p_j \cons \pi_j}{s_j})}
         \desugar
         \exFun{\sigma}
      }
      \and
      \inferrule*[
         lab={\ruleName{$\desugar$-clauses-var}}
      ]
      {
         \seq{k} \desugar \kappa
      }
      {
         \seqRange{(\pattVar{x} \clauseWith{\cons} k_1)}{(\pattVar{x} \clauseWith{\cons} k_j)}
         \desugar
         \elimVar{x}{\kappa}
      }
      \and
      \inferrule*[
         lab={\ruleName{$\desugar$-clauses-record}}
      ]
      {
         (\seqRange{\seq{p_1}}{\seq{p_j}}) \clauseWith{\concat} \seq{k} \desugar \kappa
      }
      {
         (\seqRange{\pattRecord{\seq{\bind{x}{p_1}}}}{\pattRecord{\seq{\bind{x}{p_j}}}})
         \clauseWith{\cons}
         \seq{k}
         \desugar
         \elimRecord{\seq{x}}{\kappa}
      }
      \and
      \inferrule*[
         lab={\ruleName{$\desugar$-clauses-constr}}
      ]
      {
         ((\pi_i \clauseWith{\concat} k_i) \mid c_i = c) \desugar \kappa_c
         \\
         \datatype{c} = D
         \quad
         (\forall c \in \set{\seq{c}})
      }
      {
         \seq{\pattConstr{c}{\pi} \clauseWith{\cons} k}
         \desugar
         \elimConstr{\elimBind{c}{\kappa_c} \mid c \in \set{\seq{c}}}
      }
      \and
      \inferrule*[
         lab={\ruleName{$\desugar$-clauses-non-empty-list}}
      ]
      {
         (\pattConstr{\cCons}{p \cons o} \clauseWith{\cons} k) \cons \seq{k}
         \desugar
         \kappa
      }
      {
         (\pattList{p}{o} \clauseWith{\cons} k)
         \cons
         \seq{k}
         \desugar
         \kappa
      }
      \and
      \inferrule*[
         lab={\ruleName{$\desugar$-list-end}}
      ]
      {
         (\cNil \clauseWith{\cons} k) \cons \seq{k}
         \desugar
         \kappa
      }
      {
         (\pattListEnd \clauseWith{\cons} k)
         \cons
         \seq{k}
         \desugar
         \kappa
      }
      \and
      \inferrule*[
         lab={\ruleName{$\desugar$-list-cons}}
      ]
      {
         (\pattConstr{\cCons}{p \cons o} \clauseWith{\cons} k) \cons \seq{k}
         \desugar
         \kappa
      }
      {
         (\pattListNext{p}{o} \clauseWith{\cons} k)
         \cons
         \seq{k}
         \desugar
         \kappa
      }
   \end{smathpar}
   \caption{Desugaring for function definitions}
   \label{fig:desugar:clauses}
\end{figure}
