# Supplementary material for: Cognacy Queries over Dependence Graphs for Transparent Visualisations
Source: arXiv:2403.04403 source file (2024-10-15)
Supplement: Supplementary file 11 [file or-else-bwd.tex]

\begin{figure}
   {\small \flushleft \shadebox{$s, \alpha \orElseBwd{k} \mu$}
   \begin{smathpar}
      \inferrule*[
         lab={\ruleName{$\orElseBwd{}$-done}}
      ]
      {
         \strut
      }
      {
         s', \bot
         \orElseBwd{(\seqEmpty, \clause{\seqEmpty}{s})}
         \clause{\seqEmpty}{s'}
      }
      \and
      \inferrule*[
         lab={\ruleName{$\orElseBwd{}$-var}}
      ]
      {
         s, \alpha \orElseBwd{k} \seqRange{k'_1}{k'_j}
      }
      {
         s, \alpha
         \orElseBwd{\pattVar{x} \clauseWith{\cons} k}
         \seqRange{\pattVar{x} \clauseWith{\cons} k'_1}
                  {\pattVar{x} \clauseWith{\cons} k'_j}
      }
      \and
      \inferrule*[
         lab={\ruleName{$\orElseBwd{}$-record}}
      ]
      {
         s, \alpha
         \orElseBwd{\seq{p} \clauseWith{\concat} k}
         \seqRange{\seq{p_1} \clauseWith{\concat} k'_1}
                  {\seq{p_j} \clauseWith{\concat} k'_j}
      }
      {
         s, \alpha
         \orElseBwd{\pattRecord{\seq{\bind{x}{p}}} \clauseWith{\cons} k}
         \seqRange{\pattRecord{\seq{\bind{x}{p_1}}} \clauseWith{\cons} k'_1}
                  {\pattRecord{\seq{\bind{x}{p_j}}} \clauseWith{\cons} k'_j}
      }
      \and
      \inferrule*[
         lab={\ruleName{$\orElseBwd{}$-constr}}
      ]
      {
         s, \beta
         \orElseBwd{\pi \clauseWith{\concat} k}
         \seq{\pi \clauseWith{\concat} k'}
         \\
         k^\twoPrime_i =
         \clause{(\pattVar{\varAnon} \mid n \numleq \length{\pi'})}{\alpha_i}
         \quad
         (\forall i \numleq \length{\seq{c}})
         \\
         \ctrsF(D) \supseteq c \cons \set{\seq{c}}
      }
      {
         s, \bigjoin\set{\seq{\alpha}} \join \beta
         \orElseBwd{\pattConstr{c}{\pi} \clauseWith{\cons} k}
         (\seqRange{\pattConstr{c}{\pi_1} \clauseWith{\cons} k'_1}
                   {\pattConstr{c}{\pi_j} \clauseWith{\cons} k'_j})
         \concat
         (\pattConstr{c_i}{\pattVar{\varAnon} \mid n \numleq \arity{c_i}}
         \clauseWith{\cons} k^\twoPrime_i
         \mid i \numleq \length{\seq{c}})
      }
      \and
      \inferrule*[
         lab={\ruleName{$\orElseBwd{}$-non-empty-list}}
      ]
      {
         s, \alpha
         \orElseBwd{p \clauseWith{\cons} o \clauseWith{\cons} k}
         \seq{p' \clauseWith{\cons} o' \clauseWith{\cons} k'}
      }
      {
         s, \alpha
         \orElseBwd{\pattList{p}{o} \clauseWith{\cons} k}
         \seqRange{\pattList{p'_1}{o'_1} \clauseWith{\cons} k'_1}
                  {\pattList{p'_j}{o'_j} \clauseWith{\cons} k'_j},
         k^\twoPrime
      }
      \and
      \inferrule*[
         lab={\ruleName{$\orElseBwd{}$-list-end}}
      ]
      {
         s, \alpha \orElseBwd{k} \seq{k}'
      }
      {
         s, \alpha
         \orElseBwd{\pattListEnd \clauseWith{\cons} k}
         \seqRange{\pattListEnd \clauseWith{\cons} k'_1}
                  {\pattListEnd \clauseWith{\cons} k'_j},
         k^\twoPrime
      }
      \and
      \inferrule*[
         lab={\ruleName{$\orElseBwd{}$-list-cons}}
      ]
      {
         s, \alpha
         \orElseBwd{p \clauseWith{\cons} o \clauseWith{\cons} k}
         \seq{p' \clauseWith{\cons} o' \clauseWith{\cons} k'}
      }
      {
         s, \alpha
         \orElseBwd{(\pattListNext{p}{o}) \clauseWith{\cons} k}
         \seqRange{(\pattListNext{p'_1}{o'_1}) \clauseWith{\cons} k'_1}
                  {(\pattListNext{p'_j}{o'_j}) \clauseWith{\cons} k'_j},
         k^\twoPrime
      }
   \end{smathpar}}
   \caption{Completing an (uncurried) clause with a default value of $\exNil$ (backwards rules)}
\end{figure}
