# Supplementary material for: Cognacy Queries over Dependence Graphs for Transparent Visualisations
Source: arXiv:2403.04403 source file (2024-10-15)
Supplement: Supplementary file 12 [file or-else.tex]

\begin{figure}
   {\small \flushleft \shadebox{$k, \alpha \orElse \mu$}
   \begin{smathpar}
      \inferrule*[
         lab={\ruleName{$\orElse$-done}}
      ]
      {
         \strut
      }
      {
         (\seqEmpty, \clause{\seqEmpty}{s}), \alpha
         \orElse
         \clause{\seqEmpty}{s}
      }
      \and
      \inferrule*[
         lab={\ruleName{$\orElse$-var}}
      ]
      {
         k, \alpha \orElse \seqRange{k_1}{k_j}
      }
      {
         \pattVar{x} \clauseWith{\cons} k, \alpha
         \orElse
         \seqRange{\pattVar{x} \clauseWith{\cons} k_1}
                  {\pattVar{x} \clauseWith{\cons} k_j}
      }
      \and
      \inferrule*[
         lab={\ruleName{$\orElse$-record}}
      ]
      {
         \seq{p} \clauseWith{\concat} k, \alpha
         \orElse
         \seqRange{\seq{p_1} \clauseWith{\concat} k_1}
                  {\seq{p_j} \clauseWith{\concat} k_j}
      }
      {
         \pattRecord{\seq{\bind{x}{p}}} \clauseWith{\cons} k, \alpha
         \orElse
         \seqRange{\pattRecord{\seq{\bind{x}{p_1}}} \clauseWith{\cons} k_1}
                  {\pattRecord{\seq{\bind{x}{p_j}}} \clauseWith{\cons} k_j}
      }
      \and
      \inferrule*[
         lab={\ruleName{$\orElse$-constr}},
         right={$\ctrsF(D) = c \cons \set{\seq{c}}$}
      ]
      {
         \pi \clauseWith{\concat} k, \alpha
         \orElse
         \seq{\pi \clauseWith{\concat} k}
         \\
         \seq{k}' =
         ((\pattVar{\varAnon} \mid n \numleq \length{\pi'}, \clause{\seqEmpty}{\annot{\exNil}{\alpha}})
         \mid
         i \numleq \length{\seq{c}})
         \\
         k = (\pi', \clause{\seqEmpty}{s})
      }
      {
         \pattConstr{c}{\pi} \clauseWith{\cons} k, \alpha
         \orElse
         (\seqRange{\pattConstr{c}{\pi_1} \clauseWith{\cons} k_1}
                   {\pattConstr{c}{\pi_j} \clauseWith{\cons} k_j})
         \concat
         (\pattConstr{c_i}{\pattVar{\varAnon} \mid n \numleq \arity{c_i}}
         \clauseWith{\cons} k'_i
         \mid i \numleq \length{\seq{c}})
      }
      \and
      \inferrule*[
         lab={\ruleName{$\orElse$-non-empty-list}}
      ]
      {
         p \clauseWith{\cons} o \clauseWith{\cons} k, \alpha
         \orElse
         \seq{p \clauseWith{\cons} o \clauseWith{\cons} k}
         \\
         k = (\pi, \clause{\seqEmpty}{s})
      }
      {
         \pattList{p}{o}
         \clauseWith{\cons} k, \alpha
         \orElse
         \seqRange{\pattList{p_1}{o_1} \clauseWith{\cons} k_1}
                  {\pattList{p_j}{o_j} \clauseWith{\cons} k_j},
         \pattNil \cons \pi, \clause{\seqEmpty}{\annot{\exNil}{\alpha}}
      }
      \and
      \inferrule*[
         lab={\ruleName{$\orElse$-list-end}}
      ]
      {
         k, \alpha \orElse \seq{k}
         \\
         k = (\pi, \clause{\seqEmpty}{s})
      }
      {
         \pattListEnd
         \clauseWith{\cons} k, \alpha
         \orElse
         \seqRange{\pattListEnd \clauseWith{\cons} k_1}
                  {\pattListEnd \clauseWith{\cons} k_j},
         (\pattListNext{\pattVar{\varAnon}}{\pattVar{\varAnon}}) \cons \pi, \clause{\seqEmpty}{\annot{\exNil}{\alpha}}
      }
      \and
      \inferrule*[
         lab={\ruleName{$\orElse$-list-cons}}
      ]
      {
         p \clauseWith{\cons} o \clauseWith{\cons} k, \alpha
         \orElse
         \seq{p \clauseWith{\cons} o \clauseWith{\cons} k}
         \\
         k = (\pi, \clause{\seqEmpty}{s})
      }
      {
         (\pattListNext{p}{o})
         \clauseWith{\cons} k, \alpha
         \orElse
         \seqRange{(\pattListNext{p_1}{o_1}) \clauseWith{\cons} k_1}
                  {(\pattListNext{p_j}{o_j}) \clauseWith{\cons} k_j},
         \pattListEnd \cons \pi, \clause{\seqEmpty}{\annot{\exNil}{\alpha}}
      }
   \end{smathpar}}
   \caption{Completing an (uncurried) clause with a default value of $\exNil$}
\end{figure}
