# Supplementary material for: Cognacy Queries over Dependence Graphs for Transparent Visualisations
Source: arXiv:2403.04403 source file (2024-10-15)
Supplement: Supplementary file 13 [file term-bwd.tex]

\begin{figure}
   {\flushleft \shadebox{$s' \desugarBwd{s} e$}\hfill}
   \begin{smathpar}
      \inferrule*[lab={\ruleName{$\desugarBwd{}$-lambda}}]
      {
         \mu' \desugarBwd{\mu} \sigma
      }
      {
         \exFun{\mu'} \desugarBwd{\exFun{\mu}} \exFun{\sigma}
      }
      \and
      \inferrule*[lab={\ruleName{$\desugarBwd{}$-binary-apply}}]
      {
         s_1' \desugarBwd{s_1} e_1
         \\
         s_2' \desugarBwd{s_2} e_2
      }
      {
         \exBinaryApp{s_1'}{\oplus}{s_2'}
         \desugarBwd{\exBinaryApp{s_1}{\oplus}{s_2}}
         \exForeignApp{\oplus}{e, e'}
      }
      \and
      \inferrule*[lab={\ruleName{$\desugarBwd{}$-let-rec}}]
      {
         \seq{\mu'} \desugarBwd{\seq{\mu}} \seq{\sigma}
         \\
         s' \desugarBwd{s} e
      }
      {
         \exLetRecPiecewise{\seq{\bind{x}{\mu'}}}{s'}
         \desugarBwd{\exLetRecPiecewise{\seq{\bind{x}{\mu}}}{s}}
         \exLetRecPiecewise{\seq{\bind{x}{\sigma}}}{e}
      }
      \and
      \inferrule*[lab={\ruleName{$\desugarBwd{}$-match}}]
      {
         s' \desugarBwd{s} e
         \\
         \mu' \desugarBwd{\mu} \sigma
      }
      {
         \exMatch{s'}{\mu'}
         \desugarBwd{\exMatch{s}{\mu}}
         \exApp{\exFun{\sigma}}{e}
      }
      \and
      \inferrule*[lab={\ruleName{$\desugarBwd{}$-non-empty-list}}]
      {
         s' \desugarBwd{s} e
         \\
         l' \desugarBwd{l} e'
      }
      {
         \exList{s'}{l'}
         \desugarBwd{\exList{s}{l}}
         \exConstr{\cCons}{e, e'}
      }
      \and
      \inferrule*[lab={\ruleName{$\desugarBwd{}$-if}}]
      {
         s' \desugarBwd{s} e
         \\
         s_1' \desugarBwd{s_1} e_1
         \\
         s_2' \desugarBwd{s_2} e_2
         \\
         \sigma = \elimConstr{\elimBind{\cTrue}{e_1}, \elimBind{\cFalse}{e_2}}
      }
      {
         \exIfThenElse{s'}{s_1'}{s_2'}
         \desugarBwd{\exIfThenElse{s'}{s_1'}{s_2'}}
         \exApp{\exFun{\sigma}}{e}
      }
      \and
      \inferrule*[lab={\ruleName{$\desugarBwd{}$-list-enum}}]
      {
         s_1' \desugarBwd{s_1} e
         \\
         s_2' \desugarBwd{s_2} e'
      }
      {
         \exListEnum{s_1'}{s_2'}
         \desugarBwd{\exListEnum{s_1}{s_2}}
         \exApp{\exApp{\varEnumFromTo}{e}}{e'}
      }
      \and
      \inferrule*[lab={\ruleName{$\desugarBwd{}$-list-comp-done}}]
      {
         s' \desugarBwd{s} e
      }
      {
         \exListComp{s'}{\seqEmpty}
         \desugarBwd{\exListComp{s}{\seqEmpty}}
         \exConstr{\cCons}{e, \exNil}
      }
      \and
      \inferrule*[lab={\ruleName{$\desugarBwd{}$-list-comp-guard}}]
      {
         s_1' \desugarBwd{s_1} e
         \\
         \exListComp{s_2'}{\seq{q}'}
         \desugarBwd{\exListComp{s_2}{\seq{q}}}
         e'
         \\
         \sigma = \elimConstr{\elimBind{\cTrue}{e'}, \elimBind{\cFalse}{\exNil}}
      }
      {
         \exListComp{s_2'}{\qualGuard{s_1'} \cons \seq{q}'}
         \desugarBwd{\exListComp{s_2}{\qualGuard{s_1} \cons \seq{q}}}
         \exApp{\exFun{\sigma}}{e}
      }
      \and
      \inferrule*[lab={\ruleName{$\desugarBwd{}$-list-comp-decl}}]
      {
         s_1' \desugarBwd{s_1} e
         \\
         (\clause{p}{\exListComp{s_2'}{\seq{q}'}})
         \desugarBwd{\clause{p}{\exListComp{s_2}{\seq{q}}}}
         \sigma
      }
      {
         \exListComp{s_2'}{\qualDeclaration{p}{s_1'} \cons \seq{q}'}
         \desugarBwd{\exListComp{s_2}{\qualDeclaration{p}{s_1} \cons \seq{q}}}
         \exApp{\exFun{\sigma}}{e}
      }
      \and
      \inferrule*[
         lab={\ruleName{$\desugarBwd{}$-list-comp-gen}}
      ]
      {
         s_1' \desugarBwd{s_1} e
         \\
         \exListComp{s_2'}{\seq{q}'}, \exNil
         \orElseBwd{\clause{p}{\exListComp{s_2}{\seq{q}}}}
         \mu'
         \\
         \mu' \desugarBwd{\mu} \sigma
         \\
         (\clause{p}{\exListComp{s_2}{\seq{q}}}) \orElse \mu
      }
      {
         \exListComp{s_2'}{\qualGenerator{p}{s_1'} \cons \seq{q}'}
         \desugarBwd{\exListComp{s_2}{\qualGenerator{p}{s_1} \cons \seq{q}}}
         \exApp{\exApp{\varConcatMap}{\exFun{\sigma}}}{e}
      }
   \end{smathpar}
   \\[2mm]
   {\flushleft \shadebox{$l' \desugarBwd{l} e$}
   \hfill}
   \begin{smathpar}
      \inferrule*[lab={\ruleName{$\desugarBwd{}$-list-rest-nil}}]
      {
         \strut
      }
      {
         \exListEnd
         \desugarBwd{\exListEnd}
         \exListEnd,
         \exNil
      }
      \and
      \inferrule*[lab={\ruleName{$\desugarBwd{}$-list-rest-cons}}]
      {
         s' \desugarBwd{s} e
         \\
         l' \desugarBwd{l} e'
      }
      {
         (\exListNext{s'}{l'})
         \desugarBwd{\exListNext{s}{l}}
         \exConstr{\cCons}{e, e'}
      }
   \end{smathpar}
   \caption{Desugaring for terms and function definitions (backwards rules)}
   \label{fig:desugar}
\end{figure}
