# Supplementary material for: Cognacy Queries over Dependence Graphs for Transparent Visualisations
Source: arXiv:2403.04403 source file (2024-10-15)
Supplement: Supplementary file 14 [file term.tex]

\begin{figure}
   {\flushleft \shadebox{$s \desugar e$}\hfill}
   \begin{smathpar}
      \inferrule*[lab={\ruleName{$\desugar$-lambda}}]
      {
         \mu \desugar \sigma
      }
      {
         \exFun{\mu} \desugar \exFun{\sigma}
      }
      \and
      \inferrule*[lab={\ruleName{$\desugar$-binary-apply}}]
      {
         s_1 \desugar e_1
         \\
         s_2 \desugar e_2
      }
      {
         \exBinaryApp{s_1}{\oplus}{s_2}
         \desugar
         \exForeignApp{\oplus}{e, e'}
      }
      \and
      \inferrule*[lab={\ruleName{$\desugar$-let-rec}}]
      {
         \seq{\mu} \desugar \seq{\sigma}
         \\
         s \desugar e
      }
      {
         \exLetRecPiecewise{\seq{\bind{x}{\mu}}}{s}
         \desugar
         \exLetRecPiecewise{\seq{\bind{x}{\sigma}}}{e}
      }
      \and
      \inferrule*[lab={\ruleName{$\desugar$-match}}]
      {
         s \desugar e
         \\
         \mu \desugar\sigma
      }
      {
         \exMatch{s}{\mu}
         \desugar
         \exApp{\exFun{\sigma}}{e}
      }
      \and
      \inferrule*[lab={\ruleName{$\desugar$-non-empty-list}}]
      {
         s \desugar e
         \\
         l \desugar e'
      }
      {
         \exList{s}{l}
         \desugar
         \exConstr{\cCons}{e, e'}
      }
      \and
      \inferrule*[lab={\ruleName{$\desugar$-if}}]
      {
         s \desugar e
         \\
         s_1 \desugar e_1
         \\
         s_2 \desugar e_2
         \\
         \sigma = \elimConstr{\elimBind{\cTrue}{e_1}, \elimBind{\cFalse}{e_2}}
      }
      {
         \exIfThenElse{s}{s_1}{s_2}
         \desugar
         \exApp{\exFun{\sigma}}{e}
      }
      \and
      \inferrule*[lab={\ruleName{$\desugar$-list-enum}}]
      {
         s_1 \desugar e
         \\
         s_2 \desugar e'
      }
      {
         \exListEnum{s_1}{s_2}
         \desugar
         \exApp{\exApp{\varEnumFromTo}{e}}{e'}
      }
      \and
      \inferrule*[lab={\ruleName{$\desugar$-list-comp-done}}]
      {
         s \desugar e
      }
      {
         \exListComp{s}{\seqEmpty}
         \desugar
         \exConstr{\cCons}{e, \exNil}
      }
      \and
      \inferrule*[lab={\ruleName{$\desugar$-list-comp-guard}}]
      {
         s \desugar e
         \\
         \exListComp{s'}{\seq{q}} \desugar e'
         \\
         \sigma = \elimConstr{\elimBind{\cTrue}{e'}, \elimBind{\cFalse}{\exNil}}
      }
      {
         \exListComp{s'}{\qualGuard{s} \cons \seq{q}}
         \desugar
         \exApp{\exFun{\sigma}}{e}
      }
      \and
      \inferrule*[lab={\ruleName{$\desugar$-list-comp-decl}}]
      {
         s \desugar e
         \\
         (\clause{p}{\exListComp{s'}{\seq{q}}}) \desugar \sigma
      }
      {
         \exListComp{s'}{\qualDeclaration{p}{s} \cons \seq{q}}
         \desugar
         \exApp{\exFun{\sigma}}{e}
      }
      \and
      \inferrule*[lab={\ruleName{$\desugar$-list-comp-gen}}]
      {
         s \desugar e
         \\
         (\clause{p}{\exListComp{s'}{\seq{q}}}) \orElse \mu
         \\
         \mu \desugar \sigma
      }
      {
         \exListComp{s'}{\qualGenerator{p}{s} \cons \seq{q}}
         \desugar
         \exApp{\exApp{\varConcatMap}{\exFun{\sigma}}}{e}
      }
   \end{smathpar}
   \\[2mm]
   {\flushleft \shadebox{$l \desugar e$}
   \hfill \phantom{blah}}% \textbfit{$l$ desugars to $e$}}
   \begin{smathpar}
      \inferrule*[lab={\ruleName{$\desugar$-list-rest-nil}}]
      {
         \strut
      }
      {
         \exListEnd
         \desugar
         \exListEnd,
         \exNil
      }
      \and
      \inferrule*[lab={\ruleName{$\desugar$-list-rest-cons}}]
      {
         s \desugar e
         \\
         l \desugar e'
      }
      {
         (\exListNext{s}{l})
         \desugar
         \exConstr{\cCons}{e, e'}
      }
   \end{smathpar}
   \\[2mm]
   \begin{minipage}[t]{0.48\textwidth}
      {\small \flushleft \shadebox{$\gamma \desugar \gamma'$}
      \begin{smathpar}
         \inferrule*[lab={\ruleName{$\desugar$-env}}]
         {
            \seq{v} \desugar \seq{v}'
         }
         {
            \set{\seq{\bind{x}{v}}} \desugar \set{\seq{\bind{x}{v}}'}
         }
      \end{smathpar}
      }
   \end{minipage}%
   \hspace{2mm}%
   \begin{minipage}[t]{0.48\textwidth}
      {\small \flushleft \shadebox {$u \desugar v$}
         \begin{smathpar}
            \inferrule*[lab={\ruleName{$\desugar$-closure}}]
            {
                  \gamma \desugar \gamma'
                  \\
                  \seq{\mu} \desugar \seq{\sigma}
                  \\
                  \mu \desugar \sigma
            }
            {
                  \exClosure{\gamma}{\seq{\bind{x}{\mu}}}{\mu} \desugar \exClosure{\gamma'}{\seq{\bind{x}{\sigma}}}{\sigma}
            }
         \end{smathpar}
      }
   \end{minipage}
   \caption{Desugaring for terms, function definitions, environments and closures}
   \label{fig:desugar}
\end{figure}
