# Supplementary material for: Cognacy Queries over Dependence Graphs for Transparent Visualisations
Source: arXiv:2403.04403 source file (2024-10-15)
Supplement: Supplementary file 15 [file auxiliary-funcs.tex]

\begin{figure}
   {\small
   \begin{tabularx}{\textWidth}{rL{2.8cm}L{3cm}}
      &\textbfit{Auxiliary Functions}
      &
      &
   \end{tabularx}
   }
\end{figure}
