# Supplementary material for: Cognacy Queries over Dependence Graphs for Transparent Visualisations
Source: arXiv:2403.04403 source file (2024-10-15)
Supplement: Supplementary file 16 [file demands-inductive.tex]

\begin{figure}
   \begin{subfigure}{\textwidth}
      {\small
         \begin{smathpar}
            \inferrule*[
               lab={\ruleName{Leaf}}
            ]
            {
               \strut
            }
            {
               \alpha \in \opName{F}(\alpha, \exStar{F'}{\alpha})
            }
            \and
            \inferrule*[
               lab={\ruleName{interior}}
            ]
            {
               \alpha \in \opName{F}(\alpha, \exForest{\set{\seq{G}}})
            }
            {
               \alpha \in \opName{F}(\alpha, \exStar{(\exForest{\set{\seq{G}}})}{\beta})
            }
            \and
            \inferrule*[
               lab={\ruleName{branching}}
            ]
            {
               \exists G_i \in \set{\seq{G}}. \alpha \in \opName{F}(\alpha, G_i)
            }
            {
               \alpha \in \opName{F}(\alpha, \exForest{\set{\seq{G}}})
            }
         \end{smathpar}
         \vspace{2mm}
         \begin{smathpar}
            \inferrule*[
               lab={\ruleName{start}}
            ]
            {
               \alpha \in \opName{Leaves}(\bigcup_{\alpha_i \in \set{\seq{\alpha}}} \opName{F}_{G}(\alpha_i))
            }
            {
               \alpha \in \demandsR_{G}(\set{\seq{\alpha}})
            }
         \end{smathpar}
      }
   \end{subfigure}
   \caption{First attempt at rewriting the judgement for demands}
\end{figure}
