# Supplementary material for: Cognacy Queries over Dependence Graphs for Transparent Visualisations
Source: arXiv:2403.04403 source file (2024-10-15)
Supplement: Supplementary file 17 [file eval-semantics.tex]

\begin{figure}
   \begin{subfigure}{\textwidth}
   {\small \flushleft \shadebox{$\gamma, e, G, G_{1} \evalS v, G_{2}$}
      \begin{smathpar}
      \inferrule*[
         lab={\ruleName{$\evalS$-var}},
         right={$\gamma = \gamma' \cons \bind{x}{v}$}
      ]
      {
         \strut
      }
      {
         \gamma, x, G, G_{1} \evalS v, G_{1} 
      }
      \and
      \inferrule*[
         lab={\ruleName{$\evalS$-int}},
         right={$\alpha \notin \dom{G_{1}}$},
      ]
      {
         \strut
      }
      {
         \gamma, n, G, G_{1} \evalS n_{\alpha \mapsto G}, G_{1} \cdot \set{\alpha \mapsto G}
      }
      \and
      \inferrule*[
         lab={\ruleName{$\evalS$-function}},
         right={$\alpha \notin \dom{G_{1}}$},
      ]
      {
         \strut
      }
      {
         \gamma, \exFun{\sigma}, G, G_{1} \evalS \exClosure{\gamma}{\emptyset}{\sigma}_{\alpha \mapsto G}, G_{1} \cdot \set{\alpha \mapsto G}
      }
      \and
      \inferrule*[
         lab={\ruleName{$\evalS$-record}},
         right={$\alpha \notin \dom{G_{2}}$},
      ]
      {
         \gamma, \seq{e}, G, G_{1} \evalS \seq{v}, G_{2}
      }
      {
         \gamma, \exRecord{\seq{\bind{x}{e}}}, G, G_{1} \evalS \exRecord{\seq{\bind{x}{v}}}_{\alpha}, G_{2} \cdot (\alpha \mapsto G)
      }
      \and
      \inferrule*[
         lab={\ruleName{$\evalS$-constr}},
         right={$\Sigma(c) = |\seq{e}|, \alpha \notin \dom{G_{2}}$}
      ]
      {
         \gamma, \seq{e}, G, G_{1} \evalS \seq{v}, G_{2}
      }
      {
         \gamma, \exConstr{c}{\seq{e}}, G, G_{1} \evalS \exConstr{c}{\seq{v}}_{\alpha \mapsto G}, G_{2} \cdot \set{\alpha \mapsto G}
      }
      \and
      \inferrule*[
         lab={\ruleName{$\evalS$-foreign-app}}
      ]
      {
         \gamma, \seq{e}, G, G_{1} \evalS \seq{v}, G_{2}
         \\
         \hat{f}(\seq{v}) = \exPair{u}{G_{3}}
      }
      {
         \gamma, f(\seq{e}), G, G_{1} \evalS u, G_{3}
      }
      \and
      \inferrule*[
         lab={\ruleName{$\evalS$-let}}
      ]
      {
         \gamma, e, G, G_{1} \evalS v, G_{2}
         \\
         \gamma\cdot(\bind{x}{v}), e', G, G_{2} \evalS v', G_{3}
      }
      {
         \gamma, \exLet{x}{e}{e'}, G, G_{1} \evalS v', G_{3}
      }
      \and
      \inferrule*[
         lab={\ruleName{$\evalS$-let-rec}}
      ]
      {
         \gamma, \exRecord{\seq{\bind{x}{\sigma}}}, G_{1} \closeDefs \gamma', G_{2}
         \\
         \gamma \concat \gamma', e, G, G_{2} \evalS v, G_{3}
      }
      {
         \gamma, \exLetRec{\seq{\bind{x}{\sigma}}}{e}, G, G_{1} \evalS v, G_{3} 
      }
      \and
      \inferrule*[
         lab={\ruleName{$\evalS$-app}},
         width=4in,
         right={$\alpha \notin \dom{G_{4}}$},
      ]
      {
         \gamma, e, G, G_{1} \evalS \exClosure{\gamma_{1}}{\rho}{\sigma}_{\alpha \mapsto G}, G_{2}
         \\
         \gamma_{1}, \rho, G_{2} \closeDefs \gamma_2, G_{3}
         \\
         \gamma, e', G, G_{3} \evalS v', G_{4}
         \\
         v', \sigma \match \gamma_{3}, e'', G_{5}
         \\
         \gamma_{1} \concat \gamma_{2} \concat \gamma_{3}, e'', G_{4}\cdot\set{\alpha \mapsto G} \evalS u, G_{6}
      }
      {
         \gamma, \exApp{e}{e'}, G, G_{1} \evalS u, G_{6}
      }
      \end{smathpar}
   }
   \end{subfigure}
   \\[3mm]
   \begin{subfigure}{\textwidth}
   {\small \flushleft \shadebox{$\gamma, \seq{e}, G, G_{1} \evalS \seq{v}, G_{2}$}
   \begin{smathpar}
      \inferrule*[
         lab={\ruleName{$\evalS$-seq}},
         right={$n = |\seq{e}|$}
      ]
      {
         \gamma, e_i, G, G_{i-1} \evalS v_i, G_i
         \quad
         (\forall i. 1 \leq i \leq |\seq{e}|)
      }
      {
         \gamma, \seq{e}, G, G_{0} \evalS \seq{v}, G_{n}
      }
   \end{smathpar}
   }
   \end{subfigure}
   \caption{Graph Evaluation}
\end{figure}
