# Supplementary material for: Cognacy Queries over Dependence Graphs for Transparent Visualisations
Source: arXiv:2403.04403 source file (2024-10-15)
Supplement: Supplementary file 18 [file graph-syntax.tex]

\begin{figure}[h]
   {\small
   \begin{minipage}[t]{0.48\textwidth}
      \begin{tabularx}{\textwidth}{rL{2.8cm}L{3cm}}
         &\textbfit{Inductive Graphs}&
         \\
         $G ::=$
         &
         $\set{\seq{G \mapsto \alpha}}$
         &
         collection of rooted direted graphs
         \\
      \end{tabularx}
   \end{minipage}
   }
   \caption{Syntax of Graphs}
   \label{fig:graph-syntax}
\end{figure}
