# Supplementary material for: Cognacy Queries over Dependence Graphs for Transparent Visualisations
Source: arXiv:2403.04403 source file (2024-10-15)
Supplement: Supplementary file 19 [file match.tex]

\begin{figure}
   {\small \flushleft \shadebox{$\seq{v}, \kappa, \match \gamma, \kappa', G$}
   \begin{smathpar}
      \inferrule*[
         lab={\ruleName{$\match$-done}}
      ]
      {
         \strut
      }
      {
         \epsilon, e, \match \emptyset, e, \emptyset
      }
      \and
      \inferrule*[
         lab={\ruleName{$\match$-var}}
      ]
      {
         \seq{v}, \kappa \match \gamma, \tau, G_{1}
      }
      {
         v \cdot \seq{v}, x \mapsto \kappa \match \gamma \cdot (\bind{x}{v}), \tau, G_{1}
      }
      \and
      \inferrule*[
         lab={\ruleName{$\match$-constr}}
      ]
      {
         \seq{v} \concat \seq{v}', \kappa \match \gamma, e, G_{1}
      }
      {
         \exConstr{c}{\seq{v}}_{\alpha \mapsto G} \cdot \seq{v}', (c \mapsto \kappa) \cdot\set{\seq{c \mapsto \kappa}} \match \gamma, e, G_{1} \cup \set{\alpha \mapsto G}
      }
      \and
      \inferrule*[
         lab={\ruleName{$\match$-record}}
      ]
      {
         \set{\seq{\bind{y}{u}}} \subseteq \set{\seq{\bind{x}{v}}}
         \\
         \seq{u} \concat \seq{v}', \kappa \match \gamma, e, G_{1}
      }
      {
         \set{\seq{\bind{x}{v}}}_{\alpha \mapsto G} \cdot \seq{v}', \set{\seq{y}} \mapsto \kappa \match \gamma, e, G_{1} \cup \set{\alpha \mapsto G}
      }
   \end{smathpar}
   }
   \caption{Pattern Match}
\end{figure}
