# Supplementary material for: Cognacy Queries over Dependence Graphs for Transparent Visualisations
Source: arXiv:2403.04403 source file (2024-10-15)
Supplement: Supplementary file 20 [file eval.tex]

\begin{figure}
   {\small \flushleft \shadebox{$\gamma, \seq{s} \evalSugR{\seq{S}} \seq{v}$}%
   \begin{smathpar}
      \inferrule*[
         lab={\ruleName{$\evalSugS$-seq}}
      ]
      {
         \gamma, s_i \evalSugR{S_i} v_i
         \quad
         (\forall i \numleq \length{\seq{s}})
      }
      {
         \gamma, \seq{s} \evalSugR{\seq{S}} \seq{v}
      }
      \and
   \end{smathpar}}
   {\small \flushleft \shadebox{$\gamma, s \evalSugR{S} v$}%
   \begin{smathpar}
      \inferrule*[lab={\ruleName{$\evalSugS$-nonempty-list}}]
      {
         \gamma, s \evalSugR{S} v
         \\
         \gamma, l \evalSugR{S'} v'
      }
      {
         \gamma, \exList{s}{l} \evalSugR{\trList{S}{S'}} \cCons(v, v')
      }
      \and
      \inferrule*[lab={\ruleName{$\evalSugS$-list-comp-done}}]
      {
         \gamma, s \evalSugR{S} u
      }
      {
         \gamma, \exListComp{s}{\seqEmpty} \evalSugR{\seqEmpty, S} \exConstr{\cCons}{u, \exNil}
      }
      \and
      \inferrule*[
         lab={\ruleName{$\evalSugS$-list-comp-decl}}
      ]
      {
         \gamma, s' \evalSugR{S'} u'
         \\
         u', (\clause{p}{\exListComp{s}{\seq{q}}})\match \gamma', s^\dag
         \\
         (\gamma \concat \gamma'), s^\dag \evalSugR{\seq{Q},S} u
      }
      {
         \gamma, \exListComp{s}{\qualDeclaration{p}{s'} \cons \seq{q}} \evalSugR{\trQualDecl{p}{S'} \cons \seq{Q}, S} u
      }
      \and
      \inferrule*[
         lab={\ruleName{$\evalSugS$-list-comp-gen}}
      ]
      {
         (\clause{p}{\exListComp{s'}{\seq{q}}}), \exNil \orElse \mu
         \\
         \gamma, \exApp{\exApp{\varConcatMap}{\exFun{\mu}}}{s} \evalSugS u
      }
      {
         \gamma, \exListComp{s'}{\qualGenerator{p}{s} \cons \seq{q}}
         \evalSugR{\trQualGen{p}{S'}\cons\seq{Q}, S}
         u
      }
      \and
      \inferrule*[
         lab={\ruleName{$\evalSugS$-list-comp-guard-false}}
      ]
      {
         \gamma, s \evalSugR{S} \cFalse
      }
      {
         \gamma, \exListComp{s'}{\qualGuard{s} \cons \seq{q}} \evalSugR{\trQualIfFalse{S}{q}} \exNil
      }
      \and
      \inferrule*[
         lab={\ruleName{$\evalSugS$-list-comp-guard-true}},
      ]
      {
         \gamma, \exListComp{s'}{\seq{q}} \evalSugR{\seq{Q},S} v
         \\
         \gamma, s \evalSugR{S} \cTrue
      }
      {
         \gamma, \exListComp{s'}{\qualGuard{s} \cons \seq{q}} \evalSugR{\trQualIfTrue{S} \cons \seq{Q}, S} v
      }
      \and
      \inferrule*[
         lab={\ruleName{$\evalSugS$-app}},
         width=3in,
      ]
      {
         \gamma, s \evalSugR{S} \exClosure{\gamma_1}{g}{\mu}
         \\
         \gamma, s' \evalSugR{S'} v
         \\
         \gamma_1, g \closeDefs \gamma_2
         \\
         v, \mu \match \gamma_3, s^\dag
         \\
         \gamma_1 \concat \gamma_2 \concat \gamma_3, s^\dag \evalSugR{S^\dag} v'
      }
      {
         \gamma, \exApp{s}{s'} \evalSugR{\trApp{S}{S'}{p}{S^{\dag}}} v'
      }
      \and
      \inferrule*[
         lab={\ruleName{$\evalSugS$-bin-app}}
      ]
      {
         \gamma, s_1 \evalSugR{S_1} u_1
         \\
         \gamma, s_2 \evalSugR{S_2} u_2
         \\
         \gamma, \hat{\oplus}(u_1, u_2) = u
      }
      {
         \gamma, s_1 \oplus s_1 \evalSugR{\trBinApp{S_1}{S_2}{t}} u
      }
      \and
      \inferrule*[
         lab={\ruleName{$\evalSugS$-if-true}}
      ]
      {
         \gamma, s \evalSugR{S} \cTrue
         \\
         \gamma, s_1 \evalSugR{S_1} u
      }
      {
         \gamma, \exIfThenElse{s}{s_1}{s_2}\evalSugR{\exIfThenElse{S}{S_1}{s_2}} u
      }
      \and
      \inferrule*[
         lab={\ruleName{$\evalSugS$-if-false}}
      ]
      {
         \gamma, s \evalSugR{S} \cFalse
         \\
         \gamma, s_2 \evalSugR{S_2} u
      }
      {
         \gamma, \exIfThenElse{s}{s_{1}}{s_{2}}\evalSugR{\exIfThenElse{S}{s_1}{S2}} u
      }
      \and
      \inferrule*[
         lab={\ruleName{$\evalSugS$-let-rec}}
      ]
      {
         \gamma, g \closeDefs \gamma'
         \\
         \gamma \concat \gamma', s \evalSugR{S} v
      }
      {
         \gamma, \exLetRecPiecewise{g}{s} \evalSugR{\trLetRec{g}{S}} v
      }
      \and
      \inferrule*[
         lab={\ruleName{$\evalSugS$-match-as}}
      ]
      {
         \gamma, s \evalSugR{S} v
         \\
         v, \seq{\clauseUncurried{p}{s}}' \match \gamma', s_i
         \\
         \gamma \concat \gamma', s_i \evalSugR{S'} v'
      }
      {
         \gamma, \exMatch{s}{\seq{\clauseUncurried{p}{s}}'} \evalSugR{\trMatchAs{S}{\clauseUncurried{p'}{S'}}} v'
      }
      \and
      \inferrule*[
         lab={\ruleName{$\evalSugS$-enum}}
      ]
      {
         \gamma, \exApp{\exApp{\varEnumFromTo}{s_1}}{s_2} \evalSugR{\trSurfaceApp{(\trSurfaceApp{\varEnumFromTo}{S_1}{\exClosure{\varepsilon}{\varepsilon}{\clause{y}{S'}}})}{S_2}{S^{\dag}}} v
      }
      {
         \gamma, \exListEnum{s_1}{s_2} \evalSugR{\trEnum{S_1}{S_2}} v
      }
   \end{smathpar}}
   \\[3mm]
   {\small \flushleft \shadebox{$\gamma, r \evalSugS v$}
   \begin{smathpar}
      \inferrule*[
         lab={\ruleName{$\evalSugS$-list-rest-nil}}
      ]
      {
         \strut
      }
      {
         \gamma, \exListEnd \evalSugR{\trListEnd} \exNil
      }
      \and
      \inferrule*[
         lab={\ruleName{$\evalSugS$-list-rest-next}}
      ]
      {
         \gamma, s \evalSugR{S} v
         \\
         \gamma, l \evalSugR{S'} v'
      }
      {
         \gamma, (\exListNext{s}{l}) \evalSugR{\trListNext{S}{S'}} \exConstr{\cCons}{v, v'}
      }
   \end{smathpar}
   }
   \\[2mm]
   {\small\flushleft \shadebox{$\gamma, g \closeDefs \gamma'$}
      \begin{smathpar}
         \inferrule*[
%            lab={\ruleName{$\closeDefs$-surface}}
         ]
         {
            g = \seq{\bind{x}{\mu}}
            \\
            v_i = \exClosure{\gamma}{g}{\mu_i}
            \quad
            (\forall i \le \length{\seq{x}})
         }
         {
            \gamma, g \closeDefs \set{\seq{\bind{x}{v}}}
         }
      \end{smathpar}}
   \caption{Surface semantics}
   \label{fig:surface:eval}
\end{figure}
