# Supplementary material for: Cognacy Queries over Dependence Graphs for Transparent Visualisations
Source: arXiv:2403.04403 source file (2024-10-15)
Supplement: Supplementary file 21 [file match.tex]

\begin{figure}
   {\small \flushleft \shadebox{$v, \mu \match \gamma, s$}
   \begin{smathpar}
      \inferrule*[
         lab={\ruleName{$\match$-fun}}
      ]
      {
         v, \seq{(p, \clause{\pi}{s})} \match \gamma, s
      }
      {
         v, (\seq{\clause{p \cons \pi}{s}})
         \match
         \gamma, s
      }
   \end{smathpar}}
   \\[3mm]
   {\small \flushleft \shadebox{$\seq{v}, \seq{k} \match \gamma, s$}
   \begin{smathpar}
      \inferrule*[
         lab={\ruleName{$\match$-done-uncurried}}
      ]
      {
         \strut
      }
      {
         \seqEmpty, (\seqEmpty, \clause{\seqEmpty}{s}) \match \envEmpty, s
      }
      \and
      \inferrule*[
         lab={\ruleName{$\match$-done-curried}}
      ]
      {
         \strut
      }
      {
         \seqEmpty,
         \seqRange{(\seqEmpty, \clause{p_1 \cons \pi_1}{s_1})}{(\seqEmpty, \clause{p_j \cons \pi_j}{s_j})}
         \match
         \envEmpty, \exFun{(\seq{\clause{p \cons \pi}{s}})}
      }
      \and
      \inferrule*[
         lab={\ruleName{$\match$-var}}
      ]
      {
         \seq{v}, \seq{k} \match \gamma, s
      }
      {
         v \cons \seq{v}, \seqRange{(\pattVar{x} \clauseWith{\cons} k_1)}{(\pattVar{x} \clauseWith{\cons} k_j)}
         \match
         \set{\bind{x}{v}} \disjunion \gamma, s
      }
      \and
      \inferrule*[
         lab={\ruleName{$\match$-record}}
      ]
      {
         \exRecord{\seq{\bind{y}{u}}} \subseteq \exRecord{\seq{\bind{x}{v}}}
         \\
         \seq{u} \concat \seq{v}',
         (\seqRange{\seq{p_1}}{\seq{p_j}})
         \clauseWith{\concat} \seq{k}
         \match \gamma, s
      }
      {
         \exRecord{\seq{\bind{x}{v}}} \cons \seq{v}',
         (\seqRange{\pattRecord{\seq{\bind{y}{p_1}}}}{\pattRecord{\seq{\bind{y}{p_j}}}})
         \clauseWith{\cons}
         \seq{k}
         \match
         \gamma, s
      }
      \and
      \inferrule*[
         lab={\ruleName{$\match$-constr}}
      ]
      {
         \seq{v} \concat \seq{v}',
         (\pi_i \clauseWith{\concat} k_i \mid c_i = c)
         \match \gamma, s
      }
      {
         \exConstr{c}{\seq{v}} \cons \seq{v}',
         \seq{\pattConstr{c}{\pi} \clauseWith{\cons} k}
         \match
         \gamma, s
      }
   \end{smathpar}}
   \caption{Surface semantics: pattern matching}
\end{figure}
