# Supplementary material for: Cognacy Queries over Dependence Graphs for Transparent Visualisations
Source: arXiv:2403.04403 source file (2024-10-15)
Supplement: Supplementary file 22 [file syntax.tex]

\begin{figure}
   {\small
   \begin{minipage}[t]{0.48\textwidth}
   \begin{tabularx}{\textwidth}{rL{2.8cm}L{3cm}}
      &\textbfit{Surface term}&
      \lowlight{$\SExpr\;\Gamma\;A$}
      \\
      $s ::=$
      &
      $\exBinaryApp{s}{\oplus}{s'}$
      &
      binary application
      \\
      &
      $\exLetRecPiecewise{g}{s}$
      &
      recursive functions
      \\
      &
      $\exIfThenElse{s}{s_1}{s_2}$
      &
      if
      \\
      &
      $\exMatch{s}{\seq{\clauseUncurried{p}{s}}'}$
      &
      match
      \\
      &
      $\exList{s}{l}$
      &
      non-empty list
      \\
      &
      $\exListEnum{s}{s'}$
      &
      list enum
      \\
      &
      $\exListComp{s}{\seq{q}}$
      &
      list comprehension
      \\
      &
      $\exDo{\seq{d}}$
      &
      do
      \\
      &
      $\exFun{\mu}$
      &
      lambda
      \\[2mm]
      &\textbfit{List rest}&
      \lowlight{$\ListRest\;\Gamma\;A$}
      \\
      $l ::=$
      &
      $\exListEnd$
      &
      end
      \\
      &
      $\exListNext{s}{l}$
      &
      cons
      \\[2mm]
      &\textbfit{Recursive functions}&
      \\
      $g ::=$
      &
      $\seq{\bind{x}{\mu}}$
      &
      \\[2mm]
      &\textbfit{Function definition}&
      \\
      $\mu ::=$
      &
      $\seq{\clause{\pi}{s}}$
      &
      \\[8mm]
      \end{tabularx}
   \end{minipage}%
   \begin{minipage}[t]{0.5\textwidth}
      \begin{tabularx}{\textwidth}{rL{2.8cm}L{2.9cm}}
      &\textbfit{Pattern sequence}&
      \\
      $\pi ::=$
      &
      $\seq{p}$
      &
      \\[2mm]
      &\textbfit{Pattern}&
      \lowlight{$\Patt\;A\;\Gamma$}
      \\
      $p ::=$
      &
      $\pattVar{x}$
      &
      variable
      \\
      &
      $\pattRecord{\seq{\bind{x}{p}}}$
      &
      record
      \\
      &
      $\pattConstr{c}{\pi}$
      &
      constructor
      \\
      &
      $\pattList{p}{o}$
      &
      non-empty list
      \\[2mm]
      &\textbfit{List rest pattern}&
      \lowlight{$\ListRestPatt\;A\;\Gamma$}
      \\
      $o ::=$
      &
      $\pattListEnd$
      &
      end
      \\
      &
      $\pattListNext{p}{o}$
      &
      cons
      \\[2mm]
      &\textbfit{Qualifier}&
      \\
      $q ::=$
      &
      $\qualGuard{s}$
      &
      guard
      \\
      &
      $\qualDeclaration{p}{s}$
      &
      declaration
      \\
      &
      $\qualGenerator{p}{s}$
      &
      generator
      \\[2mm]
      &\textbfit{Surface value}&
      \lowlight{$\SVal{A}$}
      \\
      $v, u ::=$
      &
      $\dots$
      &
      $\dots$
      \\
      &
      $\exClosure{\gamma}{g}{\mu}$
      &
      closure
      \\[8mm]
      \end{tabularx}
   \end{minipage}
   }
   \caption{Syntax of surface terms}
\end{figure}
