# Supplementary material for: Cognacy Queries over Dependence Graphs for Transparent Visualisations
Source: arXiv:2403.04403 source file (2024-10-15)
Supplement: Supplementary file 23 [file typing.tex]

\begin{figure}
   \flushleft \shadebox{$\Gamma \vdash g: \Delta$}
   \begin{smathpar}
      \inferrule*[right={
         \textnormal{$\Delta = \seq{\bind{x}{\tyFun{A}{B}}}$}
      }]
      {
         \Gamma \concat \Delta \vdash \seq{\mu: \tyFun{A}{B}}
      }
      {
         \Gamma \vdash \seq{\bind{x}{\mu}}: \Delta
      }
   \end{smathpar}

   \vspace{5pt}
   \flushleft \shadebox{$\Gamma \vdash s: A$}
   \begin{smathpar}
      \inferrule*[right={$\primOp: \tyForeign{(A,A')}{B} \in \Gamma$}]
      {
         \Gamma \vdash s: A
         \\
         \Gamma \vdash s': A'
      }
      {
         \Gamma \vdash \exBinaryApp{s}{\oplus}{s'}: B
      }
      \and
      \inferrule*[]
      {
         \Gamma \vdash \mu: \tyFun{A}{B}
      }
      {
         \Gamma \vdash \exApp{\lambda}{\mu}: \tyFun{A}{B}
      }
      \and
      \inferrule*
      {
         \Gamma \vdash g: \Delta
         \\
         \Gamma \concat \Delta \vdash s: A
      }
      {
         \Gamma \vdash \exLetRec{g}{s}: A
      }
      \and
      \inferrule*
      {
         \Gamma \vdash s: \tyBool
         \\
         \Gamma \vdash s_1: A
         \\
         \Gamma \vdash s_2: A
      }
      {
         \Gamma \vdash \exIfThenElse{s}{s_1}{s_2}: A
      }
      \and
      \inferrule*
      {
         \Gamma \vdash s: A
         \\
         \Gamma \vdash \mu: \tyFun{A}{B}
      }
      {
         \Gamma \vdash \exMatch{s}{\mu}: B
      }
      \and
      \inferrule*
      {
         p: A \dashv \Gamma'
         \\
         \Gamma \vdash s: A
         \\
         \Gamma \concat \Gamma' \vdash s': B
      }
      {
         \Gamma \vdash \exLet{p}{s}{s'}: B
      }
      \and
      \inferrule*
      {
         \Gamma \vdash s : A
         \\
         \Gamma \vdash r : \tyList{A}
      }
      {
         \Gamma \vdash \exList{s}{r} : \tyList{A}
      }
      \and
      \inferrule*
      {
         \Gamma \vdash s: \tyInt
         \\
         \Gamma \vdash s': \tyInt
      }
      {
         \Gamma \vdash \exListEnum{s}{s'}: \tyList{\tyInt}
      }
      \and
      \inferrule*
      {
         \Gamma \vdash \seq{q} \dashv \Delta
         \\
         \Gamma \concat \Delta \vdash s: A
      }
      {
         \Gamma \vdash \exListComp{s}{\seq{q}}: \tyList{A}
      }
      \end{smathpar}

      % List rest
      \vspace{5pt}
      \flushleft \shadebox{$\Gamma \vdash r: \tyList{A}$}
      \begin{smathpar}
      \inferrule*
      {
         \strut
      }
      {
         \Gamma \vdash \exListEnd : \tyList{A}
      }
      \and
      \inferrule*
      {
         \Gamma \vdash s : A
         \\
         \Gamma \vdash r : \tyList{A}
      }
      {
         \Gamma \vdash (\exListNext{s}{r}) : \tyList{A}
      }
      \end{smathpar}

      \vspace{0.1em}
      %% Qualifiers

      \flushleft \shadebox{$\Gamma \vdash \seq{q} \dashv \Delta $}
      \begin{smathpar}
      \inferrule*
      {
         \strut
      }
      {
         \Gamma \vdash \seqEmpty \dashv \seqEmpty
      }
      \and
      \inferrule*
      {
         \Gamma \vdash s: \tyBool
      }
      {
         \Gamma \vdash \qualGuard{s} \dashv \seqEmpty
      }
      \and
      \inferrule*
      {
         \Gamma \vdash s: \tyList{A}
         \\
         p: A \dashv \Delta
      }
      {
         \Gamma \vdash \qualGenerator{p}{s} \dashv \Delta
      }
      \and
      \inferrule*
      {
         \Gamma \vdash s: A
         \\
         p: A \dashv \Delta
      }
      {
         \Gamma \vdash \qualDeclaration{p}{s} \dashv \Delta
      }
      \and
      \inferrule*[
         right={$\seq{q} \neq \seqEmpty$}
      ]
      {
         \Gamma \vdash q \dashv \Gamma'
         \\
         \Gamma \concat \Gamma' \vdash \seq{q} \dashv \Delta
      }
      {
         \Gamma \vdash q \cons \seq{q} \dashv \Delta
      }
   \end{smathpar}
   \caption{Typing rules for surface terms (additional forms only) and qualifiers}
   \label{fig:surface-language:typing-term}
   \end{figure}
