# Supplementary material for: Cognacy Queries over Dependence Graphs for Transparent Visualisations
Source: arXiv:2403.04403 source file (2024-10-15)
Supplement: Supplementary file 24 [file clauses.tex]

\begin{figure}

   %% Patterns
   \flushleft \shadebox{$\seq{p: A} \dashv \Gamma $}
   \begin{smathpar}
      \inferrule*[
         right={$\length{\seq{p}} = n$}
      ]
      {
         p_i: A_i \dashv \Gamma_i
         \quad
         (\forall i \numleq n)
      }
      {
         \seq{p: A} \dashv \seqRangeOp{\Gamma_1}{\Gamma_n}{\concat}
      }
   \end{smathpar}
   \vspace{3mm}

   \flushleft \shadebox{$p: A \dashv \Gamma $}
   \begin{smathpar}
      \inferrule*
      {
         \strut
      }
      {
         \pattVar{x}: A \dashv \set{\bind{x}{A}}
      }
      \and
      \inferrule*[
      ]
      {
         \seq{p: A} \dashv \Gamma
      }
      {
         \pattRec{\seq{\bind{x}{p}}}: \tyRec{\seq{\bind{x}{A}}} \dashv \Gamma
      }
      \and
      \inferrule*[
         right={$\datatype{c} = \tyForeign{\seq{A}}{D}$}
      ]
      {
         \seq{p: A} \dashv \Gamma
      }
      {
         \pattConstr{c}{\seq{p}}: \tyData{D} \dashv \Gamma
      }
      \and
      \inferrule*
      {
         p: A \dashv \Gamma
         \\
         o: \tyList{A} \dashv \Gamma'
      }
      {
         \pattList{p}{o} : \tyList{A} \dashv \Gamma \concat \Gamma'
      }
   \end{smathpar}
   \vspace{3mm}

   \flushleft \shadebox{$o: \tyList{A} \dashv \Gamma $}
   \begin{smathpar}
      \inferrule*
      {
         \strut
      }
      {
         \pattListEnd : \tyList{A} \dashv \seqEmpty
      }
      \and
      \inferrule*
      {
         p : A \dashv \Gamma
         \\
         o : \tyList{A} \dashv \Gamma'
      }
      {
         (\pattListNext{p}{o}) : \tyList{A} \dashv \Gamma \concat \Gamma'
      }
      \end{smathpar}
      \vspace{3mm}

      \flushleft \shadebox{$\Gamma \vdash \mu: \tyFun{A}{B}$}
      \begin{smathpar}
      \inferrule*
      {
         p: A \dashv \Gamma'
         \\
         \Gamma \concat \Gamma' \vdash s: B
      }
      {
         \Gamma \vdash \clauseUncurried{p}{s} : \tyFun{A}{B}
      }
      \and
      \inferrule*[
         right={$\seq{p} \neq \seqEmpty$}
      ]
      {
         p : A \dashv \Gamma'
         \\
         \Gamma \concat \Gamma' \vdash \clause{\seq{p}'}{s} : \tyFun{A'}{B}
      }
      {
         \Gamma \vdash \clauseUncurried{(p \cdot \seq{p})}{s} : \tyFun{A}{\tyFun{A'}{B}}
      }
      \and
      \inferrule*[
      ]
      {
         \Gamma \vdash c: \tyFun{A}{B}
         \\
         \compatPatt{c}{\mu}
         \\
         \Gamma \vdash \mu : \tyFun{A}{B}
      }
      {
         \Gamma \vdash c \cdot \mu: \tyFun{A}{B}
      }
   \end{smathpar}

\caption{Typing rules for patterns and clauses}
\label{fig:surface-language:typing-pattern}
\end{figure}
