# Supplementary material for: Cognacy Queries over Dependence Graphs for Transparent Visualisations
Source: arXiv:2403.04403 source file (2024-10-15)
Supplement: Supplementary file 25 [file disjoint-patts.tex]

\begin{figure}
   \flushleft \shadebox{$\compatPatt{p}{p'}$}
   \begin{smathpar}
      \inferrule*[
         lab={\ruleName{$\compatPatt{}{}$-constr-neq}}
      ]
      {
         \exVar{c} \neq \exVar{c'}
      }
      {
         \compatPatt{\exConstr{c}{\seq{p}}}{\exConstr{c'}{\seq{p}'}}
      }
      \and
      \inferrule*[
         lab={\ruleName{$\compatPatt{}{}$-constr-eq}}
      ]
      {
         \compatPatt{\seq{p}}{\seq{p}'}
      }
      {
         \compatPatt{\exConstr{c}{\seq{p}}}{\exConstr{c}{\seq{p}'}}
      }
      \and
      \inferrule*[
         lab={\ruleName{$\compatPatt{}{}$-record}}
      ]
      {
         \compatPatt{\seq{p}}{\seq{p}'}
      }
      {
         \compatPatt{\exRecord{\seq{\bind{\exVar{x}}{p}}}}{\exRecord{\seq{\bind{\exVar{x}}{p}}'}}
      }
   \end{smathpar}
   {\flushleft \shadebox{$\compatPatt{\seq{p}}{\seq{p}'}$}
   \begin{smathpar}
      \inferrule*[
         lab={\ruleName{$\compatPattSym$-head}}
      ]
      {
         \compatPatt{p}{p'}
      }
      {
         \compatPatt{p\cdot\seq{p}}{p'\cdot\seq{p}'}
      }
      \and
      \inferrule*[
         lab={\ruleName{$\compatPattSym$-tail}}
      ]
      {
         \compatPatt{\seq{p}}{\seq{p}'}
      }
      {
         \compatPatt{p\cdot\seq{p}}{p\cdot\seq{p}'}
      }
   \end{smathpar}}
   {\flushleft \shadebox{$\compatPatt{c}{\mu}$}
   \begin{smathpar}
      \inferrule*[]
      {
         \exists i.(\compatPatt{p_i}{p_i'})
         \textit{ and }
         \forall j < i.\; p_j = p'_j
      }
      {
         \compatPatt{(\clause{\seq{p}}{s})}{(\clause{\seq{p}'}{s'})}
      }
      \and
      \inferrule*[
         right={$\mu \neq \seqEmpty$}
      ]
      {
         \compatPatt{c}{c'}
         \\
         \compatPatt{c}{\mu}
      }
      {
         \compatPatt{c}({c'\cdot\mu)}
      }
   \end{smathpar}}
   \caption{Disjointness of patterns and clauses}
\end{figure}
