# Supplementary material for: Cognacy Queries over Dependence Graphs for Transparent Visualisations
Source: arXiv:2403.04403 source file (2024-10-15)
Supplement: Supplementary file 26 [file closedefs-eq.tex]

\begin{proof}
   \small
   \begin{flalign}
      &
      \gamma_1 \desugar \gamma_2
      &
      \text{suppose}
      \notag
      \\
      &
      \seq{\mu} \desugar \seq{\sigma}
      &
      \text{suppose}
      \notag
      \\
      &
      \derivation{\derivationWidth}{
         \begin{smathpar}
            \inferrule*[
%               left={\ruleName{$\closeDefs$-surface}}
            ]
            {
               g = \seq{\bind{x}{\mu}}
               \\
               v_i = \exClosure{\gamma_1}{g}{\mu_i}
               \quad
               (\forall i \le \length{\seq{x}})
            }
            {
               \gamma_1, g \closeDefs \set{\seq{\bind{x}{v}}}
            }
         \end{smathpar}
      }
      &
      \text{suppose}
      \notag
      \\
      &
      \derivation{\derivationWidth}{
         \begin{smathpar}
            \inferrule*[
%               left={\ruleName{$\closeDefs$-core}}
            ]
            {
               \rho = \set{\seq{\bind{x}{\sigma}}}
               \\
               v'_i = \exClosure{\gamma_2}{\rho}{\sigma_i}
               \quad
               (\forall i \numleq \length{\seq{x}})
            }
            {
               \gamma_2, \rho
               \closeDefs
               \set{\seq{\bind{x}{v}}'}
            }
         \end{smathpar}
      }
      &
      \text{suppose}
      \notag
      \\
      &
      \qedLocal
      \derivation{\derivationWidth}{
         \begin{smathpar}
            \inferrule*
            [
               left={\ruleName{$\desugar$-env}}
            ]
            {
               \inferrule*
               [
                  left={\ruleName{$\desugar$-closure}},
                  right={$\forall i. \numleq \length{\seq{x}}$}
               ]
               {
                  \gamma_1 \desugar \gamma_2
                  \\
                  \seq{\mu} \desugar \seq{\sigma}
                  \\
                  \mu_i \desugar \sigma_i
               }
               {
                  v_i = \exClosure{\gamma_1}{g}{\mu_i} \desugar \exClosure{\gamma_2}{\rho}{\sigma_i}
               }
            }
            {
               \set{\seq{\bind{\exVar{x}}{v}}} \desugar \set{\seq{\bind{\exVar{x}}{v}}'}
            }
         \end{smathpar}
      }
      &
      \notag
   \end{flalign}
\end{proof}
