# Supplementary material for: Cognacy Queries over Dependence Graphs for Transparent Visualisations
Source: arXiv:2403.04403 source file (2024-10-15)
Supplement: Supplementary file 27 [file match-seq-eq.tex]

We prove part (2) simultaneously with the $\implies$ direction of part (1) by induction on surface-language
$\match$ derivation. We omit the proof of the $\impliedby$ direction of part (1), which is similar.

\begin{proof}
\small
\begin{flalign}
   &
   \seq{u} \desugar \seq{v}
   &
   \text{suppose}
   \locallabel{us-desugar-vs}
   \\
   &
   \seq{k} \desugar \kappa
   &
   \text{suppose}
   \notag
   \\
   &
   \seq{u}, \seq{k} \match \gamma, s
   &
   \text{suppose}
   \notag
   \\
   \intertext{\crossrule}
   %%%%%%%%%%%%%%%%%%%%%%%%%%%
   &
   \caseDerivation{\derivationWidth}{
      \begin{smathpar}
         \inferrule*[
            lab={\ruleName{$\match$-done-uncurried}}
          ]
          {
             \strut
          }
          {
             \Lowlight{\seq{u} =\;}\seqEmpty,
             \Lowlight{\seq{k} =\;}(\seqEmpty, \clause{\seqEmpty}{s})
             \match \envEmpty\Lowlight{\;= \gamma}, s
          }
      \end{smathpar}
   }
   &
   \notag
   \\
   &
   \derivation{\derivationWidth}{
      \begin{smathpar}
         \inferrule*[
            lab={\ruleName{$\desugar$-clauses-done}}
         ]
         {
            s \desugar e
         }
         {
            \Lowlight{\seq{k} =\;}(\seqEmpty, \clause{\seqEmpty}{s}) \desugar e\Lowlight{\;=\kappa}
         }
      \end{smathpar}
   }
   &
   \text{inversion}
   \locallabel{done-uncurried-inversion}
   \\
   &
   \seq{v} = \seqEmpty
   &
   \text{(\localref{us-desugar-vs})}
   \notag
   \\
   &
   \qedLocal
   \derivation{\derivationWidth}{
      \begin{smathpar}
         \inferrule*[
            lab={\ruleName{$\match$-done}}
         ]
         {
            \strut
         }
         {
            \Lowlight{\seq{v} =\;}\seqEmpty,
            \Lowlight{\kappa =\;}e \match \envEmpty, e
         }
      \end{smathpar}
   }
   &
   \notag
   \\
   &
   \qedLocal
   \envEmpty \desugar \envEmpty\text{ and }s \desugar e
   &
   \text{(\localref{done-uncurried-inversion})}
   \notag
   \\
   \intertext{\crossrule}
   %%%%%%%%%%%%%%%%%%%%%%%%%%%
   &
   \caseDerivation{\derivationWidth}{
      \begin{smathpar}
         \inferrule*[
            left={\ruleName{$\match$-done-curried}}
          ]
          {
             \strut
          }
          {
             \Lowlight{\seq{u} =\;}
             \seqEmpty, (\seqRange{(\seqEmpty, \clause{p_1 \cons \pi_1}{s_1})}
                                  {(\seqEmpty, \clause{p_j \cons \pi_j}{s_j})}) \\
             \match
             \envEmpty\Lowlight{\;=\gamma}, \exFun{(\seq{\clause{p \cons \pi}{s}})}\Lowlight{\;=s}
          }
       \end{smathpar}
   }
   &
   \notag
   \\
   &
   \derivation{\derivationWidth}{
      \begin{smathpar}
         \inferrule*[
            left={\ruleName{$\desugar$-clauses-curried}}
         ]
         {
            \seq{(p, \clause{\pi}{s})}
            \desugar
            \sigma
         }
         {
            \seqRange{(\seqEmpty, \clause{p_1 \cons \pi_1}{s_1})}
                     {(\seqEmpty, \clause{p_j \cons \pi_j}{s_j})}
            \desugar
            \exFun{\sigma}\Lowlight{\;=\kappa}
         }
       \end{smathpar}
   }
   &
   \text{inversion}
   \locallabel{done-curried-inversion}
   \\
   &
   \seq{v} = \seqEmpty
   &
   \text{(\localref{us-desugar-vs})}
   \notag
   \\
   &
   \qedLocal
   \derivation{\derivationWidth}{
      \begin{smathpar}
         \inferrule*[
            left={\ruleName{$\match$-done}}
         ]
         {
            \strut
         }
         {
            \Lowlight{\seq{v} =\;}
            \seqEmpty, \exFun{\sigma} \match \envEmpty, \exFun{\sigma}
         }
      \end{smathpar}
   }
   &
   \notag
   \\
   &
   \qedLocal
   \envEmpty \desugar \envEmpty
   &
   \notag
   \\
   &
   \qedLocal
   \derivation{\derivationWidth}{
      \begin{smathpar}
         \inferrule*[left={\ruleName{$\desugar$-lambda}}]
         {
            \inferrule*[
               left={\ruleName{$\desugar$-fun}}
            ]
            {
               \seq{(p, \clause{\pi}{s})}
               \desugar \sigma
            }
            {
               \seq{\clause{p \cons \pi}{s}}
               \desugar
               \sigma
            }
         }
         {
            \exFun{(\seq{\clause{p \cons \pi}{s}})} \desugar \exFun{\sigma}
         }
      \end{smathpar}
   }
   &
   \text{(\localref{done-curried-inversion})}
   \notag
   \\
   \intertext{\crossrule}
   %%%%%%%%%%%%%%%%%%%%%%%%%%%
   &
   \caseDerivation{\derivationWidth}{
      \begin{smathpar}
         \inferrule*[
            left={\ruleName{$\match$-var}}
          ]
          {
             \seq{u}', \seq{k}
             \match \gamma^\dagger, s
          }
          {
             \Lowlight{\seq{u} =\;}
             u \cons \seq{u}',
             \seqRange{(\pattVar{x} \clauseWith{\cons} k_1)}{(\pattVar{x} \clauseWith{\cons} k_j)}
             \match
             \set{\bind{x}{v}} \disjunion \gamma^\dagger\Lowlight{\;= \gamma}, s
          }
       \end{smathpar}
   }
   &
   \notag
   \\
   &
   \derivation{\derivationWidth}{
      \begin{smathpar}
         \inferrule*[
            left={\ruleName{$\desugar$-clauses-var}}
         ]
         {
            \seq{k} \desugar \kappa'
         }
         {
            \seqRange{(\pattVar{x} \clauseWith{\cons} k_1)}{(\pattVar{x} \clauseWith{\cons} k_j)}
            \desugar
            (\elimVar{x}{\kappa'})\Lowlight{\,= \kappa}
         }
      \end{smathpar}
   }
   &
   \text{inversion}
   \notag
   \\
   &
   \seq{v} = v \cons \seq{v}'\text{ with }u \desugar v\text{ and }\seq{u}' \desugar \seq{v}'
   \quad
   (\exists v, \seq{v}')
   &
   \text{(\localref{us-desugar-vs})}
   \notag
   \\
   &
   \seq{v}', \kappa' \match \gamma^\ddagger, e
   \textit{ with }\gamma^\dagger \desugar \gamma^\ddagger
   \textit{ and }s \desugar e
   \quad
   (\exists\gamma^\ddagger, e)
   &
   \text{IH}
   \notag
   \\
   &
   \qedLocal
   \derivation{\derivationWidth}{
      \begin{smathpar}
         \inferrule*[left={\ruleName{$\match$-var}}]
         {
            \seq{v}', \kappa' \match \gamma^\ddagger, e
         }
         {
            v \cons \seq{v}, \elimVar{x}{\kappa'} \match \set{\bind{x}{v}} \disjunion \gamma^\ddagger, e
         }
      \end{smathpar}
   }
   &
   \notag
   \\
   &
   \qedLocal
   \set{\bind{x}{u}} \disjunion \gamma^\dagger
   \desugar
   \set{\bind{x}{v}} \disjunion \gamma^\ddagger
   \textit{ and }
   s \desugar e
   &
   \text{($u \desugar v$)}
   \notag
   \\
   \intertext{\crossrule}
   %%%%%%%%%%%%%%%%%%%%%%%%%%%
   &
   \caseDerivation{\derivationWidth}{
      \begin{smathpar}
         \inferrule*[
            left={\ruleName{$\match$-record}}
         ]
         {
            \exRecord{\seq{\bind{y}{u}}^\ddagger} \subseteq \exRecord{\seq{\bind{x}{u}}^\dagger}
            \\
            \seq{u}^\ddagger \concat \seq{u}',
            (\seqRange{\seq{p_1}}{\seq{p_j}}) \clauseWith{\concat} \seq{k}
            \match \gamma, s
         }
         {
            \Lowlight{\seq{u} =\;}
            \exRecord{\seq{\bind{x}{u}}^\dagger} \cons \seq{u}',
            (\seqRange{\pattRecord{\seq{\bind{y}{p_1}}}}
                      {\pattRecord{\seq{\bind{y}{p_j}}}}) \clauseWith{\cons} \seq{k}
            \match
            \gamma, s
         }
      \end{smathpar}
   }
   &
   \notag
   \\
   &
   \derivation{\derivationWidth}{
      \begin{smathpar}
         \inferrule*[
            left={\ruleName{$\desugar$-clauses-record}}
         ]
         {
            (\seqRange{\seq{p_1}}{\seq{p_j}}) \clauseWith{\concat} \seq{k} \desugar \kappa'
         }
         {
            (\seqRange{\pattRecord{\seq{\bind{x}{p_1}}}}{\pattRecord{\seq{\bind{x}{p_j}}}})
            \clauseWith{\cons} \seq{k}
            \desugar
            (\elimRecord{\seq{x}}{\kappa'})
            \Lowlight{\;= \kappa}
         }
      \end{smathpar}
   }
   &
   \text{inversion}
   \notag
   \\
   &
   \seq{v} = \exRec{\seq{\bind{x}{v}}^\dagger} \cons \seq{v}'
   \textit{ with }
   \seq{u}^\dagger \desugar \seq{v}^\dagger
   \textit{ and }
   \seq{u}' \desugar \seq{v}'
   \quad
   (\exists \seq{v}^\dagger, \seq{v}')
   &
   \text{(\localref{us-desugar-vs})}
   \notag
   \\
   &
   \exRec{\seq{\bind{y}{v}}^\ddagger} \subseteq \exRec{\seq{\bind{x}{v}}^\dagger}
   \textit{ with }
   \seq{u}^\ddagger \desugar \seq{v}^\ddagger
   \quad
   (\exists \seq{v}^\ddagger)
   &
   \notag
   \\
   &
   \seq{u}^\ddagger \concat \seq{u}' \desugar \seq{v}^\ddagger \concat \seq{v}'
   &
   \notag
   \\
   &
   \seq{v}^\ddagger \concat \seq{v}', \kappa \match \gamma', e
   \textit{ with }
   \gamma \desugar \gamma'\textit{ and }s \desugar e
   \quad
   (\exists \gamma', e)
   &
   \text{IH}
   \notag
   \\
   &
   \qedLocal
   \derivation{\derivationWidth}{
      \begin{smathpar}
         \inferrule*[
            left={\ruleName{$\match$-record}}
         ]
         {
            \seq{v}^\ddagger \concat \seq{v}', \kappa \match \gamma', e
            \\
            \exRec{\seq{\bind{y}{v}}^\ddagger} \subseteq \exRec{\seq{\bind{x}{v}}^\dagger}
         }
         {
            \Lowlight{\seq{v} =\;}\exRec{\seq{\bind{x}{v}}^\dagger} \cons \seq{v}',
            \elimRecord{\seq{y}}{\kappa}
            \match
            \gamma', e
         }
      \end{smathpar}
   }
   &
   \notag
   \\
   \intertext{\crossrule}
   %%%%%%%%%%%%%%%%%%%%%%%%%%%
   &
   \caseDerivation{\derivationWidth}{
      \begin{smathpar}
         \inferrule*[
            left={\ruleName{$\match$-constr}}
         ]
         {
            \seq{u}^\dagger \concat \seq{u}',
            (\pi_i \clauseWith{\concat} k_i \mid c_i = c)
            \match \gamma, s
         }
         {
            \Lowlight{\seq{u} =\;}
            \exConstr{c}{\seq{u}^\dagger} \cons \seq{u}',
            \seq{(\pattConstr{c}{\pi} \clauseWith{\cons} k)}
            \match
            \gamma, s
         }
      \end{smathpar}
   }
   &
   \notag
   \\
   &
   \derivation{\derivationWidth}{
      \begin{smathpar}
         \inferrule*[
            left={\ruleName{$\desugar$-clauses-constr}}
         ]
         {
            (\pi_i \clauseWith{\concat} k_i \mid c_i = c') \desugar \kappa_{c'}
            \\
            \datatype{c'} = D
            \quad
            (\forall c' \in \set{\seq{c}})
         }
         {
            \seq{\pattConstr{c}{\pi} \clauseWith{\cons} k}
            \desugar
            \elimConstr{\elimBind{c'}{\kappa_{c'}} \mid c' \in \set{\seq{c}}}
            \Lowlight{\;= \kappa}
         }
      \end{smathpar}
   }
   &
   \text{inversion}
   \locallabel{constr-inversion}
   \\
   &
   \seq{v} = \exConstr{c}{\seq{v}^\dagger} \cons \seq{v}'
   \textit{ with }
   \seq{u}^\dagger \desugar \seq{v}^\dagger
   \textit{ and }
   \seq{u}' \desugar \seq{v}'
   \quad
   (\exists \seq{v}^\dagger, \seq{v}')
   &
   \text{(\localref{us-desugar-vs})}
   \notag
   \\
   &
   \seq{u}^\dagger \concat \seq{u}' \desugar \seq{v}^\dagger \concat \seq{v}'
   &
   \notag
   \\
   &
   (\pi_i \clauseWith{\concat} k_i \mid c_i = c) \desugar \kappa_{c}
   &
   \text{(\localref{constr-inversion})}
   \notag
   \\
   &
   \seq{v}^\dagger \concat \seq{v}', \kappa_c \match \gamma', e
   \textit{ with }
   \gamma' \desugar \gamma
   \textit{ and }
   s \desugar e
   \quad
   (\exists \gamma', e)
   &
   \text{IH}
   \notag
   \\
   &
   \sigma \eqdef
   \kappa \setminus \set{\elimBind{c}{\kappa_c}}
   &
   \notag
   \\
   &
   \qedLocal
   \derivation{\derivationWidth}{
      \begin{smathpar}
         \inferrule*[lab={\ruleName{$\match$-constr}}]
         {
            \seq{v}^\dagger \concat \seq{v}', \kappa_c \match \gamma', e
         }
         {
            \Lowlight{\seq{v} =\;}
            \exConstr{c}{\seq{v}^\dagger} \cons \seq{v}', \Lowlight{\kappa =\;}((\elimBind{c}{\kappa_c}) \cons \sigma)
            \match
            \gamma', e
         }
      \end{smathpar}
   }
   &
   \notag
\end{flalign}
\end{proof}
