# Supplementary material for: Cognacy Queries over Dependence Graphs for Transparent Visualisations
Source: arXiv:2403.04403 source file (2024-10-15)
Supplement: Supplementary file 28 [file semantics-eq-1.tex]

Case analysis on surface $\evalS$ derivation and induction on $\desugar$ derivation.
\begin{proof}
\small
\begin{flalign}
   &
   s_0 \desugar e_0
   &
   \text{suppose}
   \locallabel{desug:expr}
   \\
   &
   \gamma \desugar \gamma'
   &
   \text{suppose}
   \locallabel{desug:env}
   \\
   &
   \gamma, s_0 \evalSugS v_0
   &
   \text{suppose}
   \locallabel{eval:surf}
   \\
   \intertext{\crossrule}
   %%%%%%%%%%%%%%%%%%%%%%%%%%%%%%%%%%%%%%%%%%%%%%%%%%%%%%%%%%%%%%%%%%%%%%%%
   &
   \caseDerivation{\derivationWidth}{
      \begin{smathpar}
         \inferrule*[
            lab={\ruleName{$\desugar$-var}}
         ]
         {
            \strut
         }
         {
            \Lowlight{s_0 =\;} \exVar{x} \desugar \exVar{x} \Lowlight{\;= e_0}
         }
      \end{smathpar}
   }
   &
   \notag
   \\
   &
   \derivation{\derivationWidth}{
      \begin{smathpar}
         \inferrule*[
            lab={\ruleName{$\evalSugS$-var}}
         ]
         {
            \strut
         }
         {
            \Lowlight{\gamma =\;} {\gamma_1} \cons (\bind{x}{v}), \exVar{x} \evalSugS v
         }
      \end{smathpar}
   }
   &
   \notag
   \\
   &
   \gamma_1\cons(\bind{x}{v}) \desugar \gamma_2\cons(\bind{x}{v'})
   \textit{ with }
   v \desugar v'
   \quad
   (\exists \gamma_2, v')
   &
   (\text{\localref{desug:env}), \ruleName{$\desugar$-env}}
   \notag
   \\
   &
   \qedLocal
   \derivation{\derivationWidth}{
      \begin{smathpar}
         \inferrule*[
            lab={\ruleName{$\evalSugS$-var}}
         ]
         {
            \strut
         }
         {
            \gamma_2 \cdot (\bind{\exVar{x}}{v'}), \exVar{x} \evalSugS v'
         }
      \end{smathpar}
   }
   &
   \notag
   \\
   \intertext{\crossrule}
   %%%%%%%%%%%%%%%%%%%%%%%%%%%%%%%%%%%%%%%%%%%%%%%%%%%%%%%%%%%%%%%%%%%%%%%%
   &
   \caseDerivation{\derivationWidth}{
      \begin{smathpar}
         \inferrule*[
            lab={\ruleName{$\desugar$-constr}}
         ]
         {
            \seq{s} \desugar \seq{e}
         }
         {
            \exConstr{c}{\seq{s}} \desugar \exConstr{c}{\seq{e}}
         }
      \end{smathpar}
   }
   &
   \notag
   \\
   &
   \derivation{\derivationWidth}{
      \begin{smathpar}
         \inferrule*[
            lab={\ruleName{$\evalSugS$-constr}}
         ]
         {
            \gamma, \seq{s} \evalSugS \seq{v}
         }
         {
            \gamma, \exConstr{c}{\seq{s}} \evalSugS \exConstr{c}{\seq{v}}
         }
      \end{smathpar}
   }
   &
   \notag
   \\
   &
   \gamma', e \evalSugS \seq{v}'
   \textit{ with }
   \seq{v} \desugar \seq{v}'
   \quad
   (\exists \seq{v}')
   &
   \text{IH}
   \notag
   \\
   &
   \qedLocal
   \derivation{\derivationWidth}{
      \begin{smathpar}
         \inferrule*[
            lab={\ruleName{$\evalSugS$-constr}}
         ]
         {
            \gamma', \seq{e} \evalSugS \seq{v}'
         }
         {
            \gamma', \exConstr{c}{\seq{e}} \evalSugS \exConstr{c}{\seq{v}'}
         }
      \end{smathpar}
   }
   &
   \notag
   \\
   &
   \qedLocal
   \derivation{\derivationWidth}{
      \begin{smathpar}
         \inferrule*[
            lab={\ruleName{$\desugar$-constr}}
         ]
         {
            \seq{v} \desugar \seq{v}'
         }
         {
            \exConstr{c}{\seq{v}} \desugar \exConstr{c}{\seq{v}'}
         }
      \end{smathpar}
   }
   &
   \notag
   \intertext{\crossrule}
   %%%%%%%%%%%%%%%%%%%%%%%%%%%%%%%%%%%%%%%%%%%%%%%%%%%%%%%%%%%%%%%%%%%%%%%%
   &
   \caseDerivation{\derivationWidth}{
      \begin{smathpar}
         \inferrule*[
            lab={\ruleName{$\desugar$-app}}
         ]
         {
            s \desugar e
            \\
            s' \desugar e'
         }
         {
            \exApp{s}{s'} \desugar \exApp{e}{e'}
         }
      \end{smathpar}
   }
   &
   \notag
   \\
   &
   \derivation{\derivationWidth}{
      \begin{smathpar}
         \inferrule*[
            lab={\ruleName{$\evalSugS$-app}},
            width=3in,
         ]
         {
            \gamma, s \evalSugS \exClosure{\gamma_1}{g}{\mu}
            \\
            \gamma, s' \evalSugS v
            \\
            \gamma_1, g \closeDefs \gamma_2
            \\
            v, \mu \match \gamma_3, s^\dag
            \\
            \gamma_1 \concat \gamma_2 \concat \gamma_3, s^\dag \evalSugR{S^\dag} v^{\dag}
         }
         {
            \gamma, \exApp{s}{s'} \evalSugR{\trApp{S}{S'}{p}{S^{\dag}}} v^{\dag}
         }
      \end{smathpar}
   }
   &
   \notag
   \\
   &
   \gamma', e \evalSugS \exClosure{\gamma'_1}{\rho}{\sigma}
   \textit{ with }
   \gamma_1 \desugar \gamma_1'
   \textit{ and }
   g \desugar \rho
   \textit{ and }
   \mu \desugar \sigma
   \quad
   (\exists \gamma_1',\rho,\sigma)
   &
   \text{IH, $\desugar$-closure}
   \notag
   \\
   &
   \gamma', e' \evalSugS v'
   \textit{ with }
   v \desugar v'
   \quad
   (\exists v')
   &
   \text{IH}
   \notag
   \\
   &
   \gamma'_1, \rho \closeDefs \gamma'_2
   \textit{ with }
   \gamma_2 \desugar \gamma'_2
   \quad
   (\exists \gamma'_2)
   &
   \text{\lemref{closedefs-eq}}
   \notag
   \\
   &
   v', \sigma \match \gamma'_3, e^{\dag}
   \textit{ with }
   \gamma_3 \desugar \gamma'_3
   \textit{ and }
   s^{\dag} \desugar e^{\dag}
   \quad
   (\exists \gamma'_3, e^{\dag})
   &
   \text{\lemref{match-eq}}
   \notag
   \\
   &
   \gamma_1\concat\gamma_2\concat\gamma_3 \desugar \gamma'_1\concat\gamma'_2\concat\gamma'_3
   &
   \text{\ruleName{$\desugar$-env}}
   \notag
   \\
   &
   \gamma'_1 \concat \gamma'_2 \concat \gamma'_3, e^{\dag} \evalSugS u
   \textit{ with }
   v^{\dag} \desugar u
   \quad
   (\exists u)
   &
   \text{IH}
   \notag
   \\
   &
   \qedLocal
   \derivation{\derivationWidth}{
      \begin{smathpar}
         \inferrule*[
            lab={\ruleName{$\evalSugS$-app}},
            width=3.3in,
         ]
         {
            \gamma', (e, e') \evalS (\exClosure{\gamma_1}{\rho}{\sigma}, v')
            \\
            \gamma'_1, \rho \closeDefs \gamma'_2
            \\
            v', \sigma \match \gamma'_3, e^{\dag}
            \\
            \gamma'_1 \concat \gamma'_2 \concat \gamma'_3, e^{\dag} \evalSugS u
         }
         {
            \gamma', \exApp{e}{e'}
            \evalSugS
            u
         }
      \end{smathpar}
   }
   &
   \notag
   \\
   \intertext{\crossrule}
   %%%%%%%%%%%%%%%%%%%%%%%%%%%%%%%%%%%%%%%%%%%%%%%%%%%%%%%%%%%%%%%%%%%%%%%%
   &
   \caseDerivation{\derivationWidth}{
      \begin{smathpar}
         \inferrule*[lab={\ruleName{$\desugar$-let-rec}}]
         {
            \seq{\mu} \desugar \seq{\sigma}
            \\
            s \desugar e
         }
         {
            \exLetRecPiecewise{\seq{\bind{x}{\mu}}}{s}
            \desugar
            \exLetRecPiecewise{\seq{\bind{x}{\sigma}}}{e}
         }
      \end{smathpar}
   }
   &
   \notag
   \\
   &
   \derivation{\derivationWidth}{
      \begin{smathpar}
         \inferrule*[
            lab={\ruleName{$\evalSugS$-let-rec}}
         ]
         {
            \gamma, \seq{\bind{x}{\mu}} \closeDefs \gamma^{\dag}
            \\
            \gamma \concat \gamma^{\dag}, s \evalSugS v
         }
         {
            \gamma, \exLetRecPiecewise{\seq{\bind{x}{\mu}}}{s} \evalSugS v
         }
      \end{smathpar}
   }
   &
   \notag
   \\
   &
   \gamma', \seq{\bind{x}{\sigma}} \closeDefs \gamma^{\ddagger}
   \textit{ with }
   \gamma^{\dag} \desugar \gamma^{\ddagger}
   \quad
   (\exists \gamma^\ddagger)
   &
   \text{\lemref{closedefs-eq}}
   \notag
   \\
   &
   \gamma \concat \gamma^{\dag} \desugar \gamma' \concat \gamma^{\ddagger}
   &
   \text{\ruleName{$\desugar$-env}, (\localref{desug:env})}
   \notag
   \\
   &
   \gamma' \concat \gamma^{\ddagger}, e \evalSugS v'
   \textit{ with }
   v \desugar v'
   \quad
   (\exists v')
   &
   \text{IH}
   \notag
   \\
   &
   \qedLocal
   \derivation{\derivationWidth}{
      \begin{smathpar}
         \inferrule*[lab={\ruleName{$\evalSugS$-let-rec}}]
         {
            \gamma', \seq{\bind{\exVar{x}}{\sigma}} \closeDefs {\gamma^{\ddagger}}
            \\
            \gamma' \concat {\gamma^{\ddagger}}, e \evalSugS v'
         }
         {
            \gamma', \exLetRecPiecewise{\seq{\bind{\exVar{x}}{\sigma}}}{e} \evalSugS v'
         }
      \end{smathpar}
   }
   &
   \notag
   \\
   \intertext{\crossrule}
   %%%%%%%%%%%%%%%%%%%%%%%%%%%%%%%%%%%%%%%%%%%%%%%%%%%%%%%%%%%
   &
   \caseDerivation{\derivationWidth}{
      \begin{smathpar}
         \inferrule*[lab={\ruleName{$\desugar$-list-comp-done}}]
         {
            s \desugar e
         }
         {
            \exListComp{s}{\seqEmpty}
            \desugar
            \exConstr{\cCons}{e, \exNil}
         }
      \end{smathpar}
   }
   &
   \notag
   \\
   &
   \derivation{\derivationWidth}{
      \begin{smathpar}
         \inferrule*[lab={\ruleName{$\evalSugS$-list-comp-done}}]
         {
            \gamma, s \evalSugR{S} u
         }
         {
            \gamma, \exListComp{s}{\seqEmpty} \evalSugR{\seqEmpty, S} \exConstr{\cCons}{u, \exNil}
         }
      \end{smathpar}
   }
   &
   \notag
   \\
   &
   \gamma', e \evalS v
   \textit{ with }
   u \desugar v
   \quad
   (\exists v)
   &
   \text{IH}
   \notag
   \\
   &
   \qedLocal
   \derivation{\derivationWidth}{
      \begin{smathpar}
         \inferrule*[
            lab={\ruleName{$\evalS$-constr}}
         ]
         {
            \gamma', e \evalS v
         }
         {
            \gamma', \exConstr{\cCons}{e, \exNil} \evalS \exConstr{\cCons}{v, \exNil}
         }
      \end{smathpar}
   }
   &
   \notag
   \\
   \intertext{\crossrule}
   %%%%%%%%%%%%%%%%%%%%%%%%%%%%%%%%%%%%%%%%%%%%%%%%%%%%%%%%%%%
   &
   \caseDerivation{\derivationWidth}{
      \begin{smathpar}
         \inferrule*[lab={\ruleName{$\desugar$-list-comp-guard}}]
         {
            s \desugar e
            \\
            \exListComp{s'}{\seq{q}} \desugar e'
            \\
            \sigma = \elimConstr{\elimBind{\cTrue}{e'}, \elimBind{\cFalse}{\exNil}}
         }
         {
            \exListComp{s'}{\qualGuard{s} \cons \seq{q}}
            \desugar
            \exApp{\exFun{\sigma}}{e}
         }
      \end{smathpar}
   }
   &
   \notag
   \\
   &
   \derivation{\derivationWidth}{
      \begin{smathpar}
         \inferrule*[
            lab={\ruleName{$\evalSugS$-list-comp-guard-false}}
         ]
         {
            \gamma, s \evalSugR{S} \cFalse
         }
         {
            \gamma, \exListComp{s'}{\qualGuard{s} \cons \seq{q}} \evalSugR{\trQualIfFalse{S}{q}} \exNil
         }
      \end{smathpar}
   }
   &
   \notag
   \\
   &
   \gamma', e \evalS \cFalse
   &
   \text{IH}
   \notag
   \\
   &
   \cFalse, \sigma \match \envEmpty, \exNil
   &
   \text{\ruleName{$\match$-constr}}
   \notag
   \\
   &
   \gamma', \envEmpty \closeDefs \envEmpty
   &
   \text{\defref{core:close-defs}}
   \notag
   \\
   &
   \gamma', \exNil \evalS \exNil
   &
   \text{\ruleName{$\evalS$-constr}}
   \notag
   \\
   &
   \qedLocal
   \derivation{\derivationWidth}{
      \begin{smathpar}
         \inferrule*[
            lab={\ruleName{$\evalSugS$-app}},
            width=3.3in,
         ]
         {
            \gamma', \exFun{\sigma} \evalS \exClosure{\gamma'}{\envEmpty}{\sigma}
            \\
            \gamma', e \evalS \cFalse
            \\
            \gamma', \envEmpty \closeDefs \envEmpty
            \\
            \cFalse, \sigma \match \envEmpty, \exNil
            \\
            \gamma' \concat \envEmpty \concat \envEmpty, \exNil \evalSugS \exNil
         }
         {
            \gamma', \exApp{\exFun{\sigma}}{e}
            \evalSugS
            \exNil
         }
      \end{smathpar}
   }
   &
   \notag
   \\
   \intertext{\crossrule}
   %%%%%%%%%%%%%%%%%%%%%%%%%%%%%%%%%%%%%%%%%%%%%%%%%%%%%%%%%%%
   &
   \caseDerivation{\derivationWidth}{
      \begin{smathpar}
         \inferrule*[lab={\ruleName{$\desugar$-list-comp-guard}}]
         {
            s \desugar e
            \\
            \exListComp{s'}{\seq{q}} \desugar e'
            \\
            \sigma = \elimConstr{\elimBind{\cTrue}{e'}, \elimBind{\cFalse}{\exNil}}
         }
         {
            \exListComp{s'}{\qualGuard{s} \cons \seq{q}}
            \desugar
            \exApp{\exFun{\sigma}}{e}
         }
      \end{smathpar}
   }
   &
   \notag
   \\
   &
   \derivation{\derivationWidth}{
      \begin{smathpar}
         \inferrule*[
            lab={\ruleName{$\evalSugS$-list-comp-guard-true}},
         ]
         {
            \gamma, \exListComp{s'}{\seq{q}} \evalSugR{\seq{Q},S} v
            \\
            \gamma, s \evalSugR{S} \cTrue
         }
         {
            \gamma, \exListComp{s'}{\qualGuard{s} \cons \seq{q}} \evalSugR{\trQualIfTrue{S} \cons \seq{Q}, S} v
         }
      \end{smathpar}
   }
   &
   \notag
   \\
   &
   \gamma', e \evalS \cTrue
   &
   \text{IH}
   \notag
   \\
   &
   \cTrue, \sigma \match \envEmpty, e'
   &
   \text{\ruleName{$\match$-constr}}
   \notag
   \\
   &
   \gamma', e' \evalS v'
   \textit{ with }
   v \desugar v'
   \quad
   (\exists v')
   &
   \text{IH}
   \notag
   \\
   &
   \gamma, \envEmpty \closeDefs \envEmpty
   &
   \text{\defref{core:close-defs}}
   \notag
   \\
   &
   \qedLocal
   \derivation{\derivationWidth}{
      \begin{smathpar}
         \inferrule*[
            lab={\ruleName{$\evalSugS$-app}},
            width=3.3in,
         ]
         {
            \gamma', \exFun{\sigma} \evalS \exClosure{\gamma'}{\envEmpty}{\sigma}
            \\
            \gamma', e \evalS \cTrue
            \\
            \gamma', \envEmpty \closeDefs \envEmpty
            \\
            \cTrue, \sigma \match \envEmpty, e'
            \\
            \gamma' \concat \envEmpty \concat \envEmpty, e' \evalSugS v'
         }
         {
            \gamma', \exApp{\exFun{\sigma}}{e}
            \evalSugS
            v'
         }
      \end{smathpar}
   }
   &
   \notag
   \\
   \intertext{\crossrule}
   %%%%%%%%%%%%%%%%%%%%%%%%%%%%%%%%%%%%%%%%%%%%%%%%%%%%%%%%%%%
   &
   \caseDerivation{\derivationWidth}{
      \begin{smathpar}
         \inferrule*[lab={\ruleName{$\desugar$-list-comp-decl}}]
         {
            s \desugar e
            \\
            (\clause{p}{\exListComp{s'}{\seq{q}}}) \desugar \sigma
         }
         {
            \exListComp{s'}{\qualDeclaration{p}{s} \cons \seq{q}}
            \desugar
            \exApp{\exFun{\sigma}}{e}
         }
      \end{smathpar}
   }
   &
   \notag
   \\
   &
   \derivation{\derivationWidth}{
      \begin{smathpar}
         \inferrule*[
            lab={\ruleName{$\evalSugS$-list-comp-decl}}
         ]
         {
            \gamma, s \evalSugR{S'} u'
            \\
            u', (\clause{p}{\exListComp{s'}{\seq{q}}}) \match \gamma^\dag, s^\dag
            \\
            \gamma \concat \gamma^\dag, s^\dag \evalSugR{\seq{Q},S} u
         }
         {
            \gamma, \exListComp{s'}{\qualDeclaration{p}{s} \cons \seq{q}} \evalSugR{\trQualDecl{p}{S'} \cons \seq{Q}, S} u
         }
      \end{smathpar}
   }
   &
   \notag
   \\
   &
   \gamma', e \evalS v'
   \textit{ with }
   u' \desugar v'
   \quad
   (\exists v')
   &
   \text{IH}
   \notag
   \\
   &
   v', \sigma \match \gamma^\ddagger, e^\dag
   \textit{ with }
   \gamma^\dag \desugar \gamma^\ddagger
   \textit{ and }
   s^\dag \desugar e^\dag
   \quad
   (\exists \gamma^\ddagger, e^\dag)
   &
   \text{\lemref{match-eq}}
   \notag
   \\
   &
   \gamma', \exFun{\sigma} \evalS \exClosure{\gamma'}{\envEmpty}{\sigma}
   \textit{ with }
   \gamma \desugar \gamma'
   &
   \text{\ruleName{$\evalS$-lambda}}
   \notag
   \\
   &
   \gamma', \envEmpty \closeDefs \envEmpty
   &
   \text{\defref{surface:close-defs}}
   \notag
   \\
   &
   \gamma' \concat \envEmpty \concat \gamma^\ddagger, e^\dag \evalS u^\dag
   \textit{ with }
   u \desugar u^\dag
   \quad
   (\exists u^\dag)
   &
   \text{IH}
   \notag
   \\
   &
   \qedLocal
   \derivation{\derivationWidth}{
      \begin{smathpar}
         \inferrule*[
            lab={\ruleName{$\evalSugS$-app}},
            width=3.3in,
         ]
         {
            \gamma', (\exFun{\sigma}, e) \evalS (\exClosure{\gamma'}{\envEmpty}{\sigma}, v')
            \\
            \gamma', \envEmpty \closeDefs \envEmpty
            \\
            v', \sigma \match \gamma^\ddagger, e^\dag
            \\
            \gamma' \concat \envEmpty \concat \gamma^\ddagger, e^\dag \evalSugS u^\dag
         }
         {
            \gamma', \exApp{\exFun{\sigma}}{e}
            \evalSugS
            u^\dag
         }
      \end{smathpar}
   }
   &
   \notag
   \\
   \intertext{\crossrule}
   %%%%%%%%%%%%%%%%%%%%%%%%%%%%%%%%%%%%%%%%%%%%%%%%%%%%%%%%%%%
   &
   \caseDerivation{\derivationWidth}{
      \begin{smathpar}
         \inferrule*[lab={\ruleName{$\desugar$-list-comp-gen}}]
         {
            s \desugar e
            \\
            (\clause{p}{\exListComp{s'}{\seq{q}}}), \exNil \orElse \mu
            \\
            \mu \desugar \sigma
         }
         {
            \exListComp{s'}{\qualGenerator{p}{s} \cons \seq{q}}
            \desugar
            \exApp{\exApp{\varConcatMap}{\exFun{\sigma}}}{e}
         }
      \end{smathpar}
   }
   &
   \notag
   \\
   &
   \derivation{\derivationWidth}{
      \begin{smathpar}
         \inferrule*[
            lab={\ruleName{$\evalSugS$-list-comp-gen}},
            flushleft
         ]
         {
            (\clause{p}{\exListComp{s'}{\seq{q}}}), \exNil \orElse \mu
            \\
            \gamma, \exApp{\exApp{\varConcatMap}{\exFun{\mu}}}{s} \evalSugS u
         }
         {
            \gamma, \exListComp{s'}{\qualGenerator{p}{s} \cons \seq{q}} \evalSugR{\trQualGen{p}{S'}\cons\seq{Q}, S} u
         }
      \end{smathpar}
   }
   &
   \notag
   \\
   &
   \derivation{\derivationWidth}{
      \begin{smathpar}
         \inferrule*[left=\ruleName{$\desugar$-app}]
         {
            \inferrule*[
               left={\ruleName{$\desugar$-app}}
            ]
            {
               \inferrule*[
%                  left={\ruleName{$\desugar$-var}}
               ]
               {
                  \strut
               }
               {
                  \varConcatMap \desugar \varConcatMap
               }
               \\
               \inferrule*[
                  left={\ruleName{$\desugar$-lambda}}
               ]
               {
                  \mu \desugar \sigma
               }
               {
                  \exFun{\mu} \desugar \exFun{\sigma}
               }
            }
            {
               \exApp{\varConcatMap}{\exFun{\mu}} \desugar \exApp{\varConcatMap}{\exFun{\sigma}}
            }
            \\
            s \desugar e
         }
         {
            \exApp{\exApp{\varConcatMap}{\exFun{\mu}}}{s} \desugar \exApp{\exApp{\varConcatMap}{\exFun{\sigma}}}{e}
         }
      \end{smathpar}
   }
   &
   \notag
   \\
   &
   \qedLocal
   \gamma', \exApp{\exApp{\varConcatMap}{\exFun{\sigma}}}{e} \evalS v
   \textit{ with }
   u \desugar v
   \quad
   (\exists v)
   &
   \text{IH}
   \notag
\end{flalign}
\end{proof}
