# Supplementary material for: Cognacy Queries over Dependence Graphs for Transparent Visualisations
Source: arXiv:2403.04403 source file (2024-10-15)
Supplement: Supplementary file 30 [file close-defs.tex]

\begin{figure}
   {\small \flushleft \shadebox{$\gamma, \rho, G \closeDefs \gamma', G'$} 
      \begin{smathpar}
         \inferrule*[]
         {
            v_{i} = \exClosure{\gamma}{\rho}{\rho(x_i)}_{\alpha_{i} \mapsto G'}
         }
         {
            \gamma,\rho, G \closeDefs \set{\seq{\bind{x}{v}}}, \set{\alpha_{i} \mapsto G' \mid 1 \leq i \leq |\seq{e}|}
         }
      \end{smathpar}
   }
\end{figure}
